# Supplementary material for: ET-Plan-Bench: Embodied Task-level Planning Benchmark Towards Spatial-Temporal Cognition with Foundation Models
Source: arXiv:2410.14682 source file (2025-02-13)
Supplement: Supplementary file 1 [file selected_success_failure_cases_appendix.pdf]

# Pages index

- Navigation Tasks with or without Spatial Constraints
  - Navi + Layout Map
  - Navi
  - Navi + Occlusion\_Size
  - Navi + Occlusion\_Distance
  - Navi + Relation
  - Navi + Relation + Occlusion\_Size
  - Navi + Relation + Occlusion\_Distance
- Navigation & Manipulation Tasks with or without Spatial Constraints
  - Navi & Mani + Layout Map
  - Navi & Mani
  - Navi & Mani + Occlusion\_Size
  - Navi & Mani + Occlusion\_Distance
  - Navi & Mani + Relation
  - Navi & Mani + Relation + Occlusion\_Size
  - Navi & Mani + Relation + Occlusion\_Distance
- Navigation & Manipulation Tasks with Temporal Constraints
  - Navi & Mani + Multi Objects
  - Navi & Mani + Multi Objects + Optimal Path with 2 Arms
  - Navi & Mani + Multi Objects + Temp Dependency

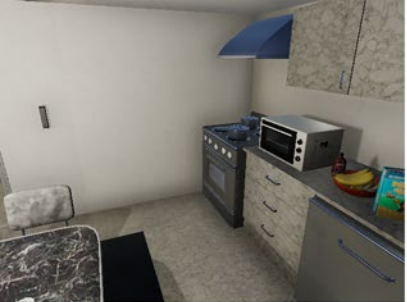

Can you get the box on the wall shelf?

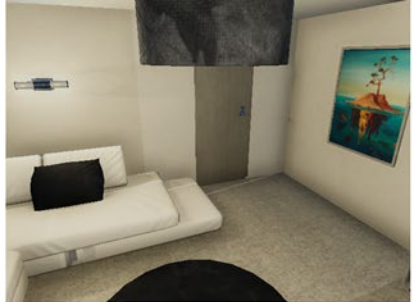

1: Walk to the livingroom

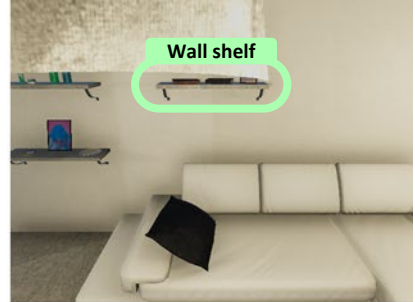

2: Walk to the wall shelf (1)

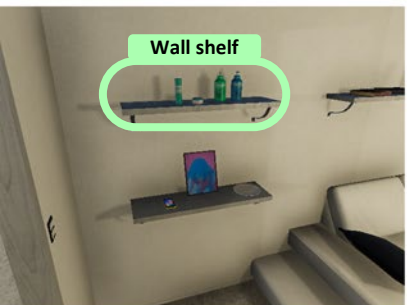

3: Walk to the wall shelf (2)

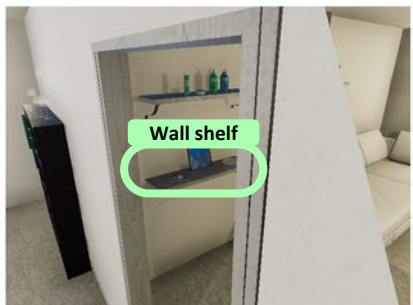

4: Walk to the wall shelf (3)

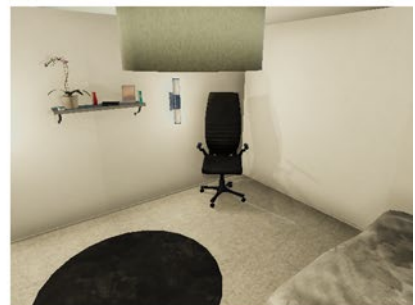

5: Walk to the bedroom

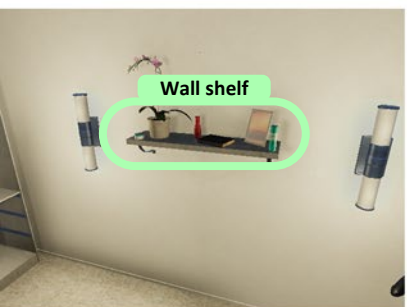

6: Walk to the wall shelf (4)

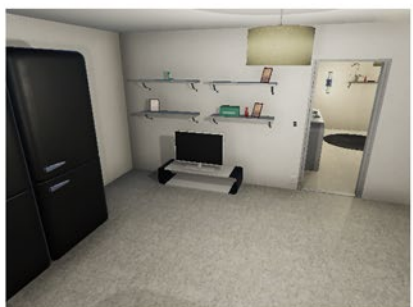

7: Walk to the kitchen

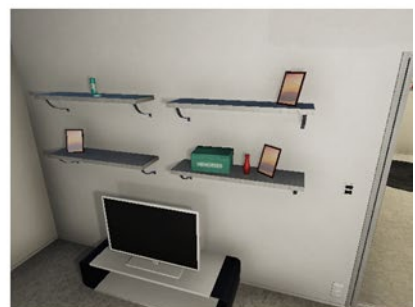

8: Walk to the box

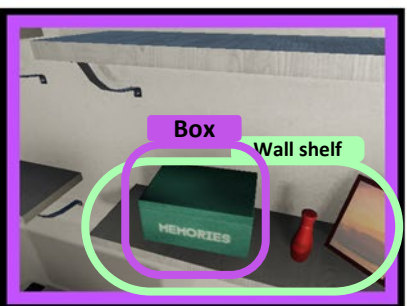

Detected object

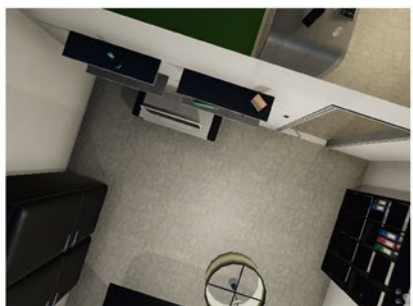

Final state

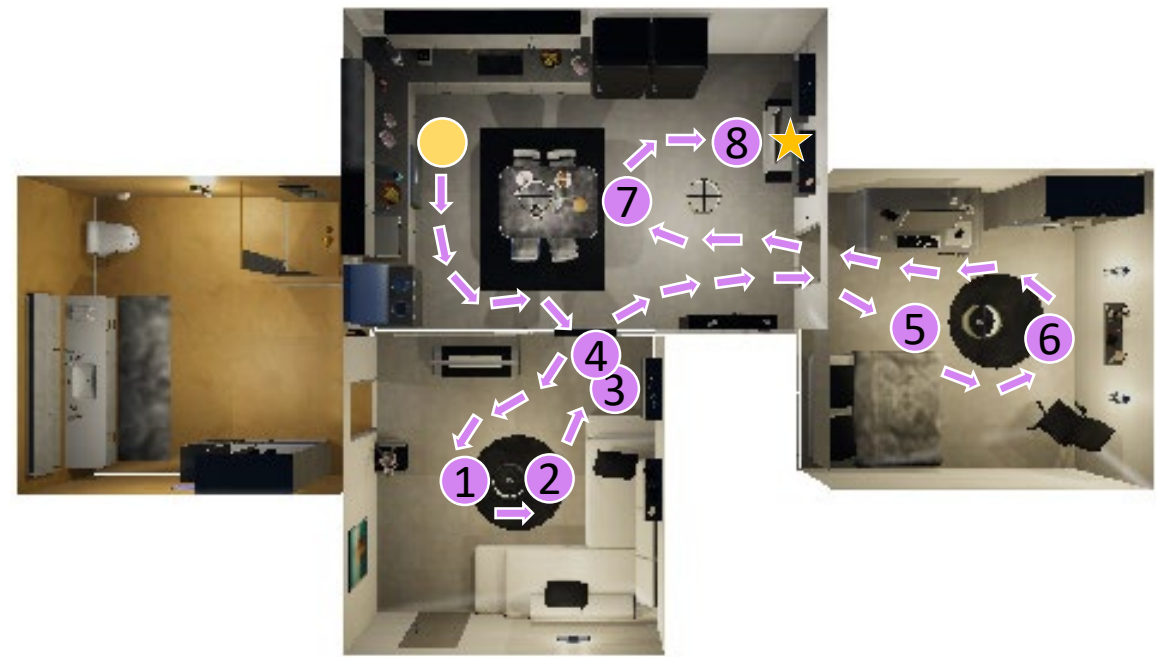

Task: Can you get the **box** on the **wall shelf**?

- 1: Walk to the livingroom
- 2: Walk to the **wall shelf** (1)
- 3: Walk to the **wall shelf** (2)
- 4: Walk to the **wall shelf** (3)
- 5: Walk to the bedroom
- 6: Walk to the **wall shelf** (4)
- 7: Walk to the kitchen
- 8: Walk to the **box**

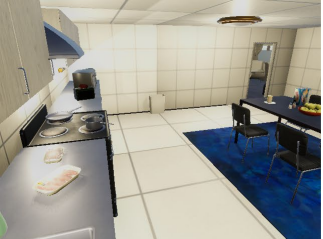

Find the mug and put it inside the fridge.

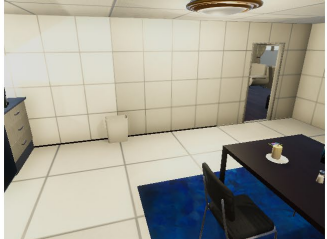

1: Walk to the kitchen

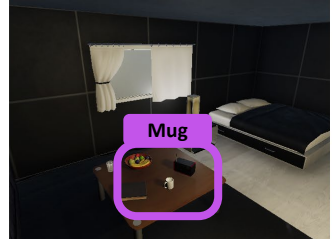

2: Walk to the mug

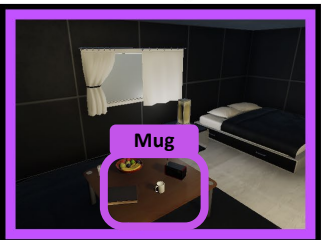

3: Grab the mug

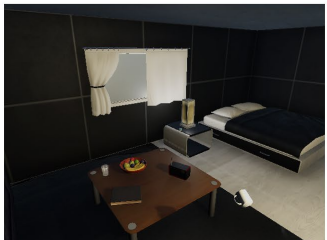

3: Grab the mug

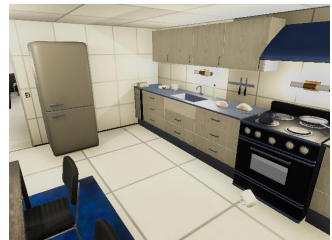

4: Walk to the kitchen

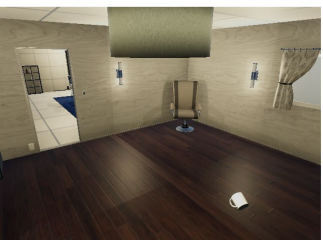

5: Walk to the livingroom

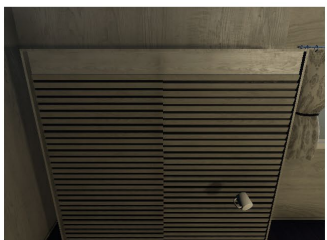

6: Walk to the closet

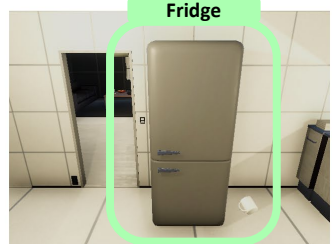

7: Walk to the fridge

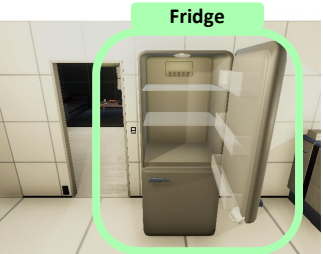

8: Open the fridge

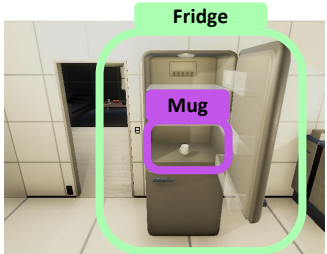

9: Put the mug inside the fridge

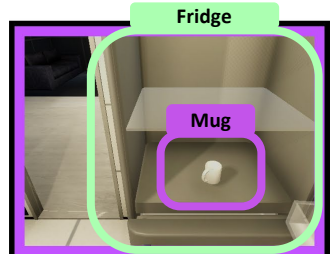

9: Put the mug inside the fridge

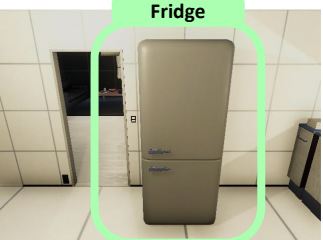

10: Close the fridge

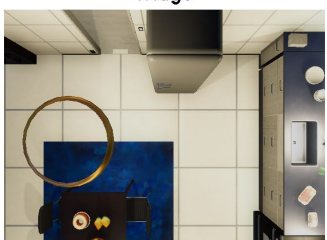

Final state

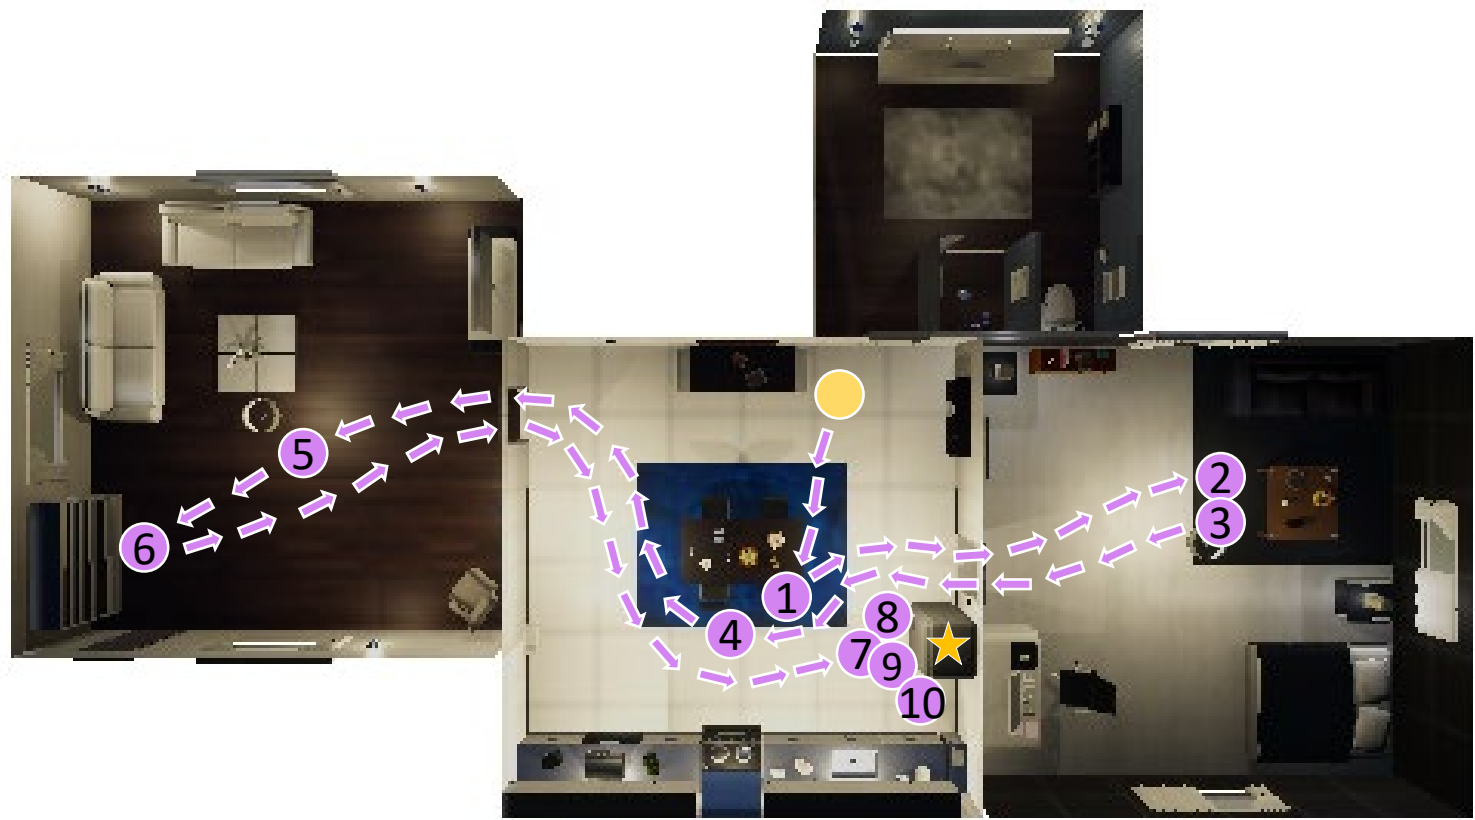

Task: Find the **mug** and put it inside the **fridge**.

1: Walk to the kitchen

2: Walk to the **mug**

3: Grab the **mug**

4: Walk to the kitchen

5: Walk to the livingroom

6: Walk to the closet

7: Walk to the **fridge**

8: Open the **fridge**

9: Put the mug inside the **fridge**

10: Close the **fridge**

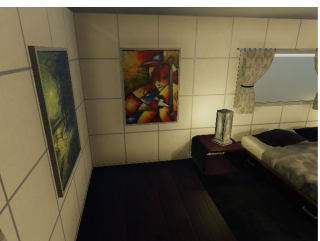

Please place the cutlets on the kitchen table.

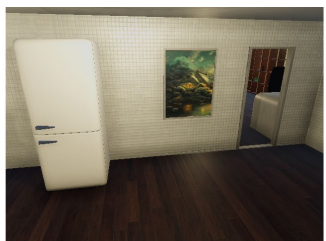

1: Walk to the kitchen

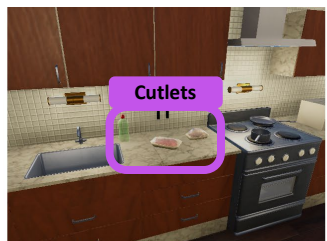

2: Walk to the cutlets

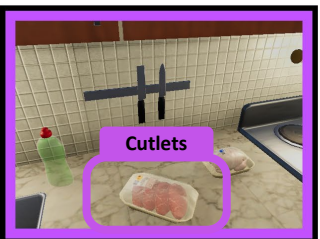

3: Grab the cutlets

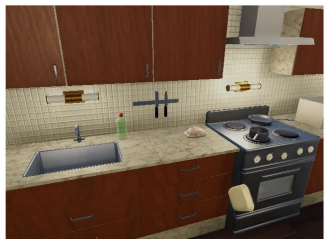

3: Grab the cutlets

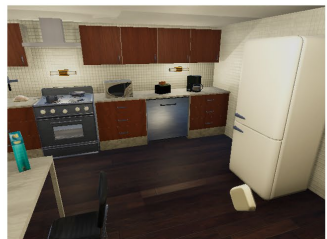

4: Walk to the kitchen

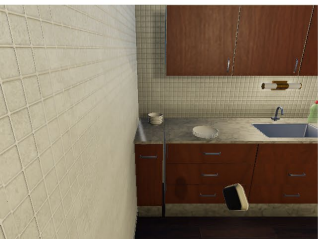

5: Walk to the kitchen counter (1)

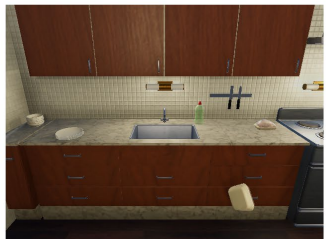

6: Walk to the kitchen counter (2)

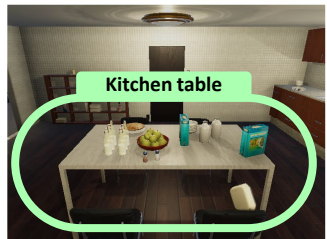

7: Walk to the kitchentable

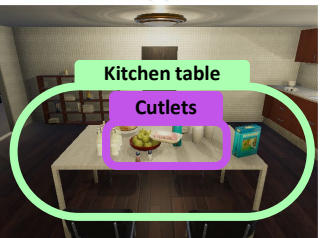

8: Put the cutlets in the kitchentable

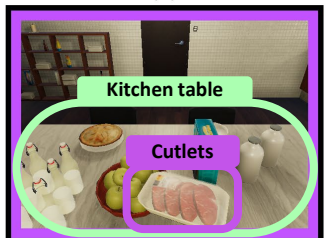

8: Put the cutlets in the kitchentable

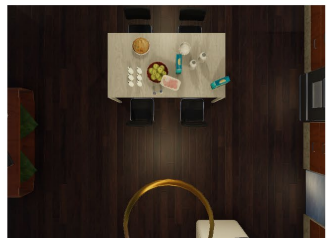

Final state

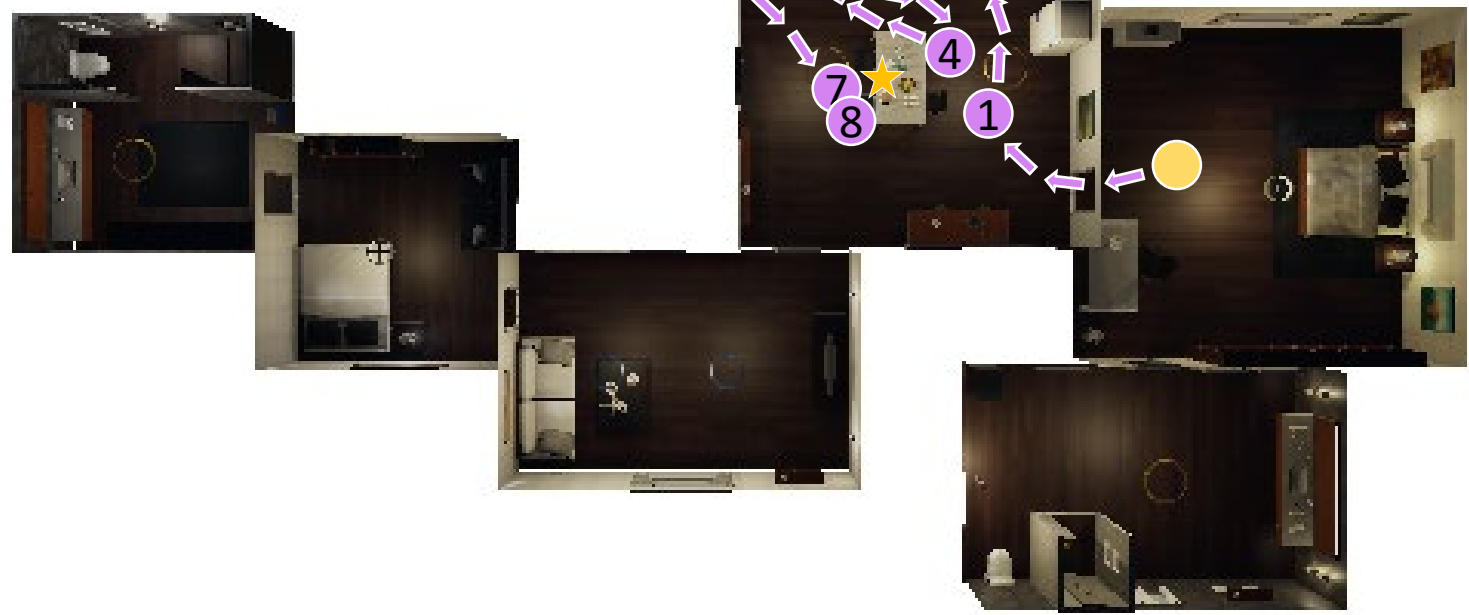

Task: Please place the **cutlets** on the **kitchen table**.

- 1: Walk to the kitchen
- 2: Walk to the **cutlets**
- 3: Grab the **cutlets**
- 4: Walk to the kitchen

- 5: Walk to the kitchen counter (1)
- 6: Walk to the kitchen counter (2)
- 7: Walk to the **kitchen table**
- 8: Put the cutlets in the **kitchen table**

Navi or Navi & Manipulation

Navi or Navi & Manipulation + relation (pick two relations, something like “face to”, ‘next to’)

Navi or Navi & Manipulation + occlusion size

Navi or Navi & Manipulation + distance

Navi & Manipulation + multiple objects

Navi & Manipulation + optimal path

Navi & Manipulation + temp dependency

NAVI SUCCESS

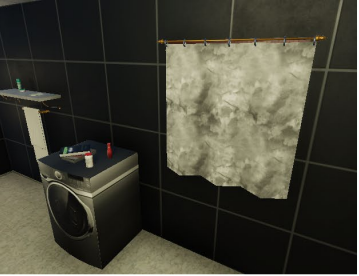

Can you lead me to the desk?

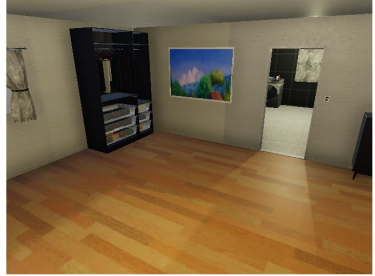

1: Walk to the bedroom

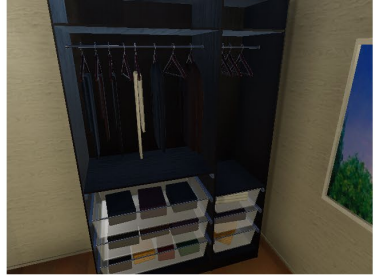

2: Walk to the closet

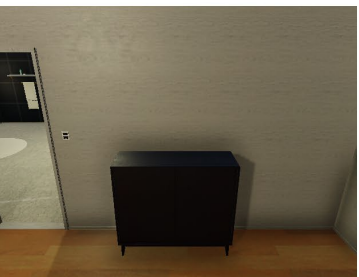

3: Walk to the cabinet (1)

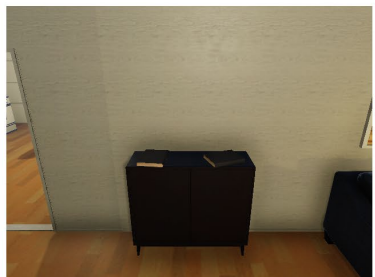

4: Walk to the cabinet (2)

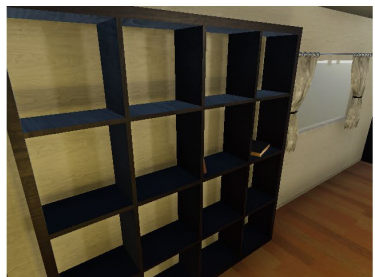

5: Walk to the bookshelf

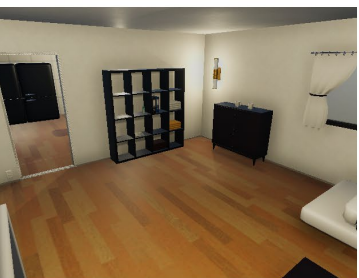

6: Walk to the livingroom

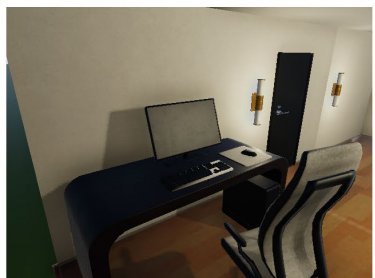

7: Walk to the desk

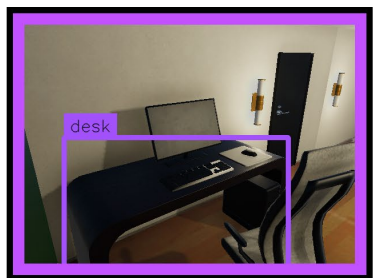

Detected object

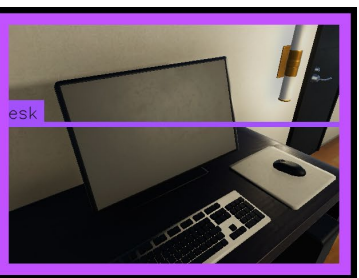

Detected object

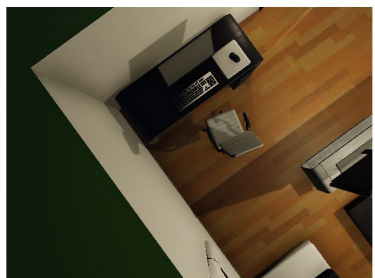

Final state

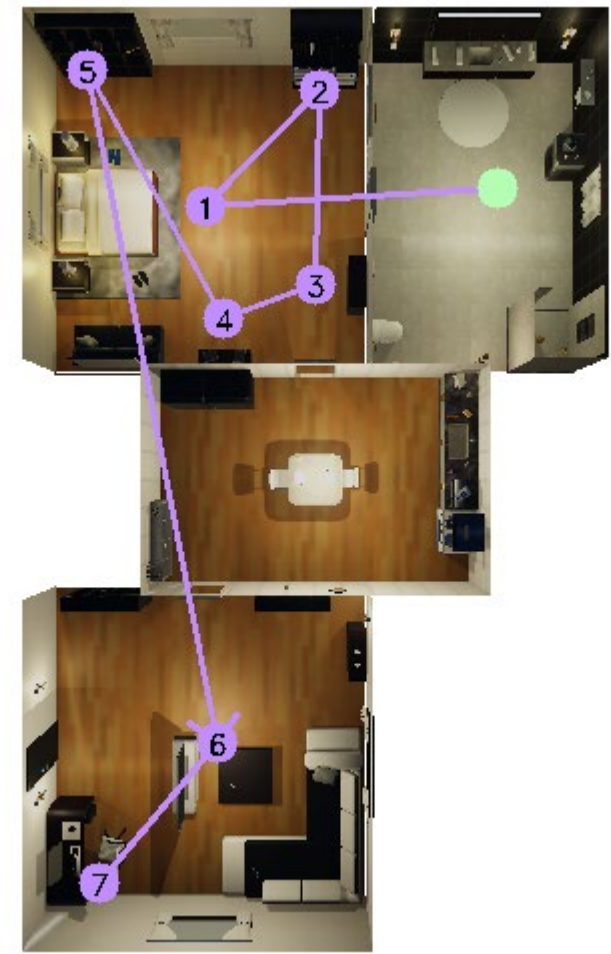

Can you lead me to the desk?

1: Walk to the bedroom

2: Walk to the closet

3: Walk to the cabinet (1)

4: Walk to the cabinet (2)

5: Walk to the bookshelf

6: Walk to the livingroom

7: Walk to the desk

NAVI FAILURE

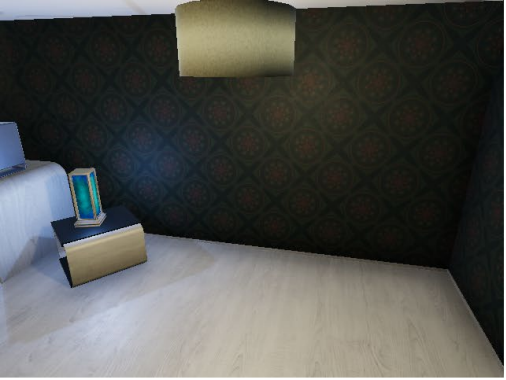

Can you show me where the bench is?

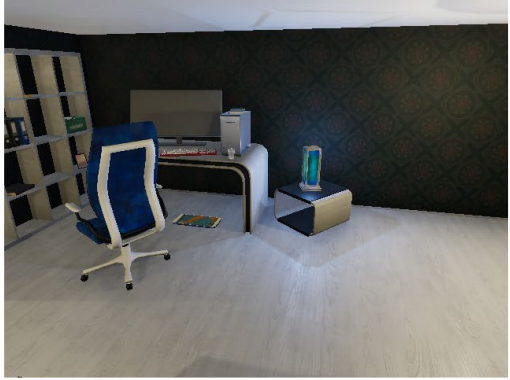

1: Walk to the livingroom

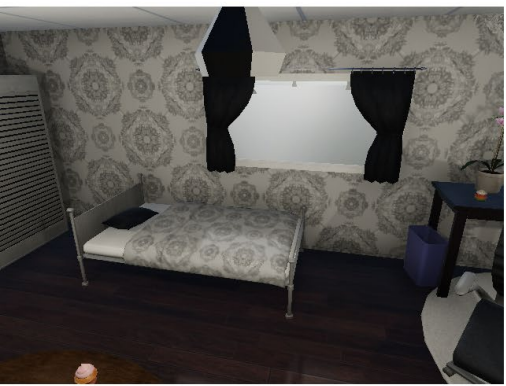

2: Walk to the bedroom

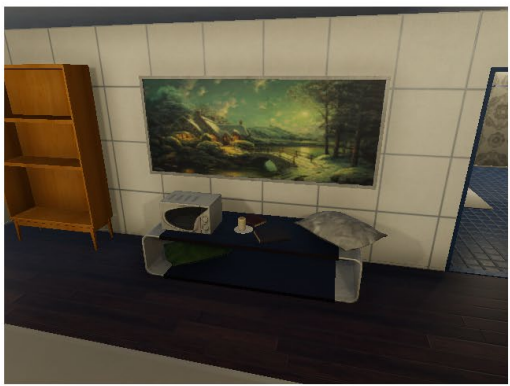

3: Walk to the kitchen

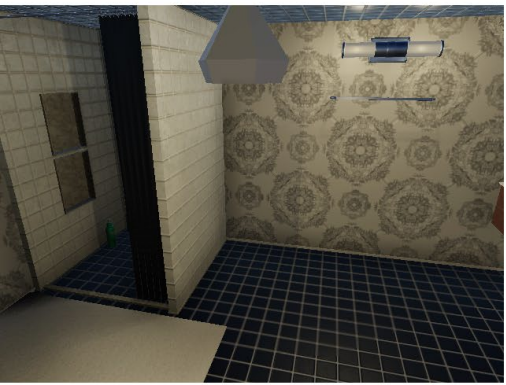

4: Walk to the bathroom

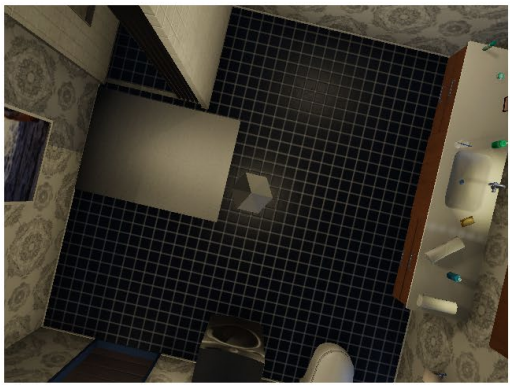

Final state

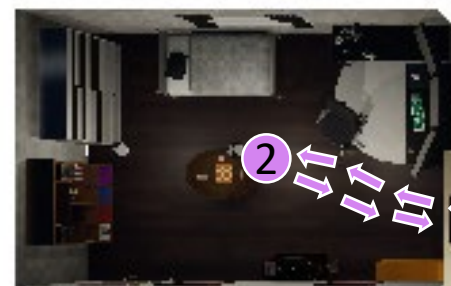

Task: Can you show me where the **bench** is?

- 1: Walk to the livingroom
- 2: Walk to the bedroom
- 3: Walk to the kitchen
- 4: Walk to the bathroom

The LLM decided not to explore any of the rooms other than the initial observation.

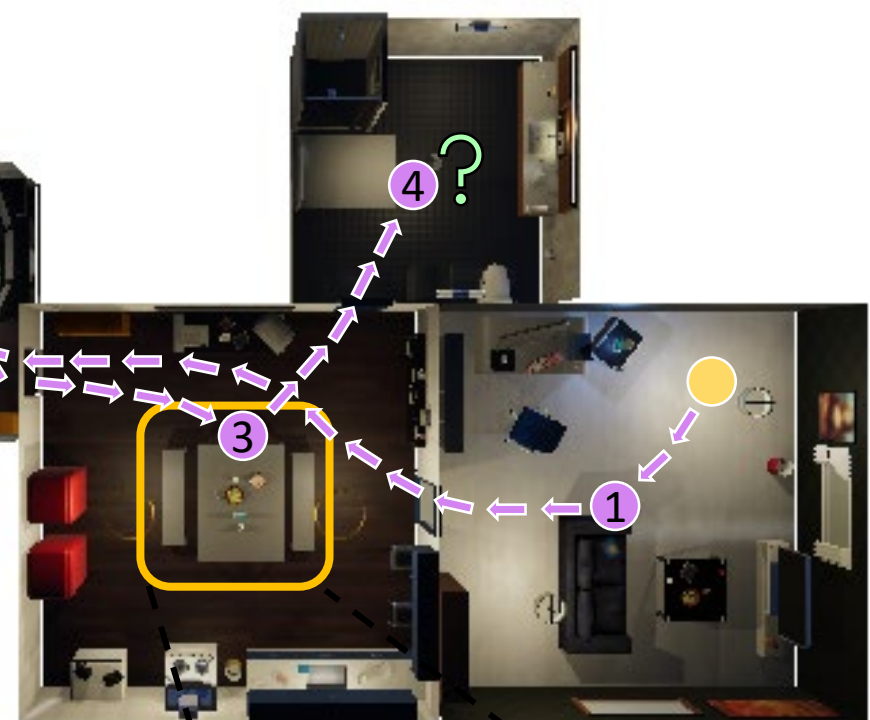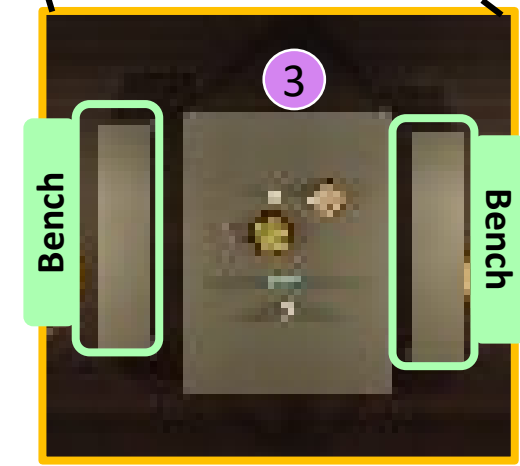

Both benches are obscured by the table.

NAVI RELATION SUCCESS

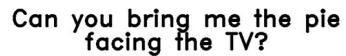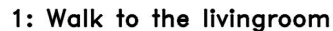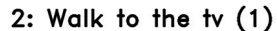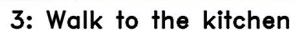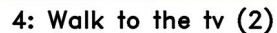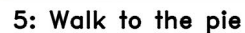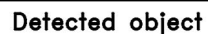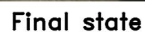

**Task: Can you bring the pie facing the TV?**

- 1: Walk to the livingroom
- 2: Walk to the **tv** (1)
- 3: Walk to the **tv** (2)
- 4: Walk to the kitchen
- 5: Walk to the **pie**

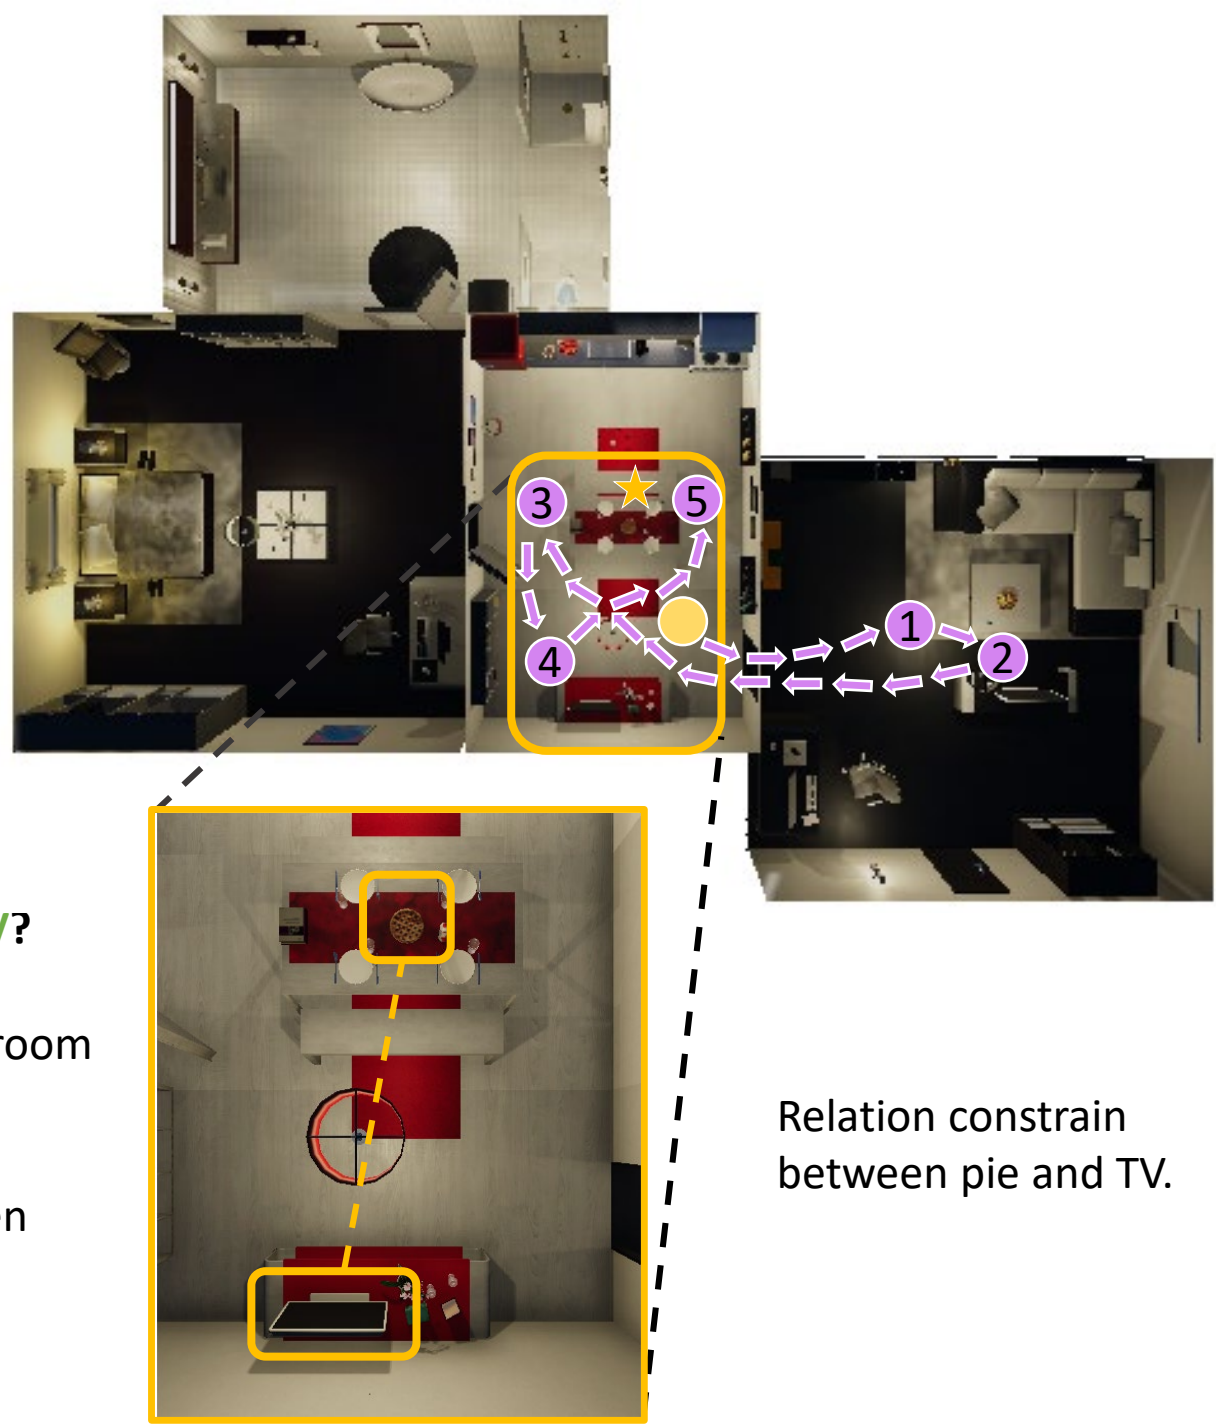

Relation constrain  
between pie and TV.

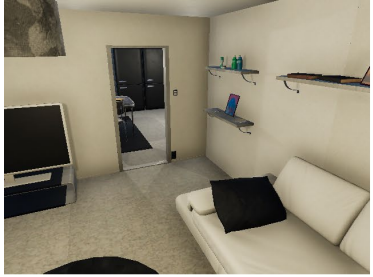

Can you locate the bookshelf facing the TV?

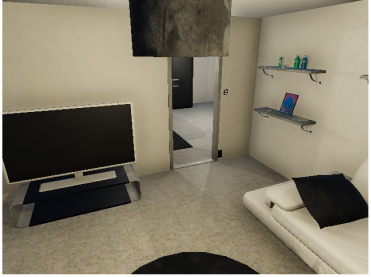

1: Walk to the livingroom

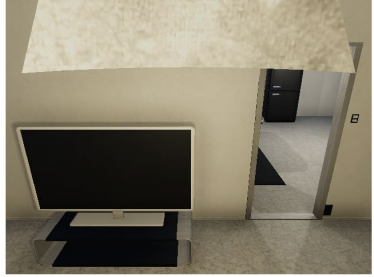

2: Walk to the tv

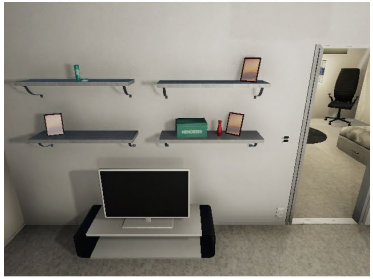

3: Walk to the tv

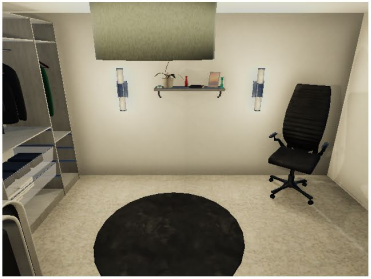

4: Walk to the bedroom

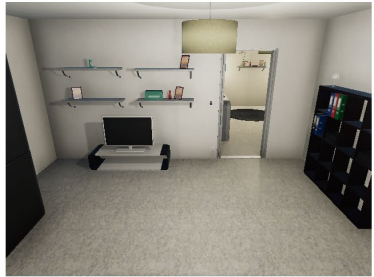

5: Walk to the kitchen

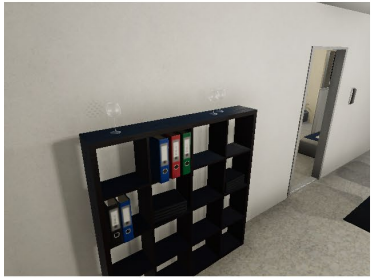

6: Walk to the bookshelf

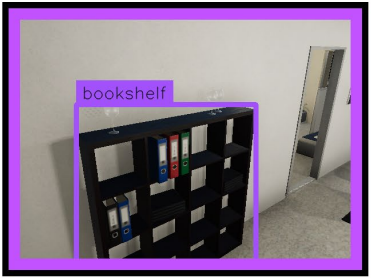

Detected object

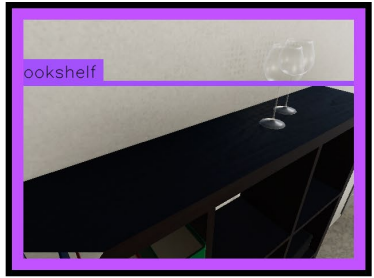

Detected object

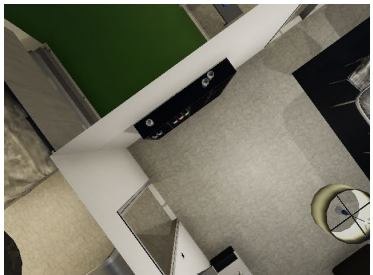

Final state

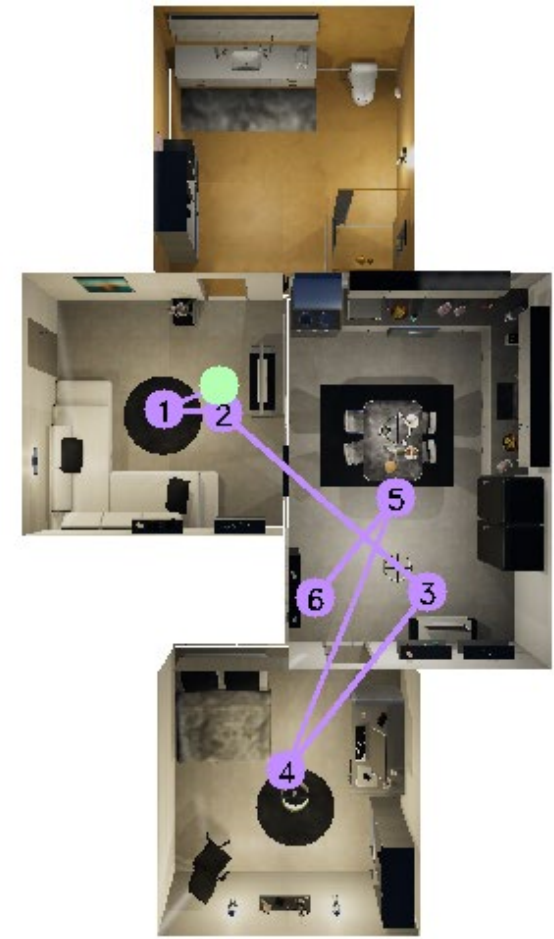

Can you locate the bookshelf facing the TV?

1: Walk to the livingroom

2: Walk to the tv

3: Walk to the tv

4: Walk to the bedroom

5: Walk to the kitchen

6: Walk to the bookshelf

NAVI RELATION FAILURE

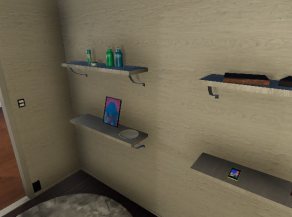

Can you bring me the deodorant close to the toothpaste?

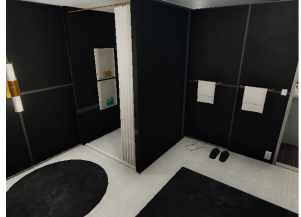

1: Walk to the bathroom

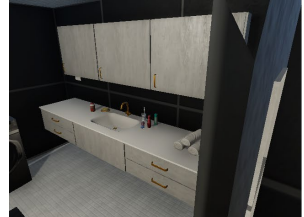

2: Walk to the deodorant

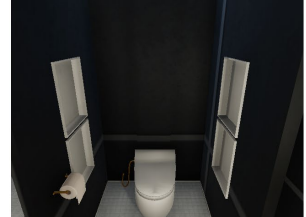

3: Walk to the toilet

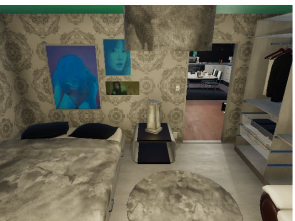

4: Walk to the bedroom

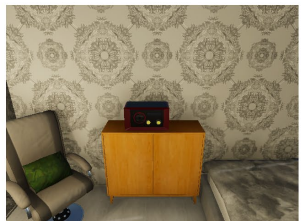

5: Walk to the cabinet (1)

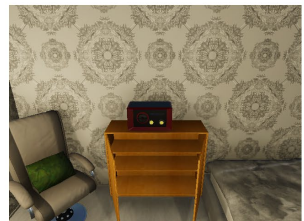

6: Open the cabinet

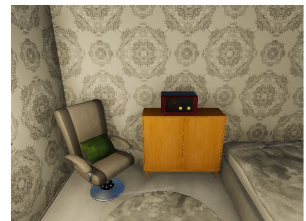

7: Close the cabinet

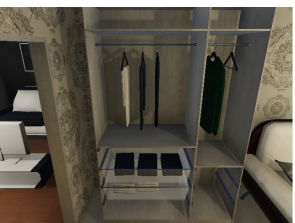

8: Walk to the closet drawer (1)

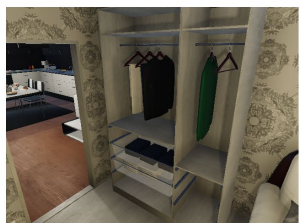

9: Walk to the closet drawer (2)

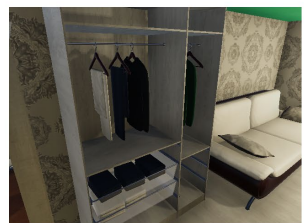

10: Walk to the closet

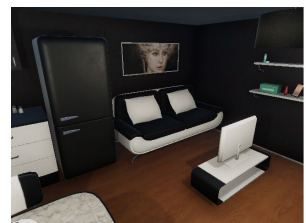

11: Walk to the kitchen

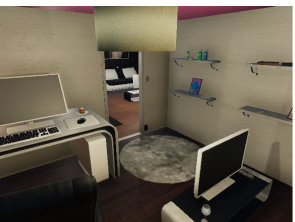

12: Walk to the livingroom

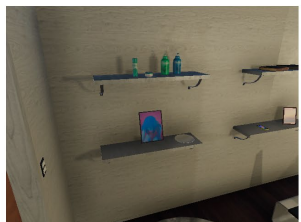

13: Walk to the wall shelf (1)

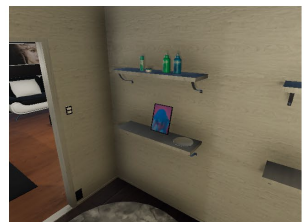

14: Walk to the wall shelf (2)

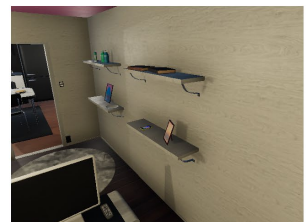

15: Walk to the wall shelf (3)

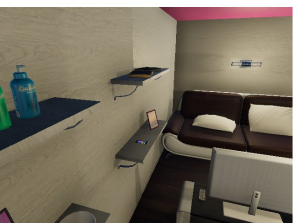

16: Walk to the wall shelf (4)

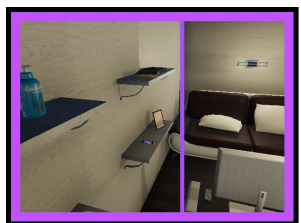

Detected object

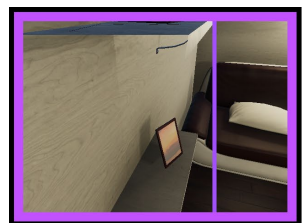

Detected object

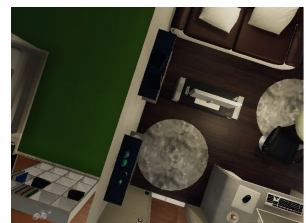

Final state

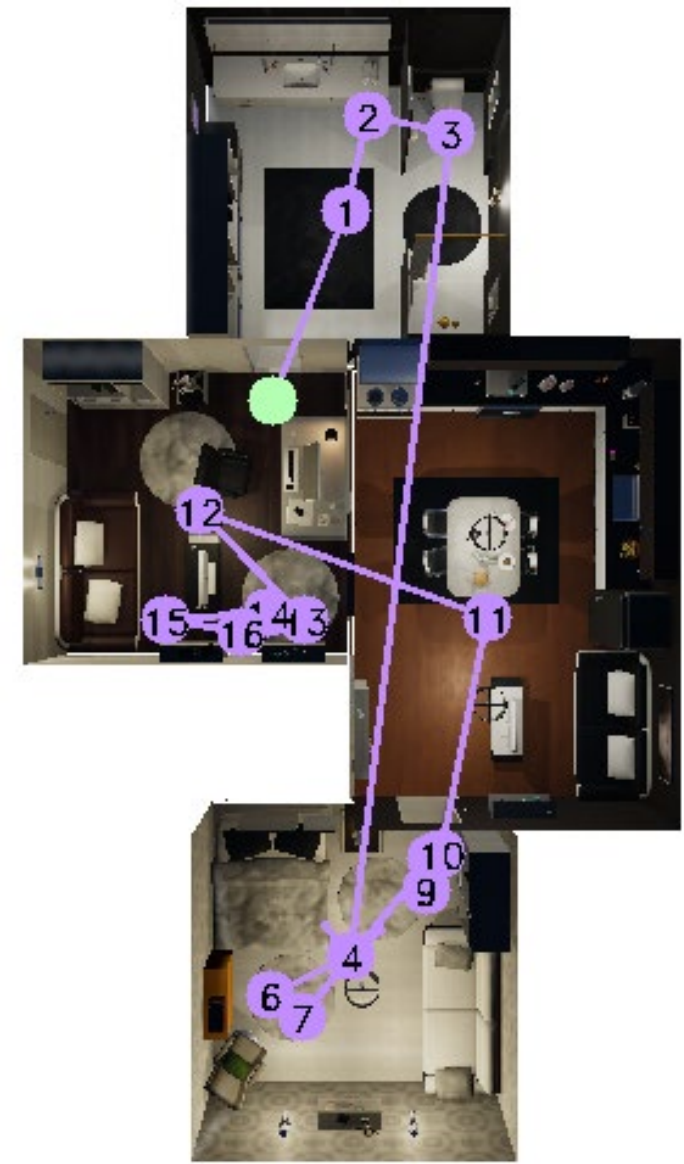

NAVI OCCLUSION SIZE SUCCESS

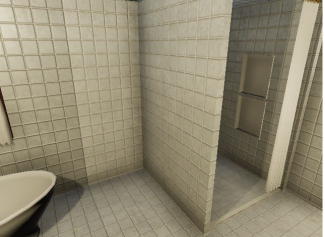

Can you locate the condiment shaker inside the kitchen?

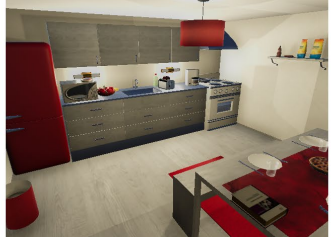

1: Walk to the kitchen

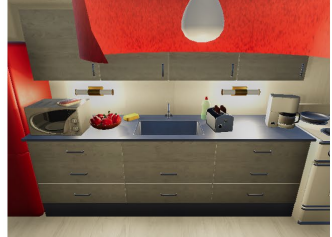

2: Walk to the kitchen counter (1)

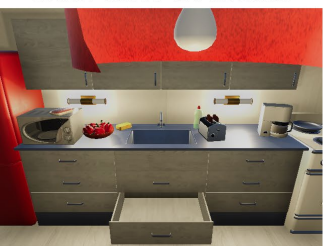

3: Open the kitchen counter

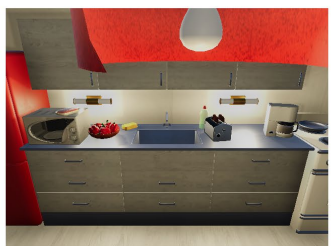

4: Close the kitchen counter

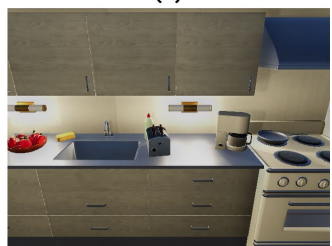

5: Walk to the kitchen cabinet (1)

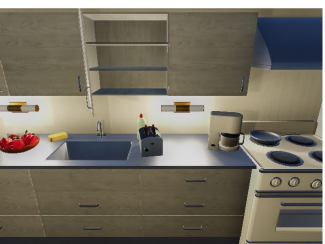

6: Open the kitchen cabinet

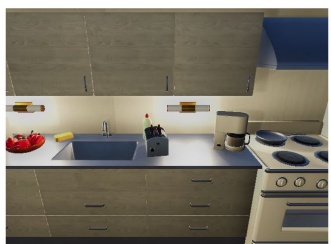

7: Close the kitchen cabinet

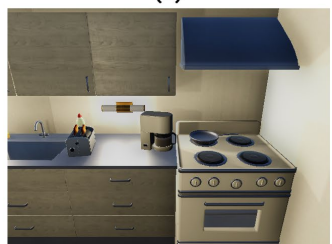

8: Walk to the kitchen cabinet (2)

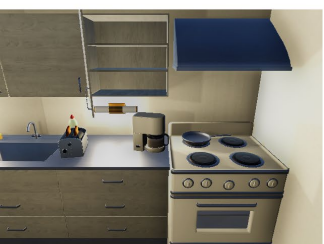

9: Open the kitchen cabinet

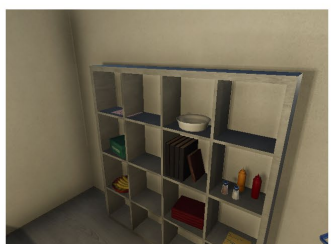

10: Walk to the bookshelf

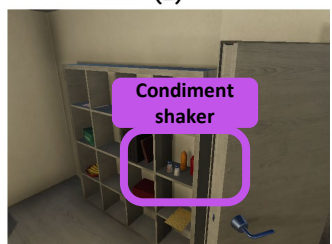

11: Walk to the condimentshaker

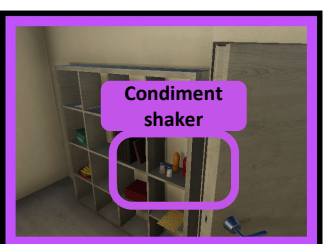

Condiment shaker

Detected object

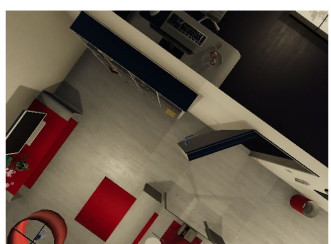

Final state

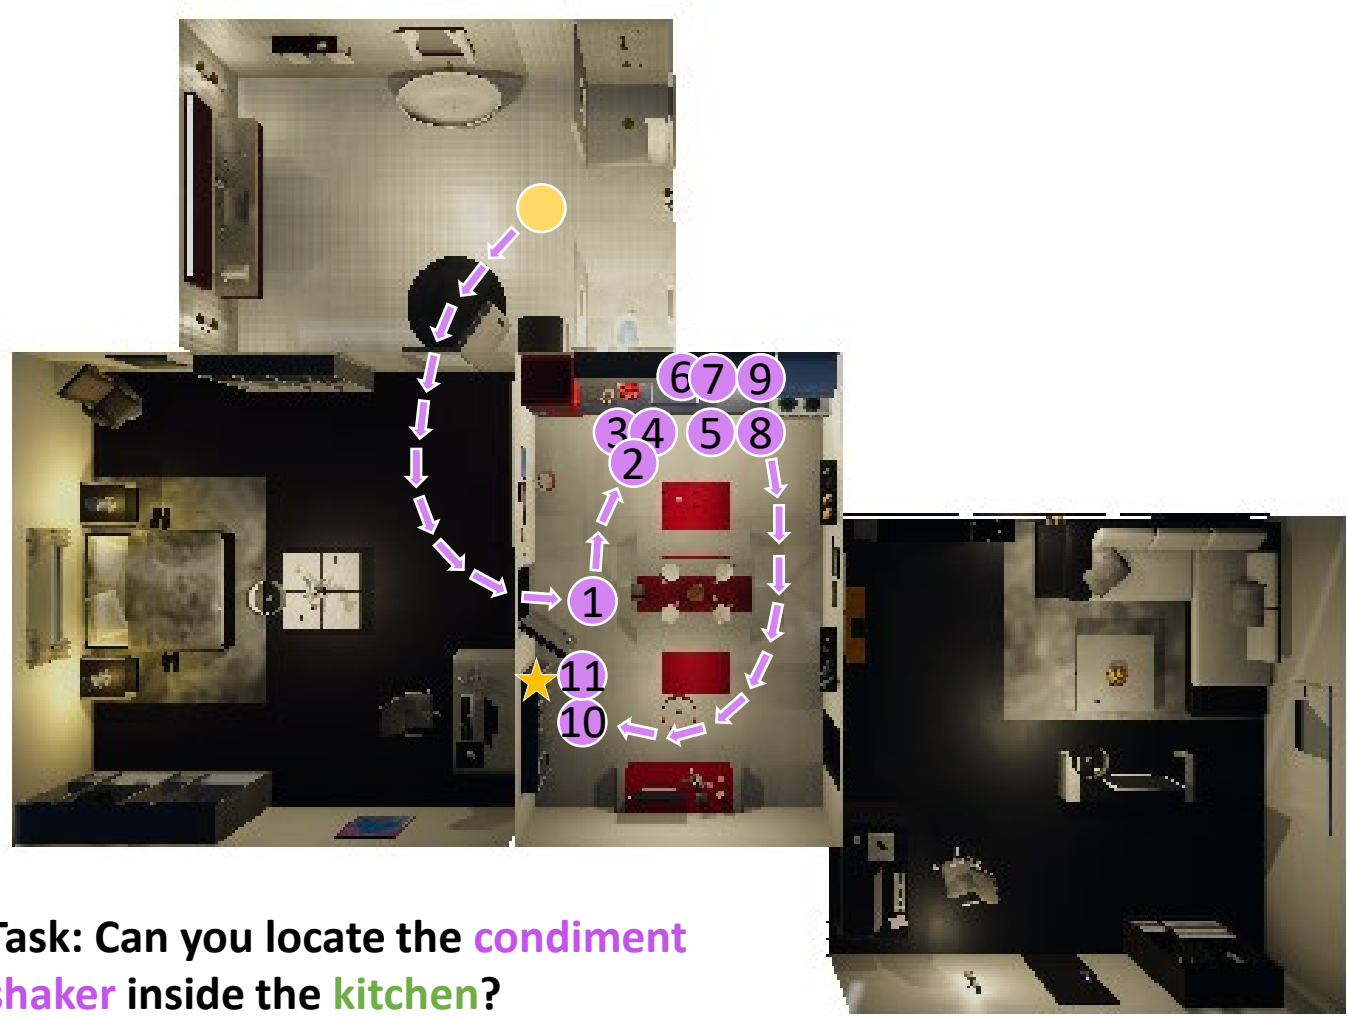

Task: Can you locate the **condiment shaker** inside the **kitchen**?

- 1: Walk to the **kitchen**
- 2: Walk to the kitchen counter (1)
- 3: Open the kitchen counter
- 4: Close the kitchen counter
- 5: Walk to the kitchen cabinet (1)

- 6: Open the kitchen cabinet
- 7: Close the kitchen cabinet
- 8: Walk to the kitchen cabinet (2)
- 9: Open the kitchen cabinet
- 10: Walk to the bookshelf
- 11: Walk to the **condiment shaker**

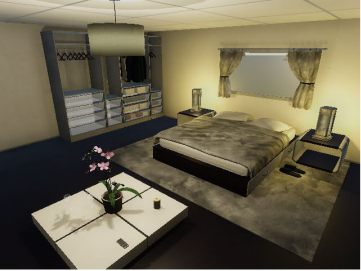

Can you bring me the toothbrush from inside the bathroom?

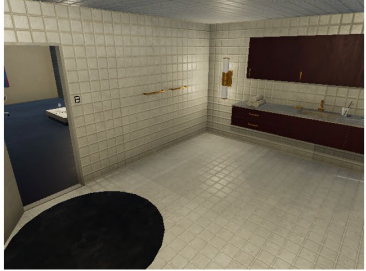

1: Walk to the bathroom

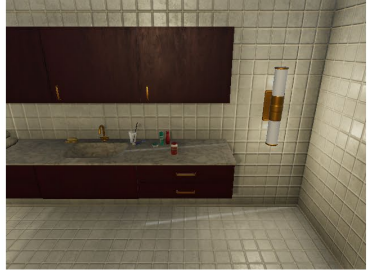

2: Walk to the bathroom counter (1)

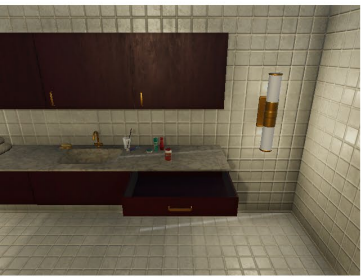

3: Open the bathroom counter

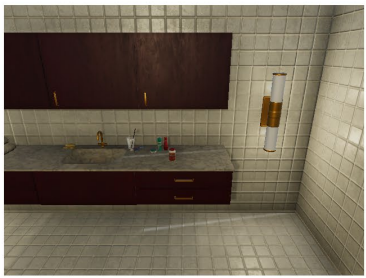

4: Close the bathroom counter

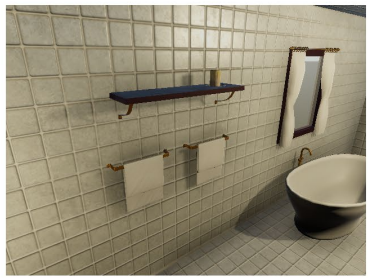

5: Walk to the wall shelf (1)

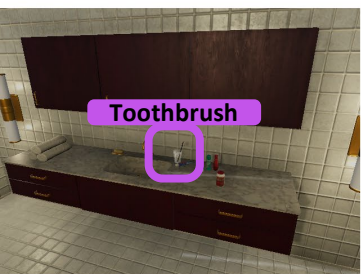

6: Walk to the toothbrush

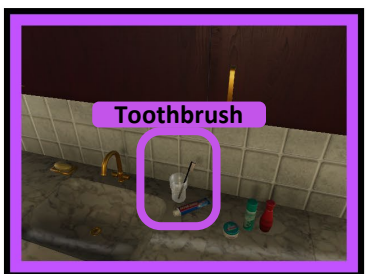

Detected object

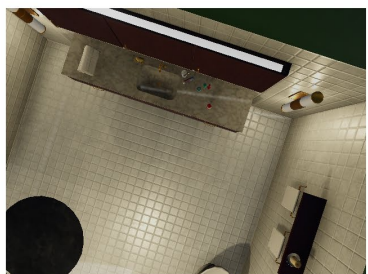

Final state

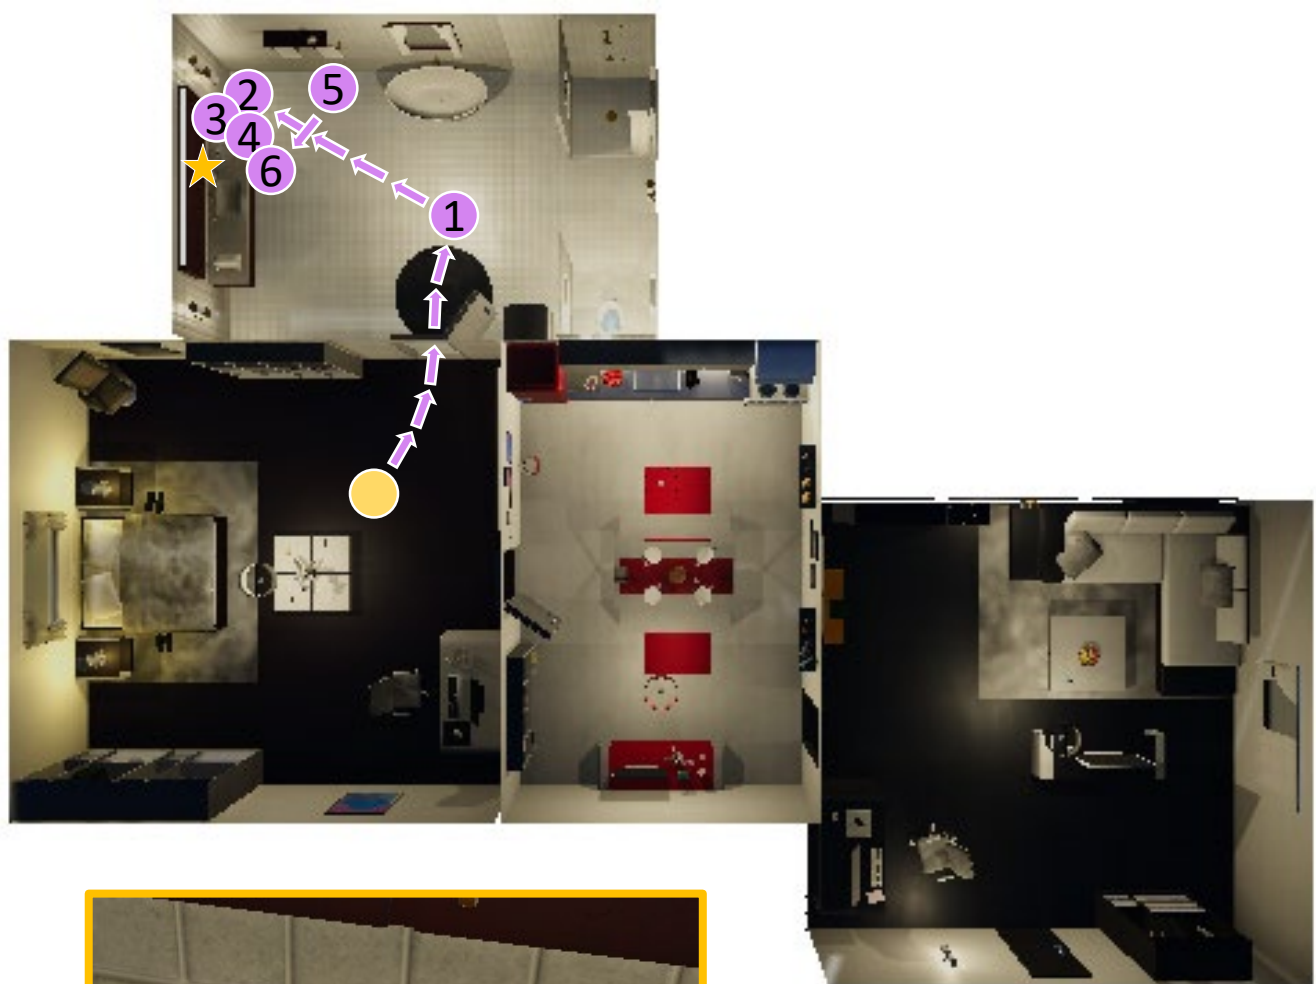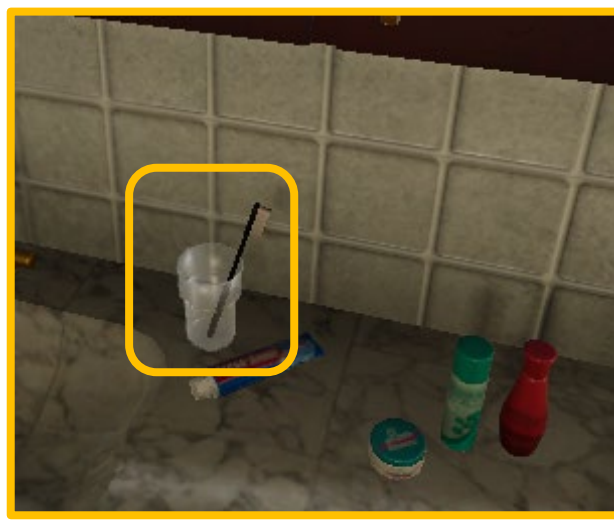

Toothbrush is semi-obstructed by the glass.

Task: Can you bring me the toothbrush from inside the bathroom?

1: Walk to the bathroom  
2: Walk to the bathroom counter (1)

3: Open the bathroom counter  
4: Close the bathroom counter  
5: Walk to the wall shelf (1)  
6: Walk to the toothbrush

NAVI OCCLUSION SIZE FAILURE

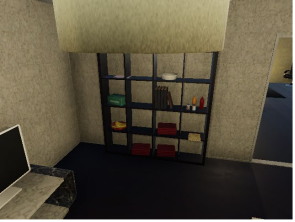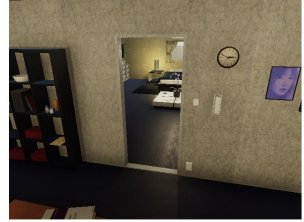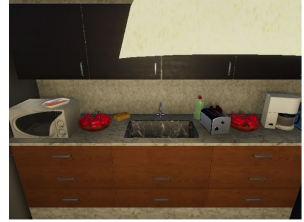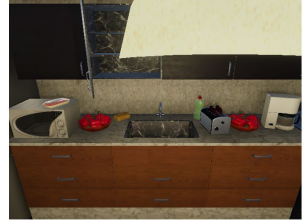

Can you get a cutlery fork from inside the kitchen?

1: Walk to the kitchen

2: Walk to the kitchen cabinet (1)

3: Open the kitchen cabinet

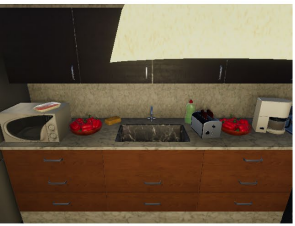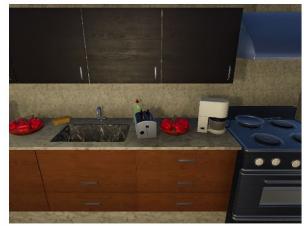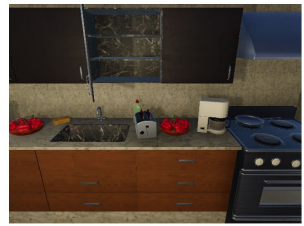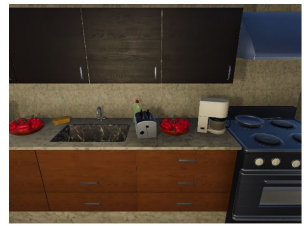

4: Close the kitchen cabinet

5: Walk to the kitchen cabinet (2)

6: Open the kitchen cabinet

7: Close the kitchen cabinet

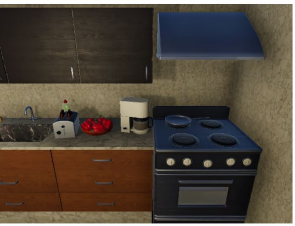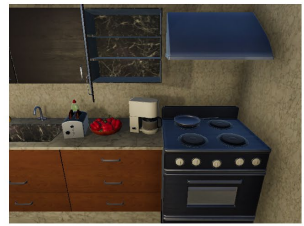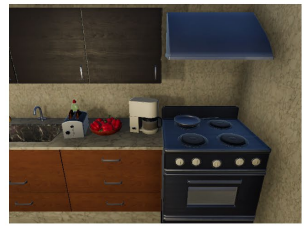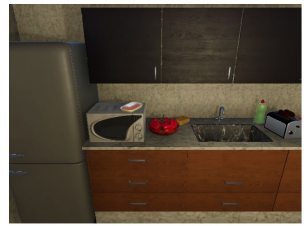

8: Walk to the kitchen cabinet (3)

9: Open the kitchen cabinet

10: Close the kitchen cabinet

11: Walk to the kitchen cabinet (4)

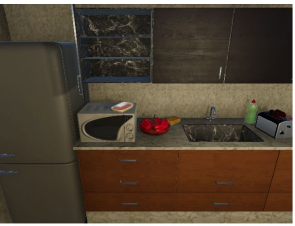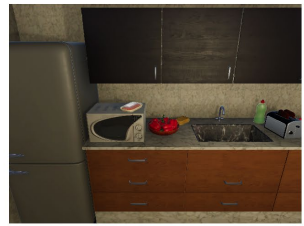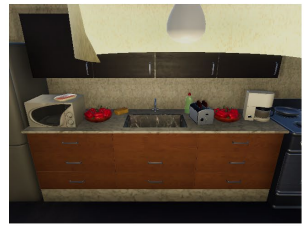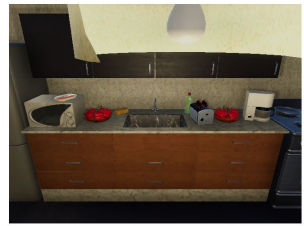

12: Open the kitchen cabinet

13: Close the kitchen cabinet

14: Walk to the kitchen counter (1)

15: Open the kitchen counter

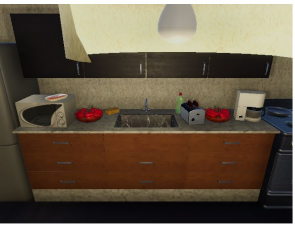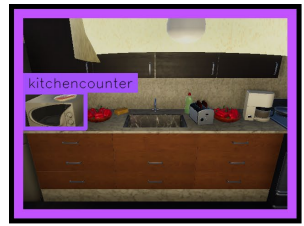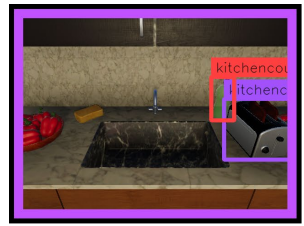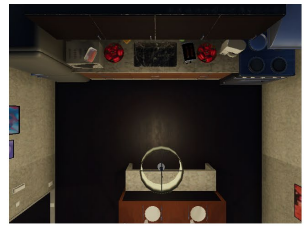

16: Close the kitchen counter

Detected object

Detected object

Final state

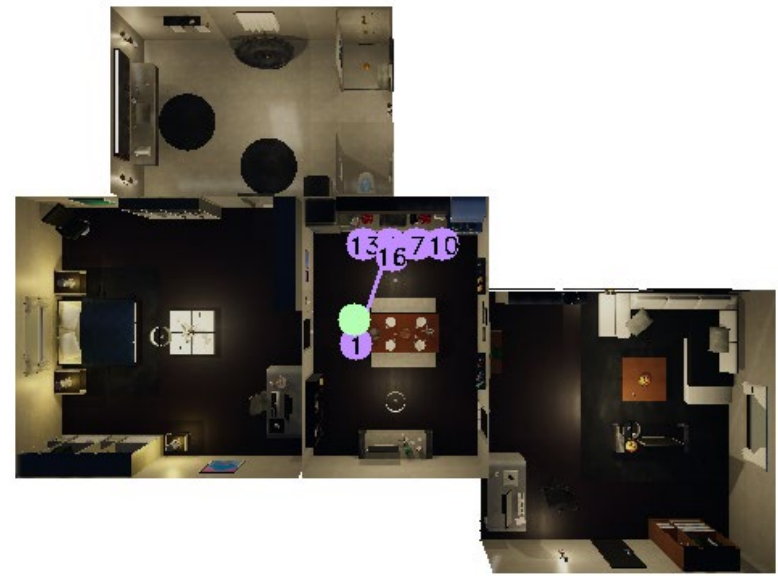

Can you get a cutlery fork from inside the kitchen?

- 1: Walk to the kitchen
- 2: Walk to the kitchen cabinet (1)
- 3: Open the kitchen cabinet
- 4: Close the kitchen cabinet
- 5: Walk to the kitchen cabinet (2)
- 6: Open the kitchen cabinet
- 7: Close the kitchen cabinet
- 8: Walk to the kitchen cabinet (3)

- 9: Open the kitchen cabinet
- 10: Close the kitchen cabinet
- 11: Walk to the kitchen cabinet (4)
- 12: Open the kitchen cabinet
- 13: Close the kitchen cabinet
- 14: Walk to the kitchen counter (1)
- 15: Open the kitchen counter
- 16: Close the kitchen counter

NAVI OCCLUSION DISTANCE  
SUCCESS

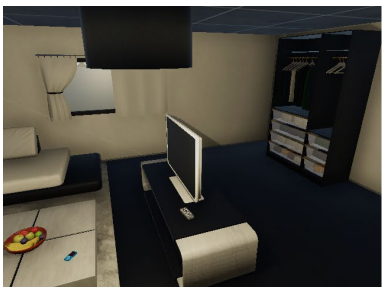

Can you find the candle inside the bedroom?

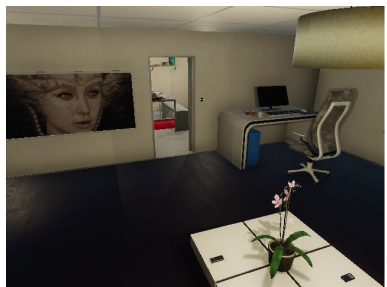

1: Walk to the bedroom

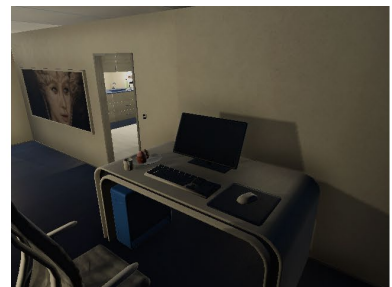

2: Walk to the desk

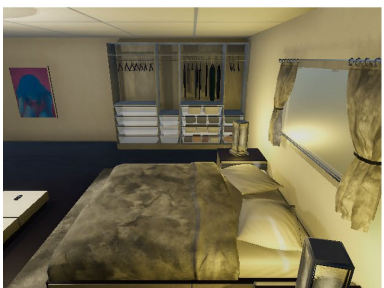

3: Walk to the bed

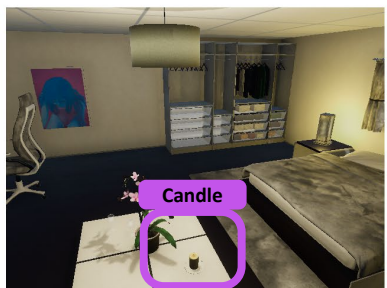

4: Walk to the candle

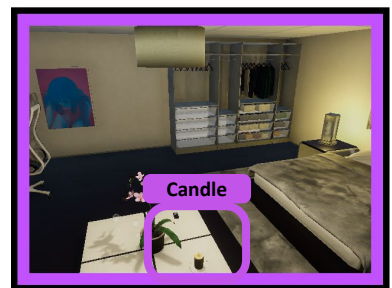

Detected object

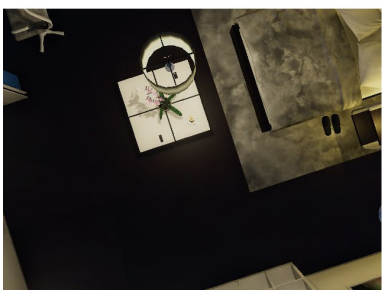

Final state

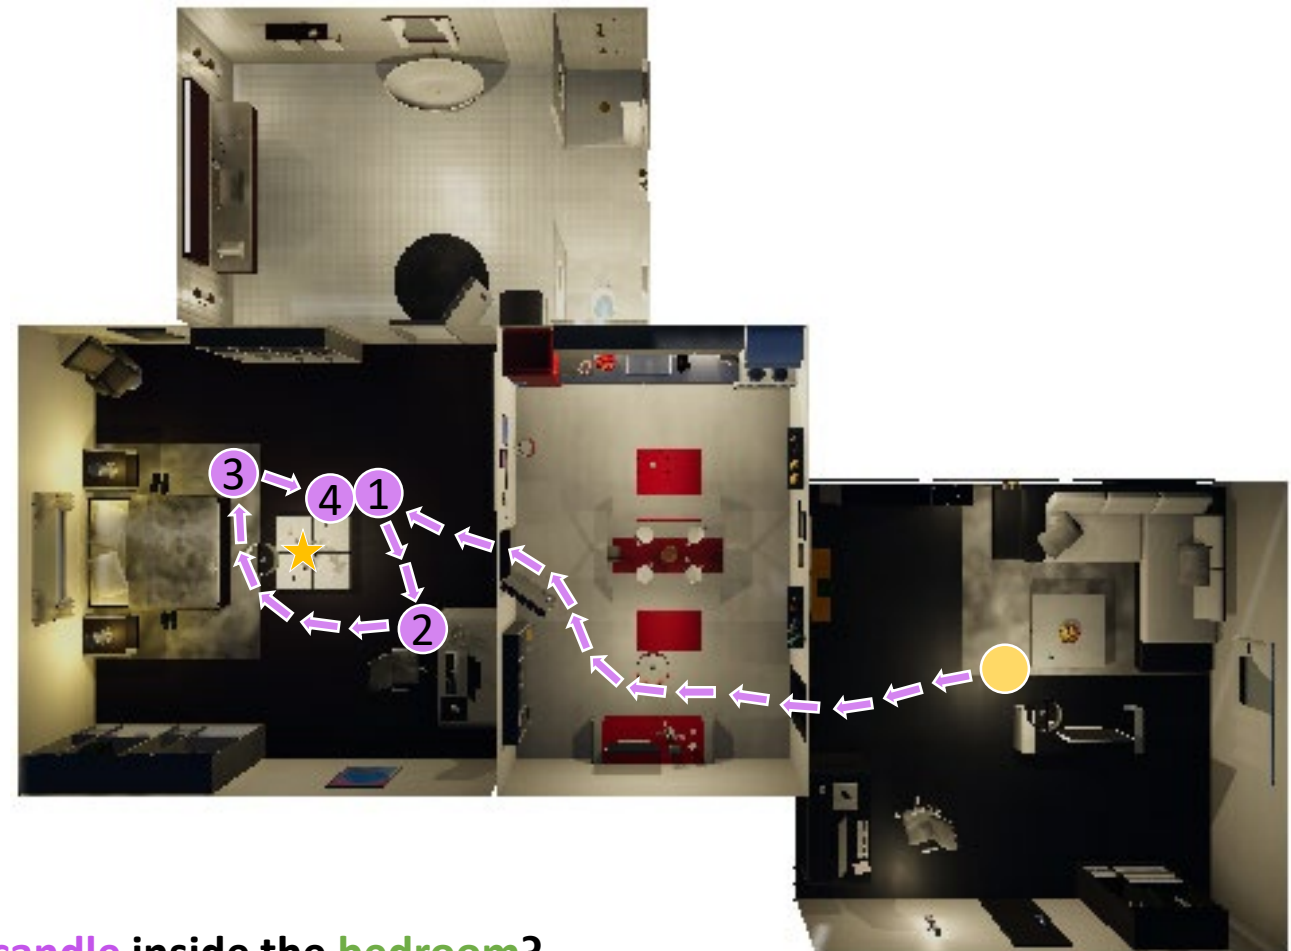

**Task:** Can you find the **candle** inside the **bedroom**?

1: Walk to the **bedroom**

2: Walk to the desk

3: Walk to the bed

4: Walk to the **candle**

NAVI OCCLUSION DISTANCE  
FAILURE

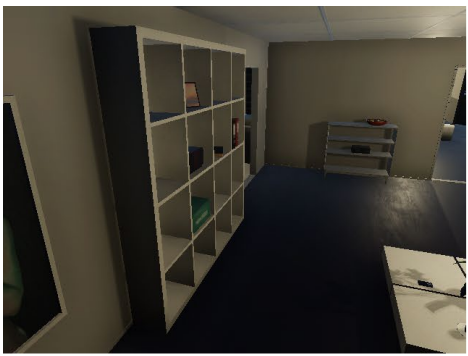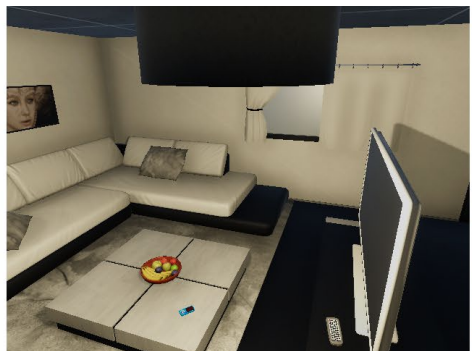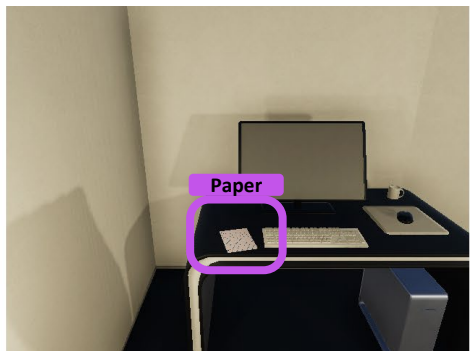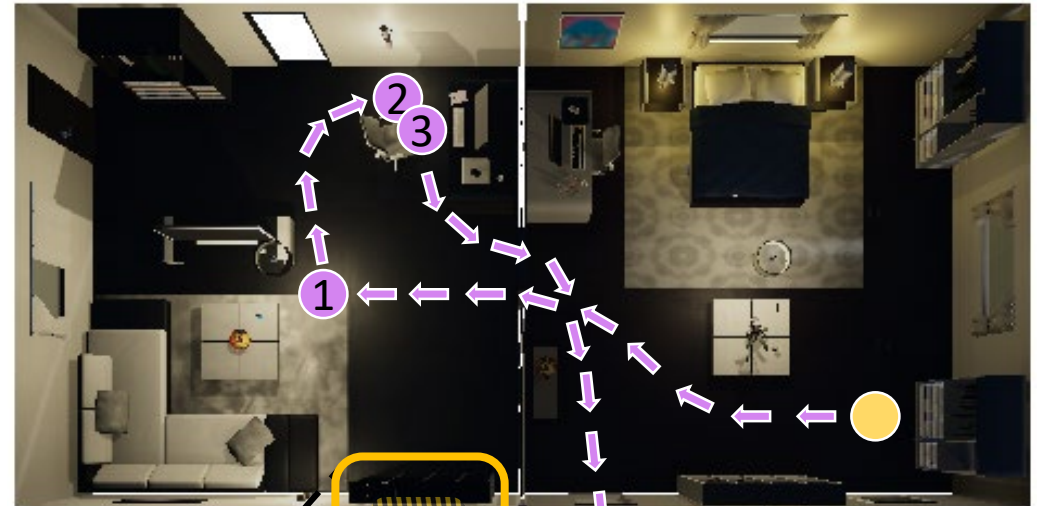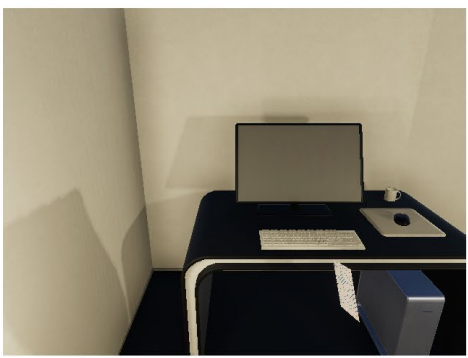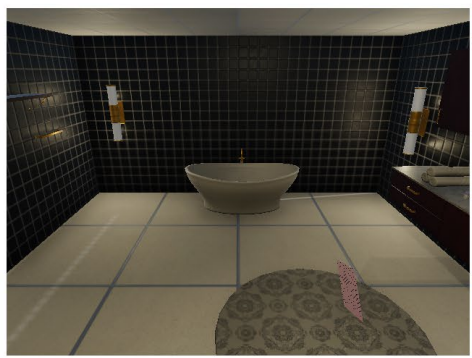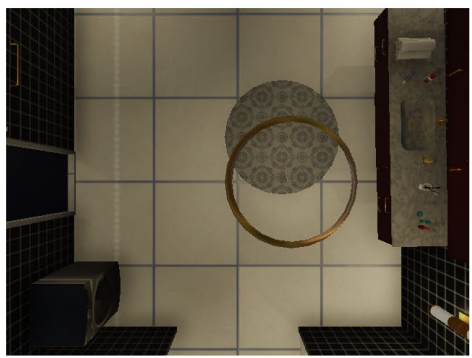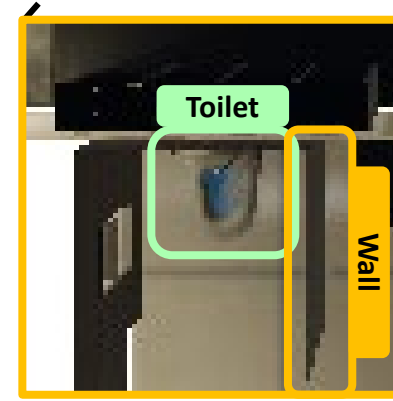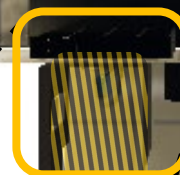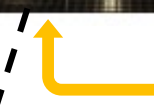

Unexplored area

The toilet was blocked by a wall and the LLM decided not to explore near this area.

Your task is to get paper inside livingroom and move it to toilet inside bathroom.

Your task is to get **paper** inside livingroom and move it to **toilet** inside bathroom.

- 1: Walk to the livingroom
- 2: Walk to the **paper**
- 3: Grab the **paper**
- 4: Walk to the bathroom

1: Walk to the livingroom

2: Walk to the paper

3: Grab the paper

4: Walk to the bathroom

Final state

*Navi & Manipulation + multiple  
objects*  
Success

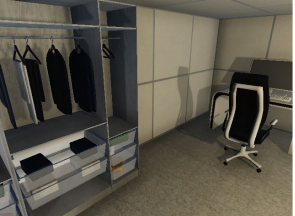

Find a wineglass and a mug, then put them on the kitchen cabinet

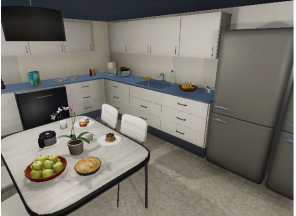

1: Walk to the kitchen

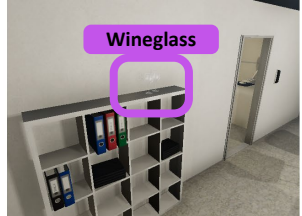

2: Walk to the wineglass

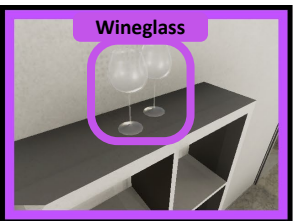

3: Grab the wineglass

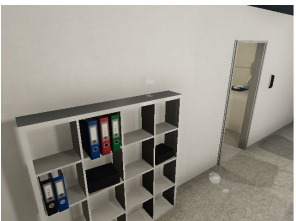

3: Grab the wineglass

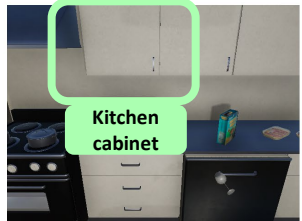

4: Walk to the kitchen cabinet (1)

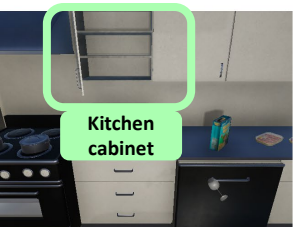

5: Open the kitchen cabinet

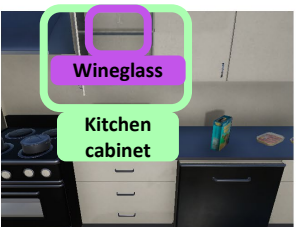

6: Put the wineglass inside the kitchen cabinet

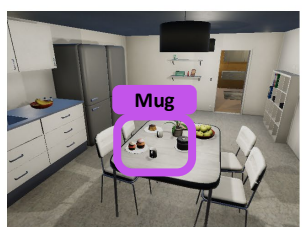

7: Walk to the mug

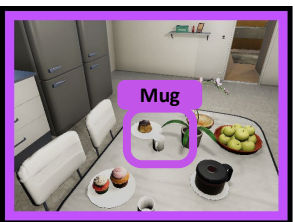

8: Grab the mug

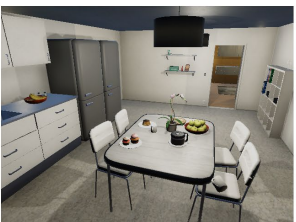

8: Grab the mug

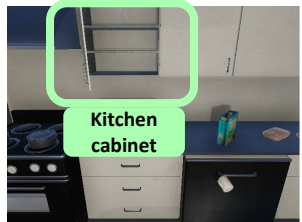

9: Walk to the kitchen cabinet (1)

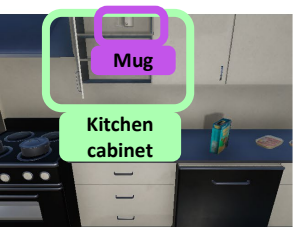

10: Put the mug inside the kitchen cabinet

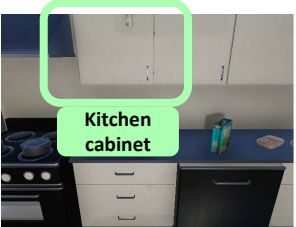

11: Close the kitchen cabinet

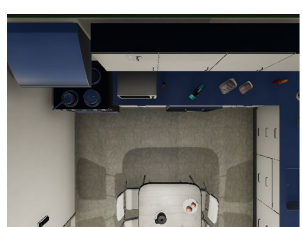

Final state

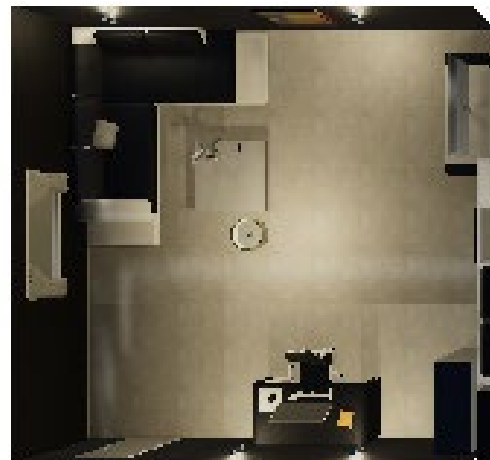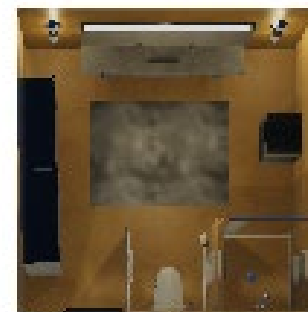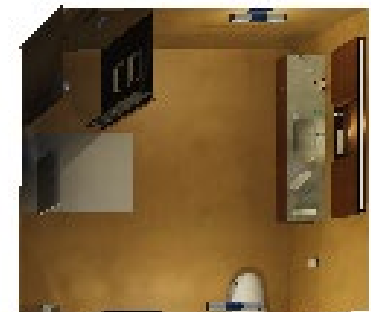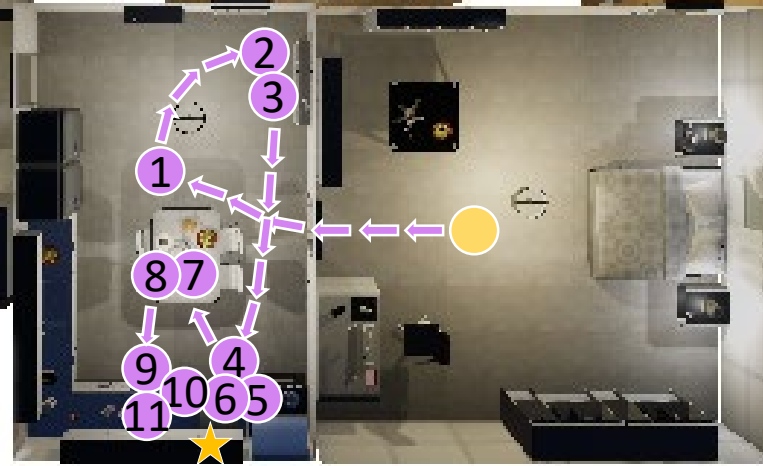

Task: Find a **wineglass** and a **mug**, then put them on the **kitchen cabinet**

1: Walk to the kitchen

2: Walk to the **wineglass**

3: Grab the **wineglass**

4: Walk to the **kitchen cabinet** (1)

5: Open the **kitchen cabinet**

6: Put the wineglass inside the **kitchen cabinet**

7: Walk to the **mug**

8: Grab the **mug**

9: Walk to the **kitchen cabinet** (1)

10: Put the mug inside the **kitchen cabinet**

11: Close the **kitchen cabinet**

*Navi & Manipulation + multiple  
objects*

FAILURE

*Navi & Manipulation + optimal path*

Success

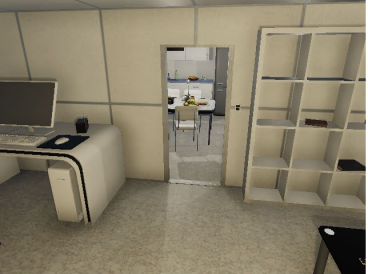

Gather the coffeepot and wineglass and then lay them into then dishwasher.

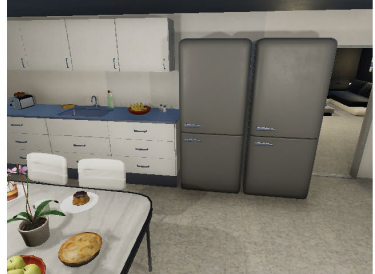

1: Walk to the kitchen

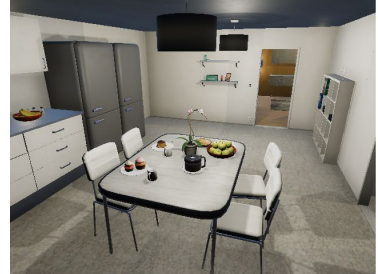

2: Walk to the coffeepot

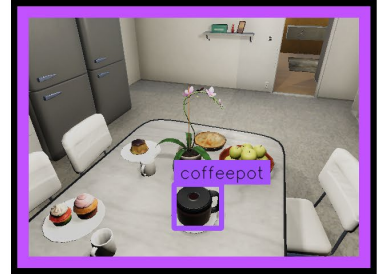

3: Grab the coffeepot

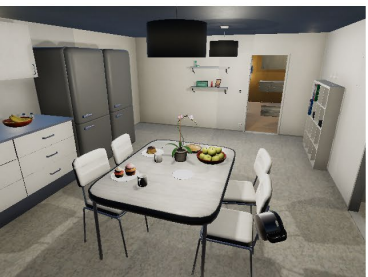

3: Grab the coffeepot

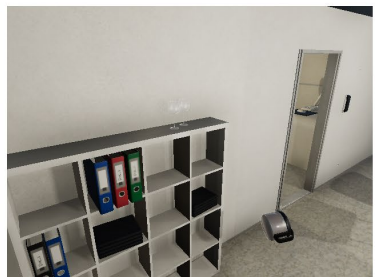

4: Walk to the wineglass

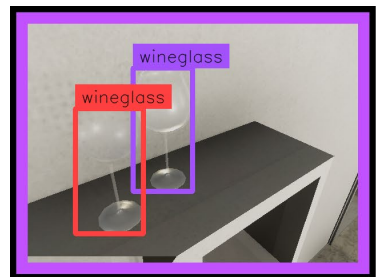

5: Grab the wineglass

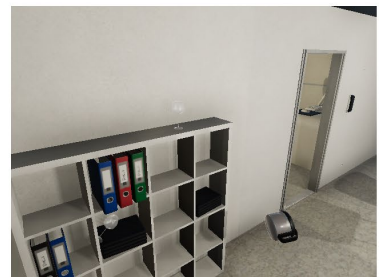

5: Grab the wineglass

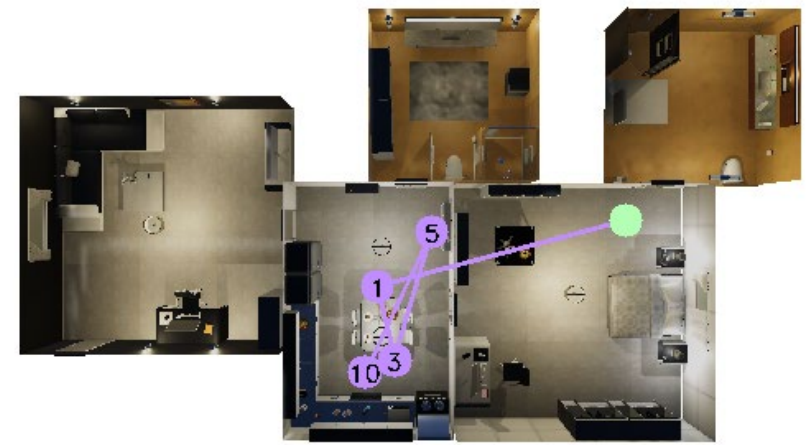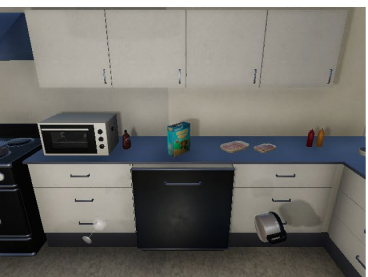

6: Walk to the dishwasher

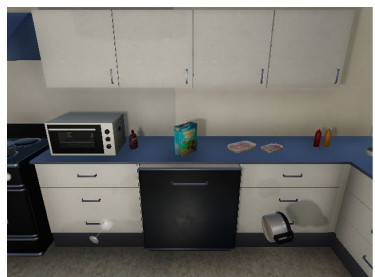

7: Open the dishwasher

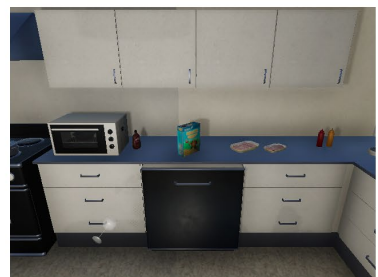

8: Put the coffeepot inside the dishwasher

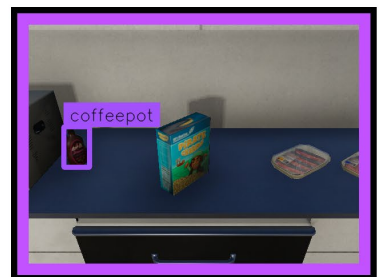

8: Put the coffeepot inside the dishwasher

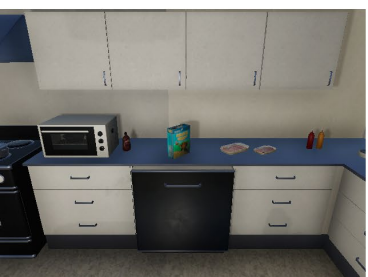

9: Put the wineglass inside the dishwasher

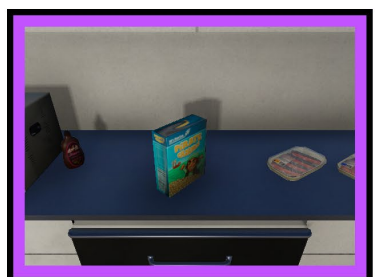

9: Put the wineglass inside the dishwasher

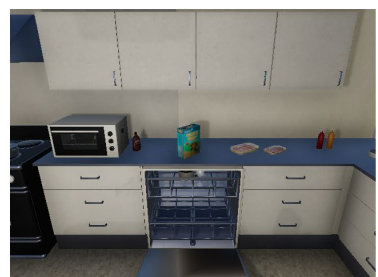

10: Close the dishwasher

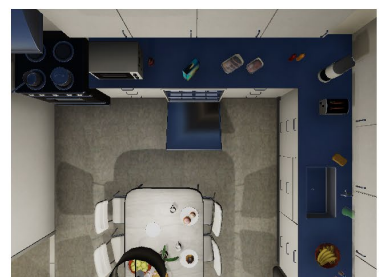

Final state

*Navi & Manipulation + optimal path*

FAILURE

*Navi & Manipulation + temp  
dependency*

Success

*Navi & Manipulation + temp  
dependency*

FAILURE
