# Supplementary material for: ET-Plan-Bench: Embodied Task-level Planning Benchmark Towards Spatial-Temporal Cognition with Foundation Models
Source: arXiv:2410.14682 source file (2025-02-13)
Supplement: Supplementary file 2 [file selected_success_failure_cases_appendix_fixed.pdf]

# Pages index

- Navigation Tasks with or without Spatial Constraints
  - Navi + Layout Map
  - Navi
  - Navi + Occlusion\_Size
  - Navi + Occlusion\_Distance
  - Navi + Relation
  - Navi + Relation + Occlusion\_Size
  - Navi + Relation + Occlusion\_Distance
- Navigation & Manipulation Tasks with or without Spatial Constraints
  - Navi & Mani + Layout Map
  - Navi & Mani
  - Navi & Mani + Occlusion\_Size
  - Navi & Mani + Occlusion\_Distance
  - Navi & Mani + Relation
  - Navi & Mani + Relation + Occlusion\_Size
  - Navi & Mani + Relation + Occlusion\_Distance
- Navigation & Manipulation Tasks with Temporal Constraints
  - Navi & Mani + Multi Objects
  - Navi & Mani + Multi Objects + Optimal Path with 2 Arms
  - Navi & Mani + Multi Objects + Temp Dependency

Navi or Navi & Manipulation

Navi or Navi & Manipulation + relation (pick two relations, something like “face to”, ‘next to’)

Navi or Navi & Manipulation + occlusion size

Navi or Navi & Manipulation + distance

Navi & Manipulation + multiple objects

Navi & Manipulation + optimal path

Navi & Manipulation + temp dependency

| Task                                                  | Success | Failure |
|-------------------------------------------------------|---------|---------|
| Navi                                                  | 1       | 1       |
| Navi & Manipulation                                   | 1       |         |
| Navi + relation                                       | 3       | 1       |
| Navi & Manipulation + relation                        |         |         |
| Navi + occlusion size                                 | 2       | 1       |
| Navi & Manipulation + occlusion size                  | 1       |         |
| Navi + distance                                       | 1       |         |
| Navi & Manipulation + distance                        |         | 1       |
| Navi & Manipulation + multiple objects                | 1       |         |
| Navi & Manipulation + multiple objects + optimal path | 1       |         |
| Navi & Manipulation + temp dependency                 | -----   | -----   |

NAVI / NAVI & MANI  
SUCCESS

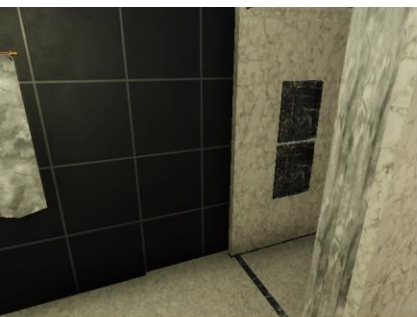

Can you lead me to the desk?

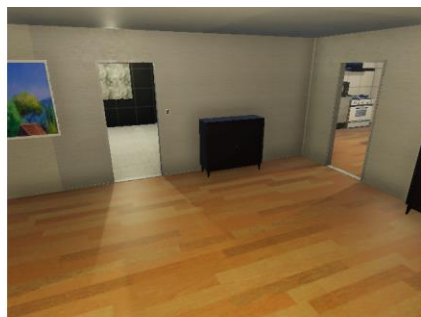

1: Walk to the bedroom

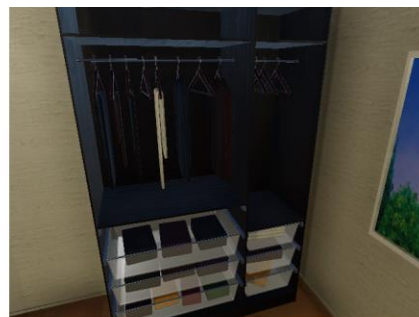

2: Walk to the closet

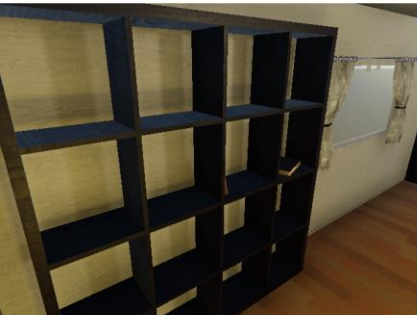

3: Walk to the bookshelf

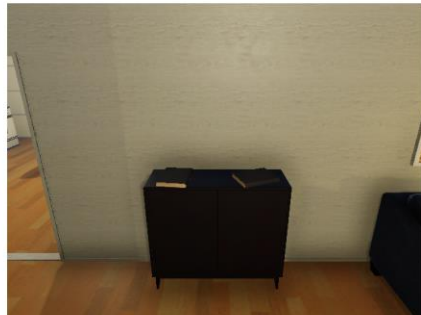

4: Walk to the cabinet (1)

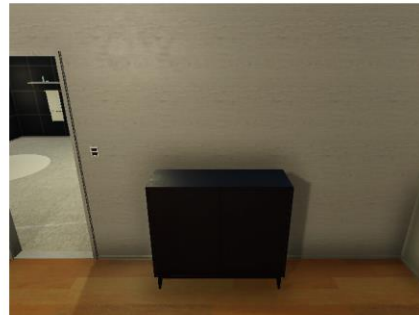

5: Walk to the cabinet (2)

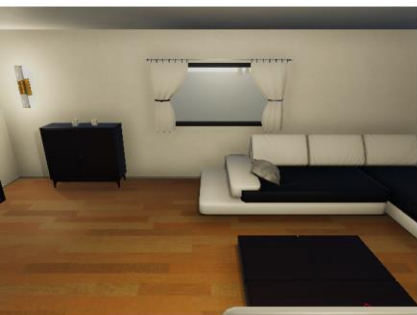

6: Walk to the livingroom

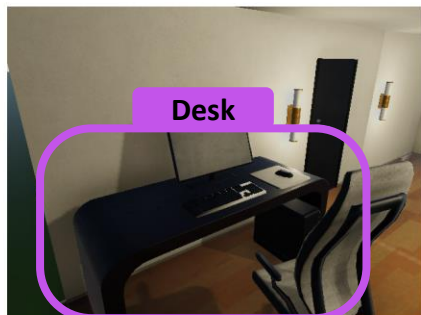

7: Walk to the desk

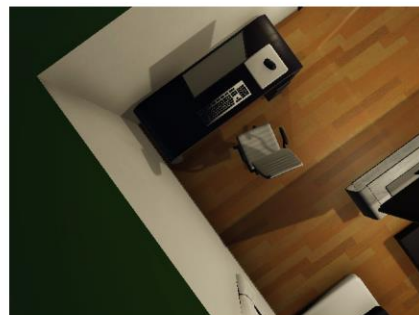

Final state

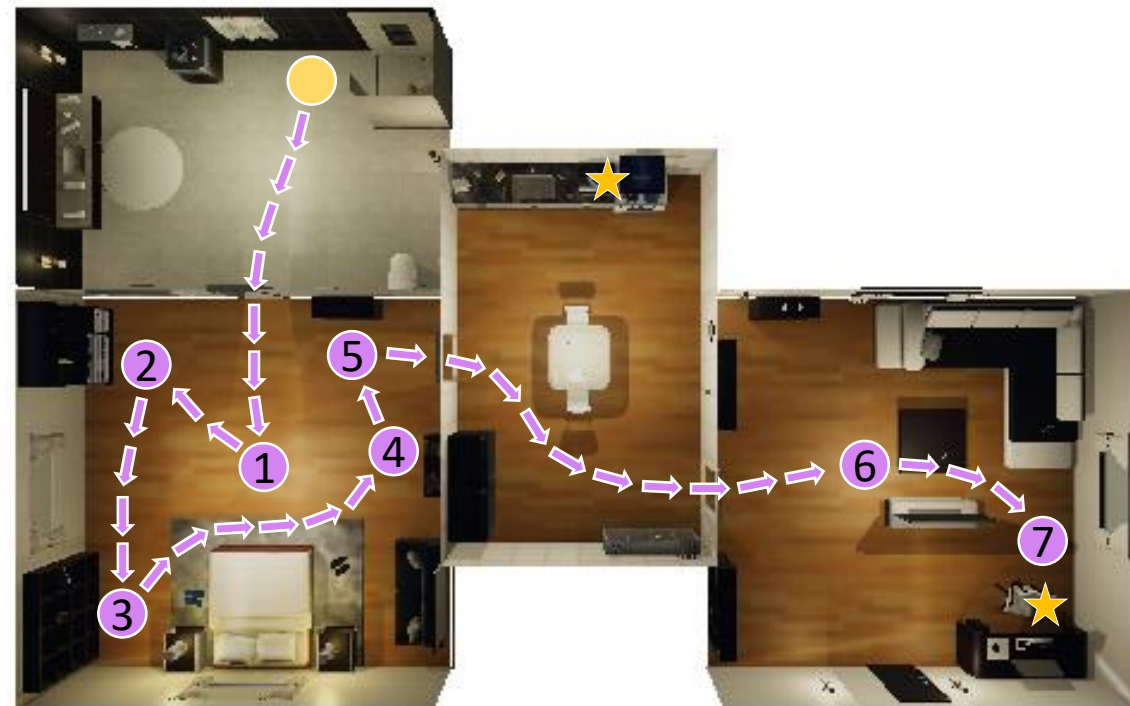

## Navigation

Task: Can you lead me to the **desk**?

1: Walk to the bedroom

2: Walk to the closet

3: Walk to the cabinet (1)

4: Walk to the cabinet (2)

5: Walk to the bookshelf

6: Walk to the livingroom

7: Walk to the **desk**

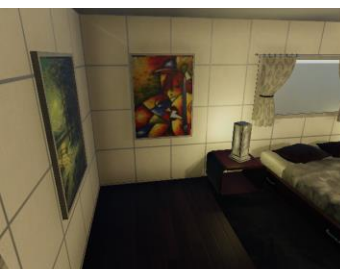

Please place the cutlets on the kitchen table.

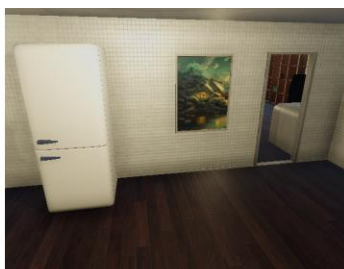

1: Walk to the kitchen

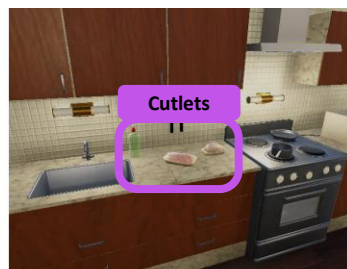

2: Walk to the cutlets

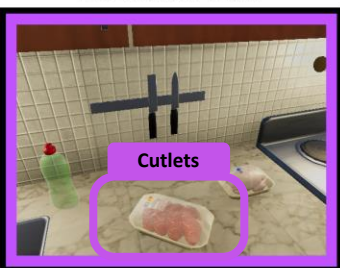

3: Grab the cutlets

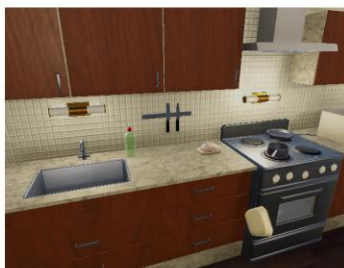

3: Grab the cutlets

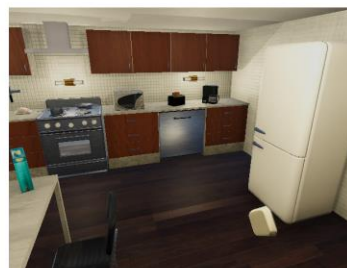

4: Walk to the kitchen

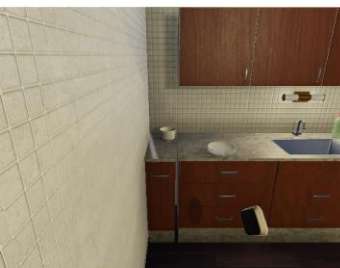

5: Walk to the kitchen counter (1)

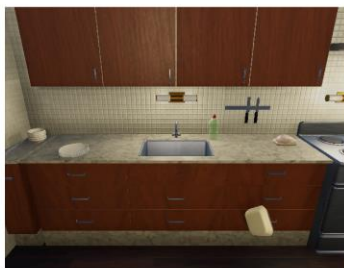

6: Walk to the kitchen counter (2)

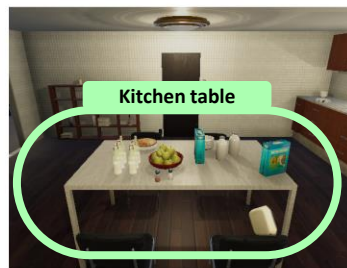

7: Walk to the kitchentable

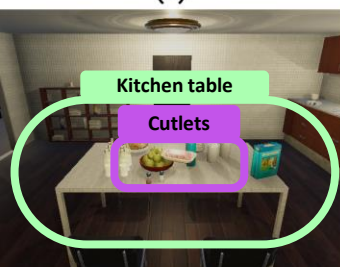

8: Put the cutlets in the kitchentable

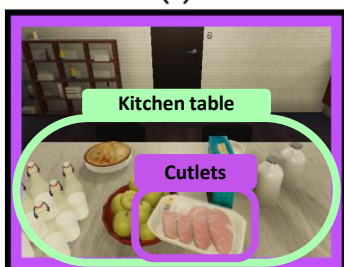

8: Put the cutlets in the kitchentable

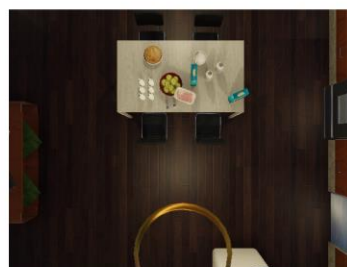

Final state

## Navi & Mani

Task: Please place the **cutlets** on the **kitchen table**.

- 1: Walk to the kitchen
- 2: Walk to the **cutlets**
- 3: Grab the **cutlets**
- 4: Walk to the kitchen

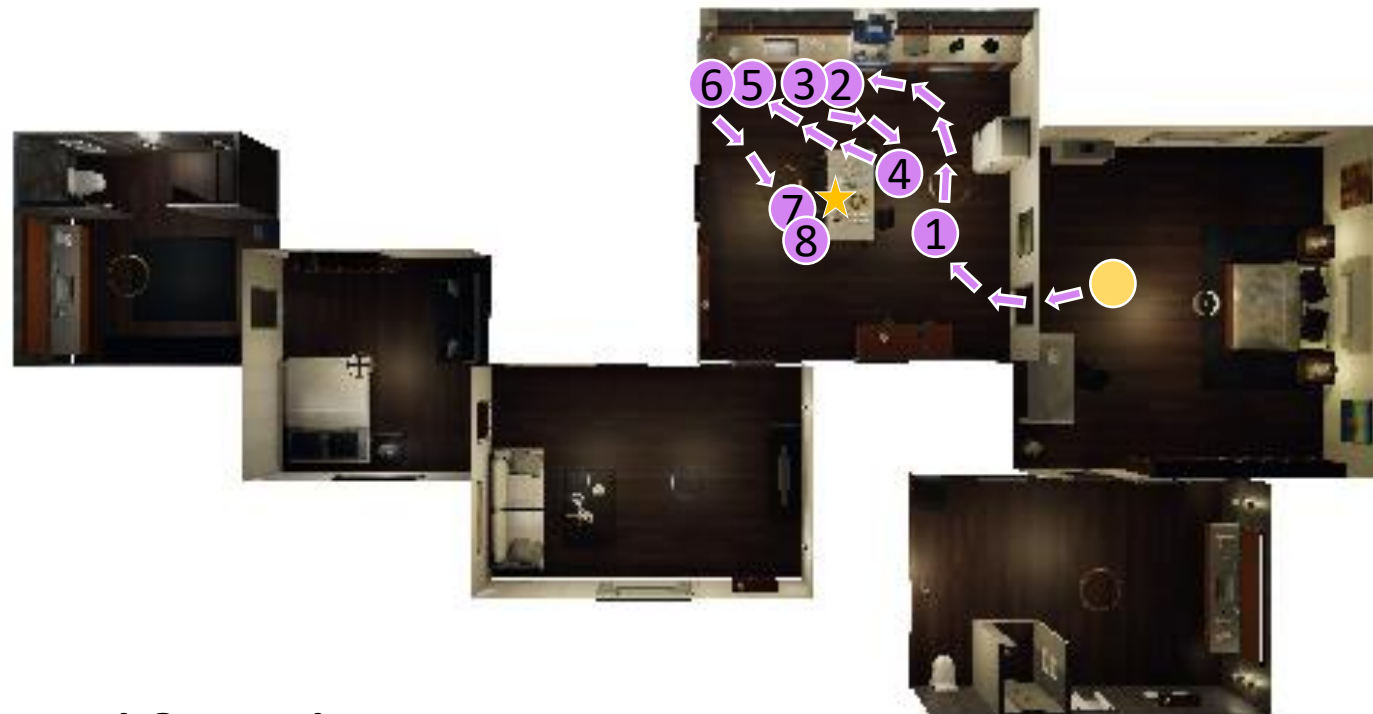

- 5: Walk to the kitchen counter (1)
- 6: Walk to the kitchen counter (2)
- 7: Walk to the **kitchen table**
- 8: Put the cutlets in the **kitchen table**

NAVI

FAILURE

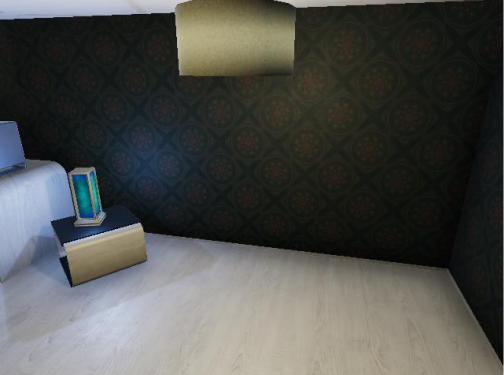

Can you show me where the bench is?

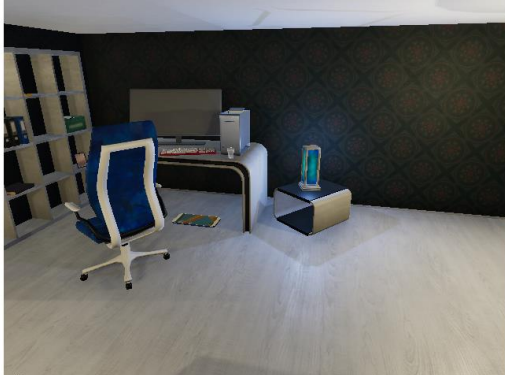

1: Walk to the livingroom

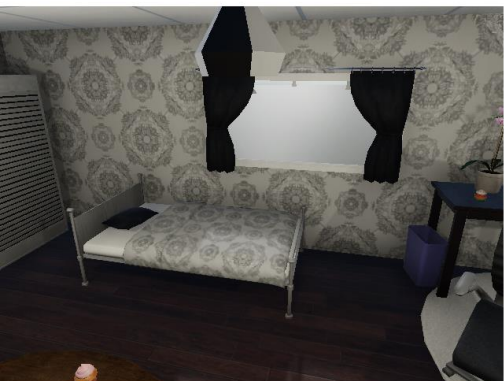

2: Walk to the bedroom

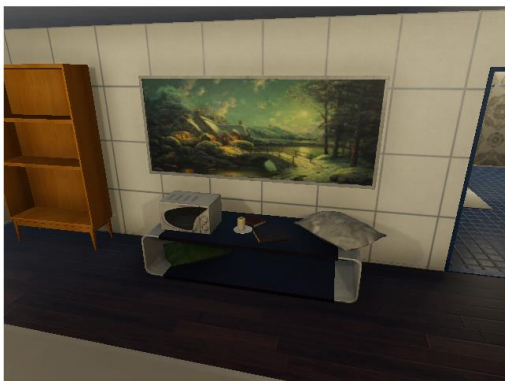

3: Walk to the kitchen

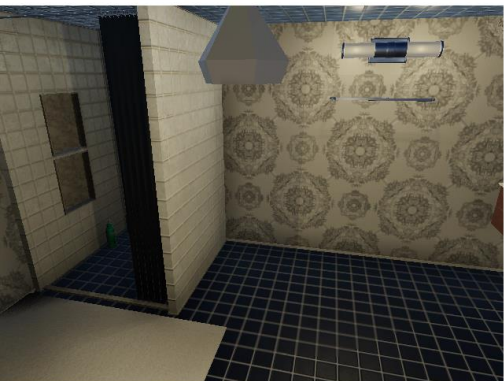

4: Walk to the bathroom

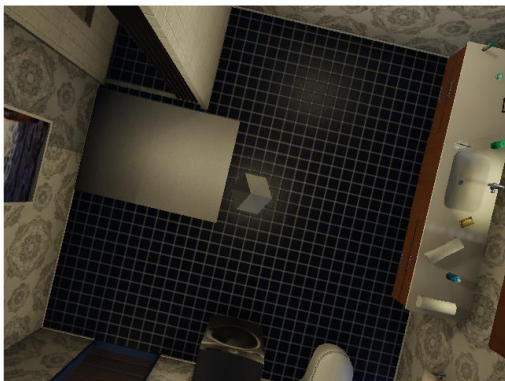

Final state

# Navigation

Task: Can you show me where the bench is?

- 1: Walk to the livingroom
- 2: Walk to the bedroom
- 3: Walk to the kitchen
- 4: Walk to the bathroom

The LLM decided not to explore any of the rooms other than the initial observation.

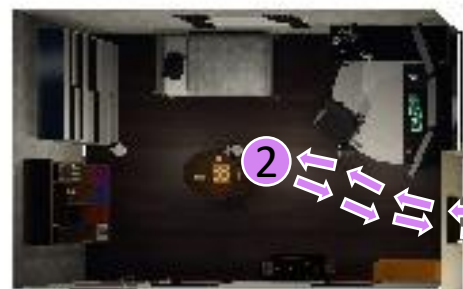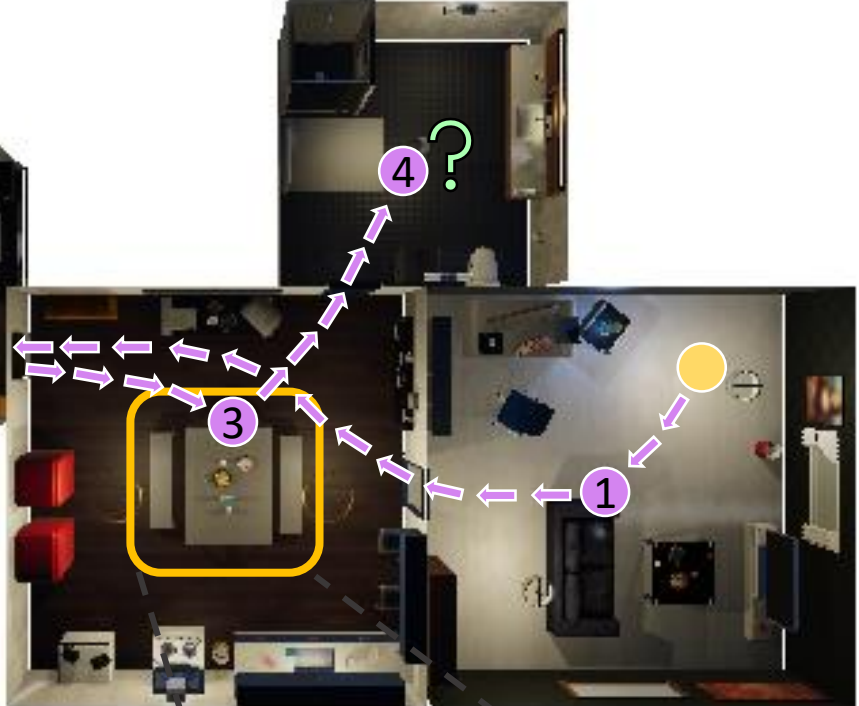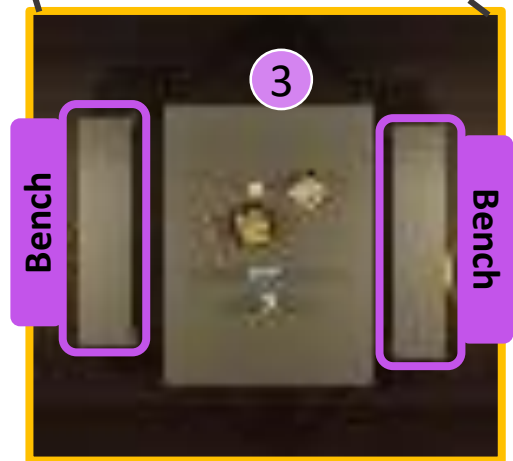

Both benches are obscured by the table.

NAVI RELATION  
SUCCESS

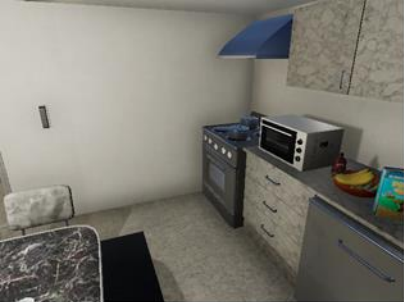

Can you get the box on the wall shelf?

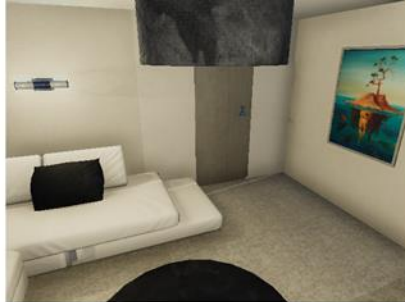

1: Walk to the livingroom

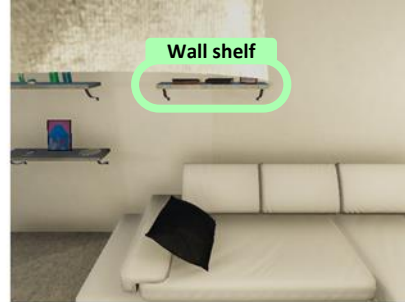

2: Walk to the wall shelf (1)

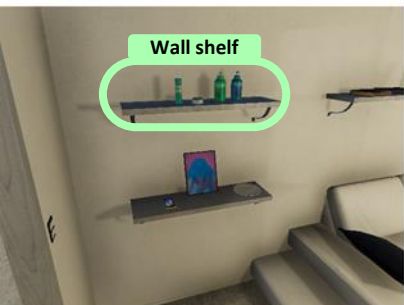

3: Walk to the wall shelf (2)

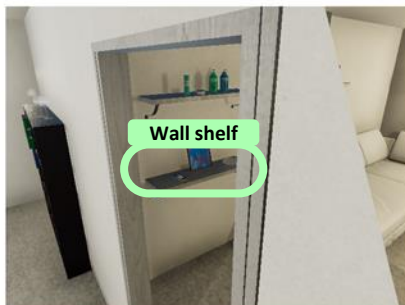

4: Walk to the wall shelf (3)

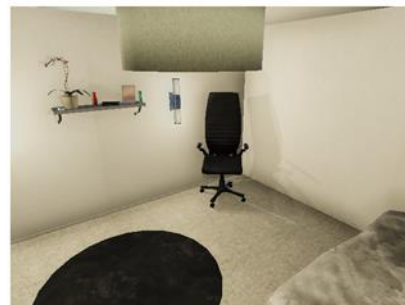

5: Walk to the bedroom

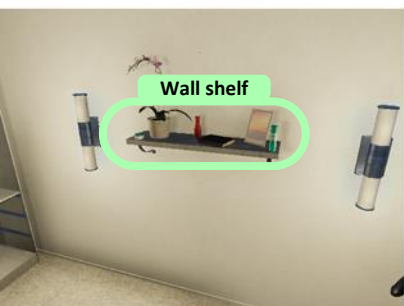

6: Walk to the wall shelf (4)

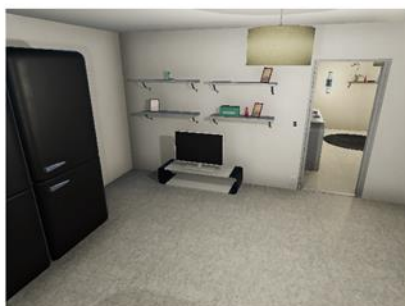

7: Walk to the kitchen

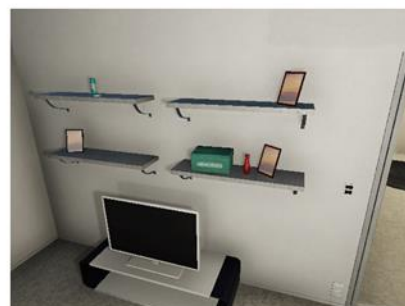

8: Walk to the box

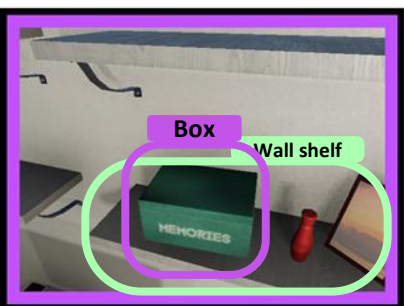

Detected object

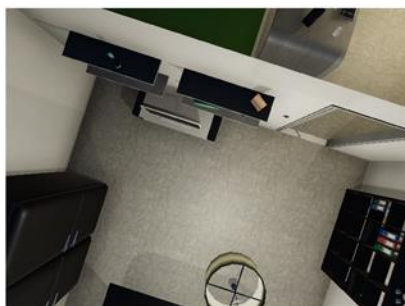

Final state

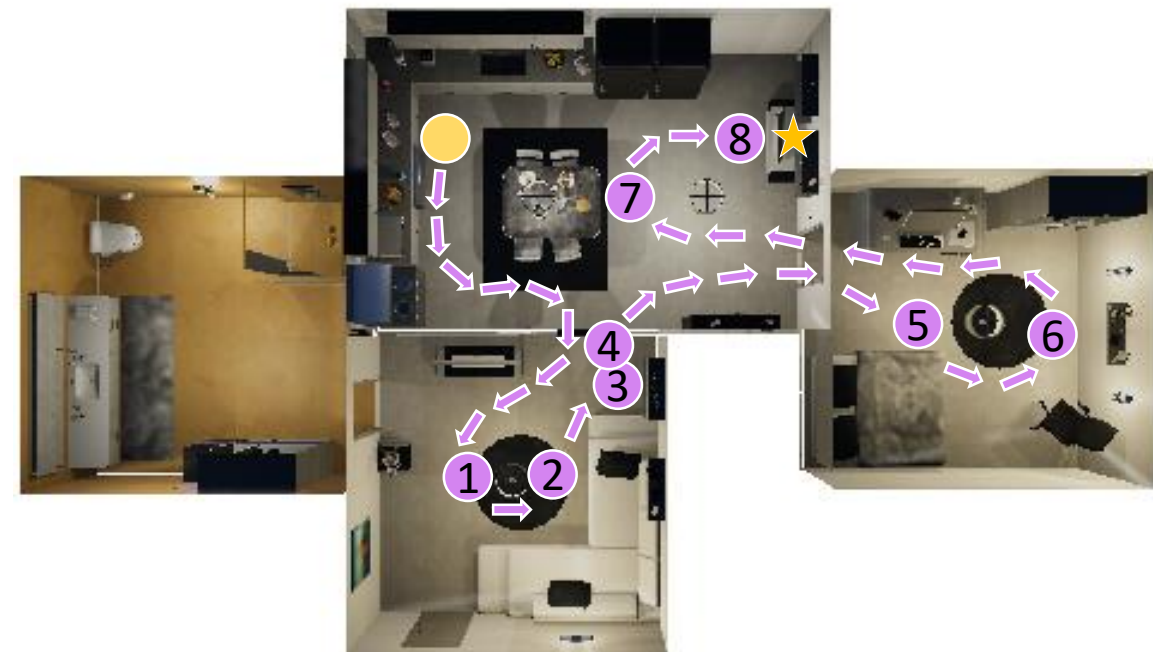

## Navi + Relation

Task: Can you get the **box** on the **wall shelf**?

- 1: Walk to the livingroom
- 2: Walk to the **wall shelf** (1)
- 3: Walk to the **wall shelf** (2)
- 4: Walk to the **wall shelf** (3)
- 5: Walk to the bedroom
- 6: Walk to the **wall shelf** (4)
- 7: Walk to the kitchen
- 8: Walk to the **box**

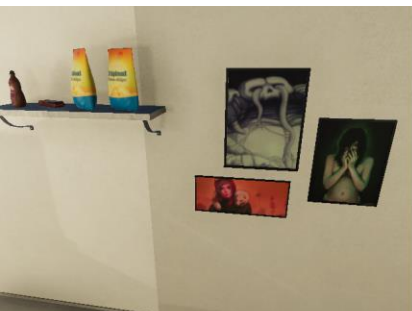

Can you bring me the pie facing the TV?

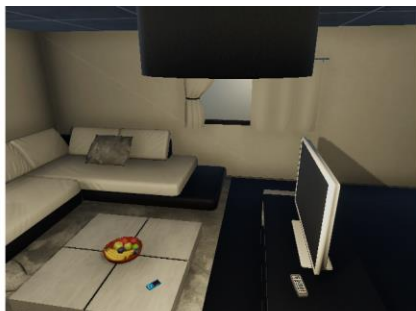

1: Walk to the livingroom

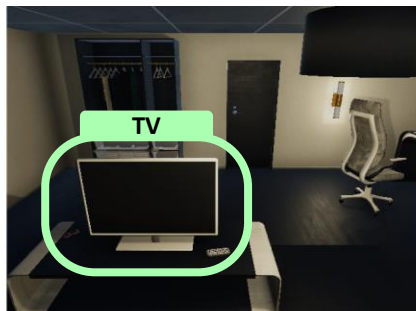

2: Walk to the tv (1)

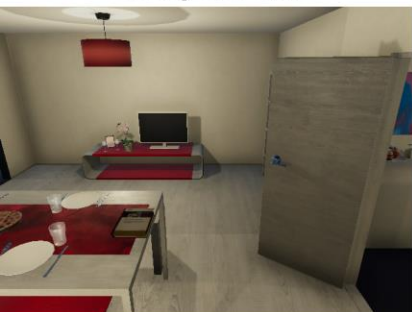

3: Walk to the kitchen

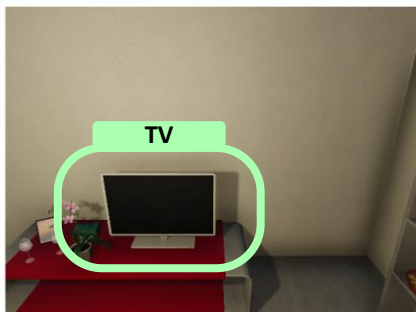

4: Walk to the tv (2)

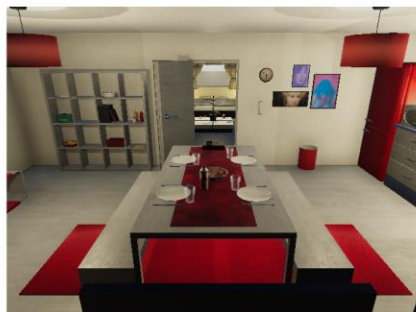

5: Walk to the pie

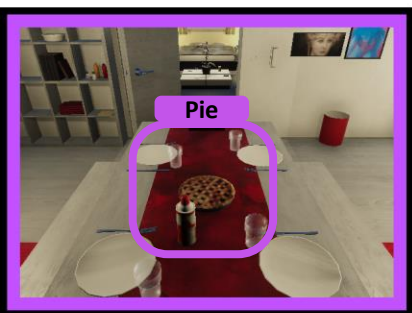

Detected object

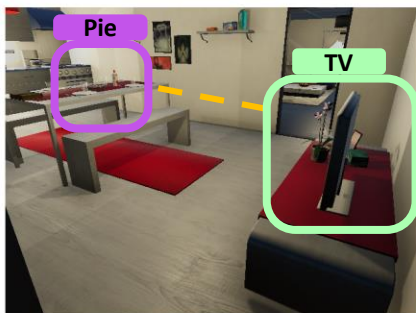

Final state

## Navi + Relation

Task: Can you bring me the **pie** facing the **TV**?

- 1: Walk to the livingroom
- 2: Walk to the **tv** (1)
- 3: Walk to the **tv** (2)
- 4: Walk to the kitchen
- 5: Walk to the **pie**

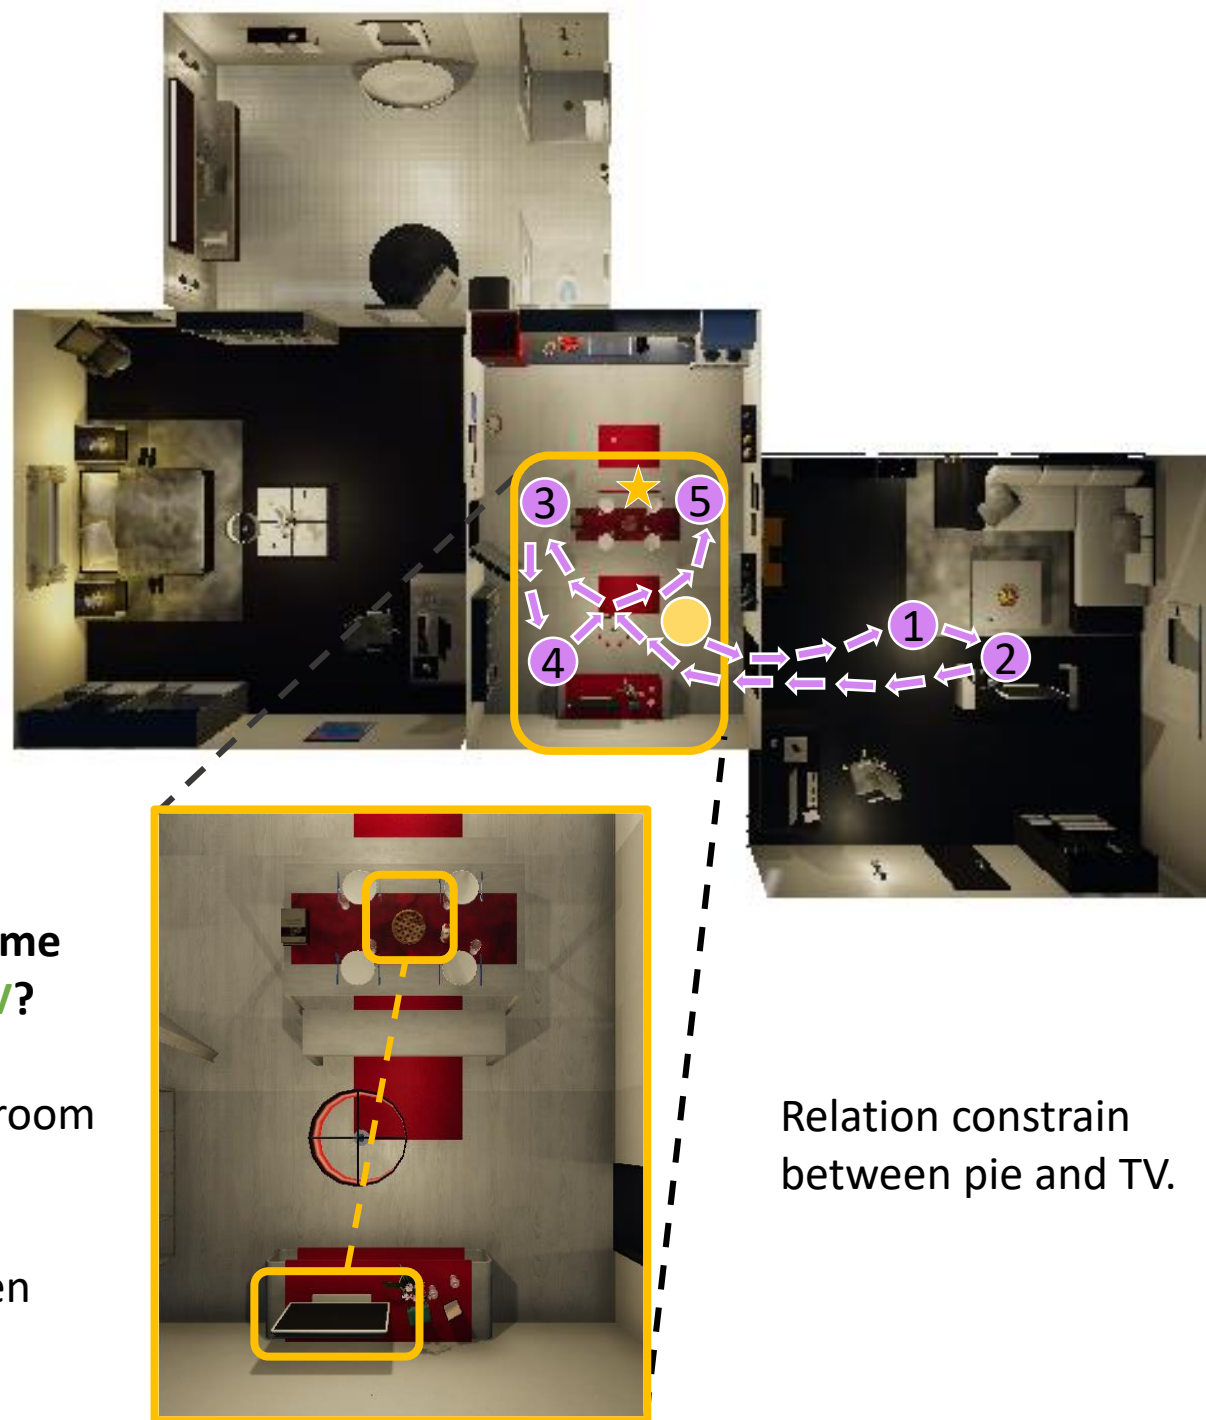

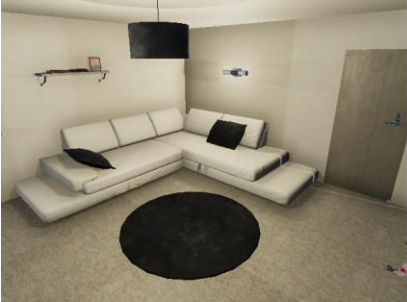

Can you locate the bookshelf facing the TV?

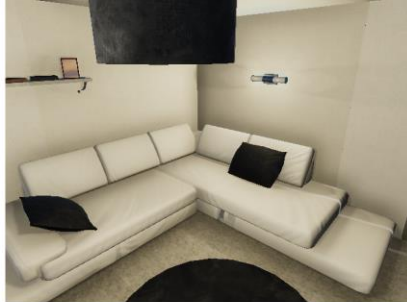

1: Walk to the livingroom

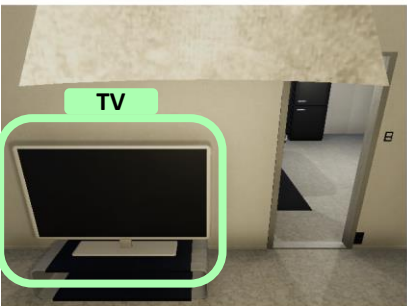

2: Walk to the tv (1)

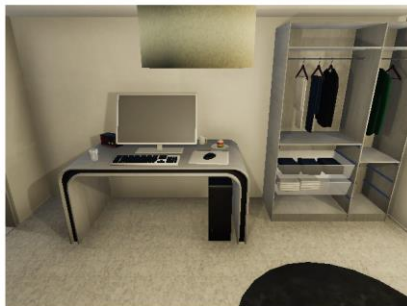

3: Walk to the bedroom

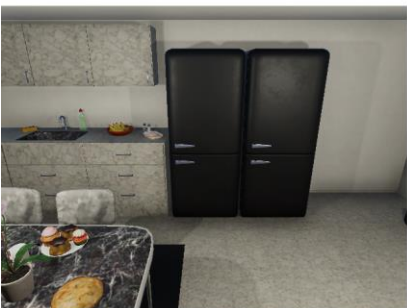

4: Walk to the kitchen

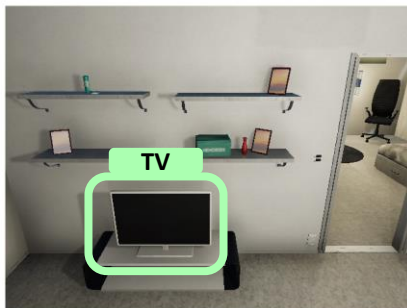

5: Walk to the tv (2)

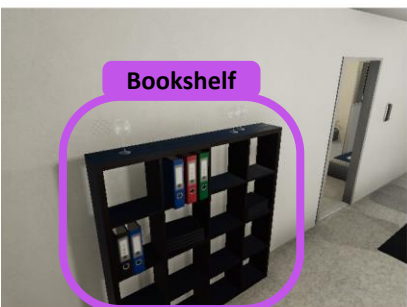

6: Walk to the bookshelf

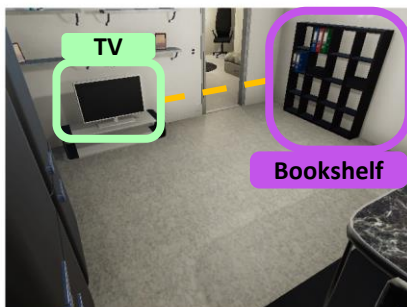

Final state

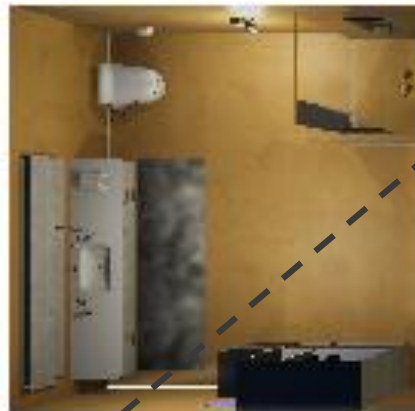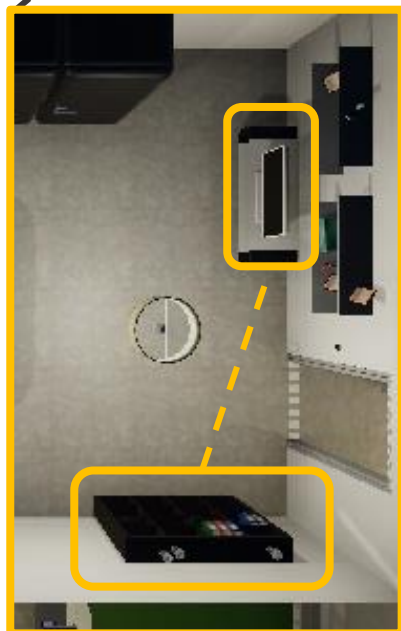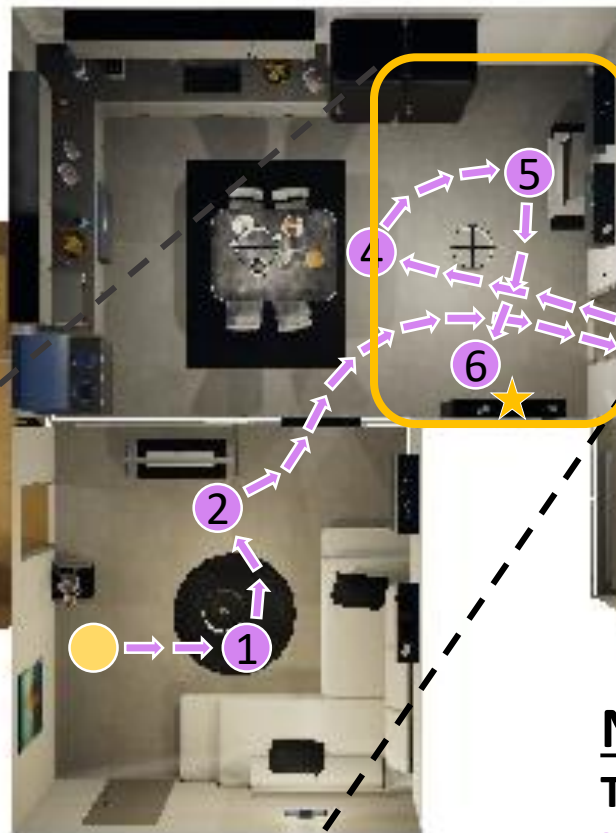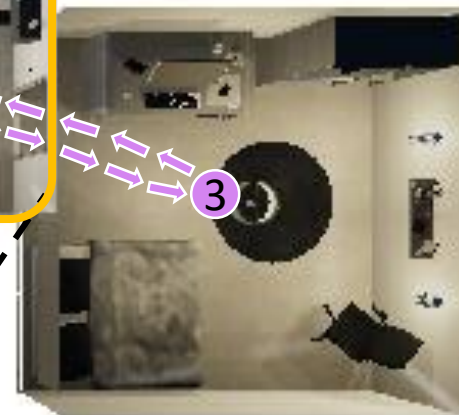

## Navi + Relation

Task: Can you locate the bookshelf facing the TV?

- 1: Walk to the livingroom
- 2: Walk to the tv (1)
- 3: Walk to the bedroom
- 4: Walk to the kitchen
- 5: Walk to the tv (2)
- 6: Walk to the bookshelf

Relation constrain  
between bookshelf  
and TV.

NAVI + RELATION  
FAILURE

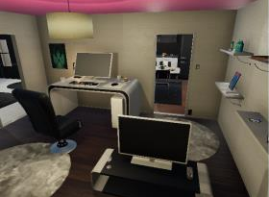

Can you bring me the deodorant close to the toothpaste?

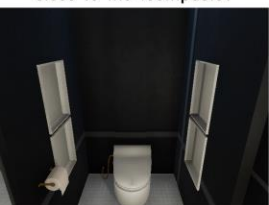

3: Walk to the toilet

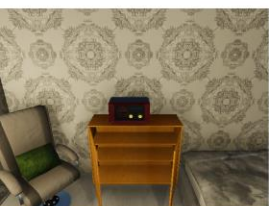

6: Open the cabinet

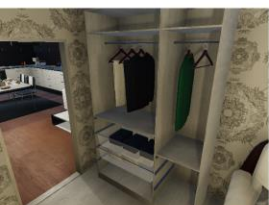

9: Walk to the closet drawer (2)

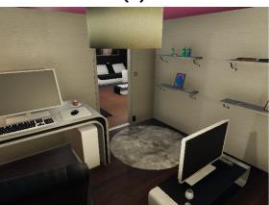

12: Walk to the livingroom

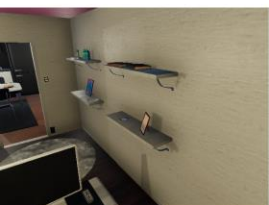

15: Walk to the wall shelf (3)

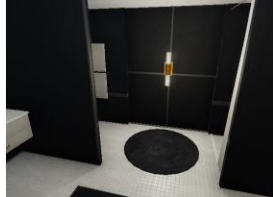

1: Walk to the bathroom

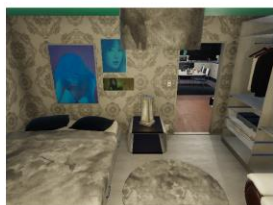

4: Walk to the bedroom

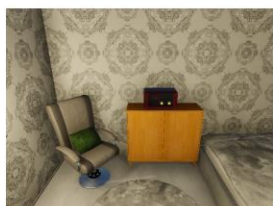

7: Close the cabinet

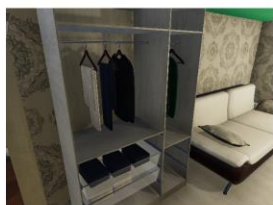

10: Walk to the closet

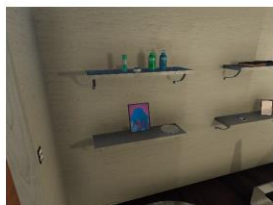

13: Walk to the wall shelf (1)

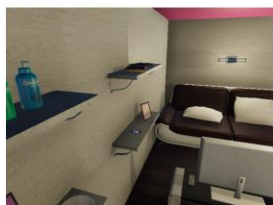

16: Walk to the wall shelf (4)

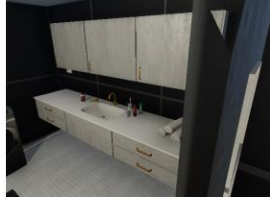

2: Walk to the deodorant

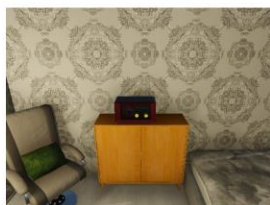

5: Walk to the cabinet (1)

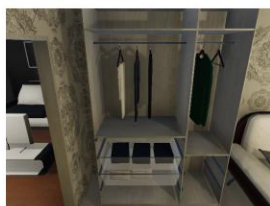

8: Walk to the closet drawer (1)

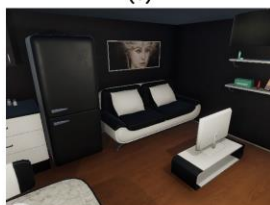

11: Walk to the kitchen

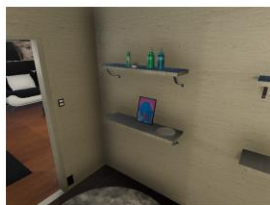

14: Walk to the wall shelf (2)

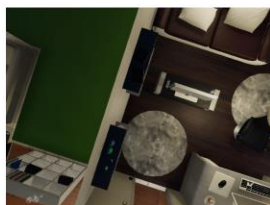

Final state

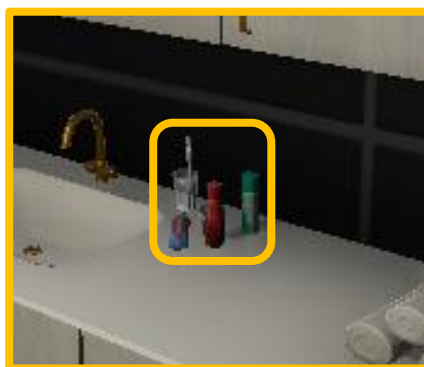

The objects in the counter obstruct the visibility and relations between them.

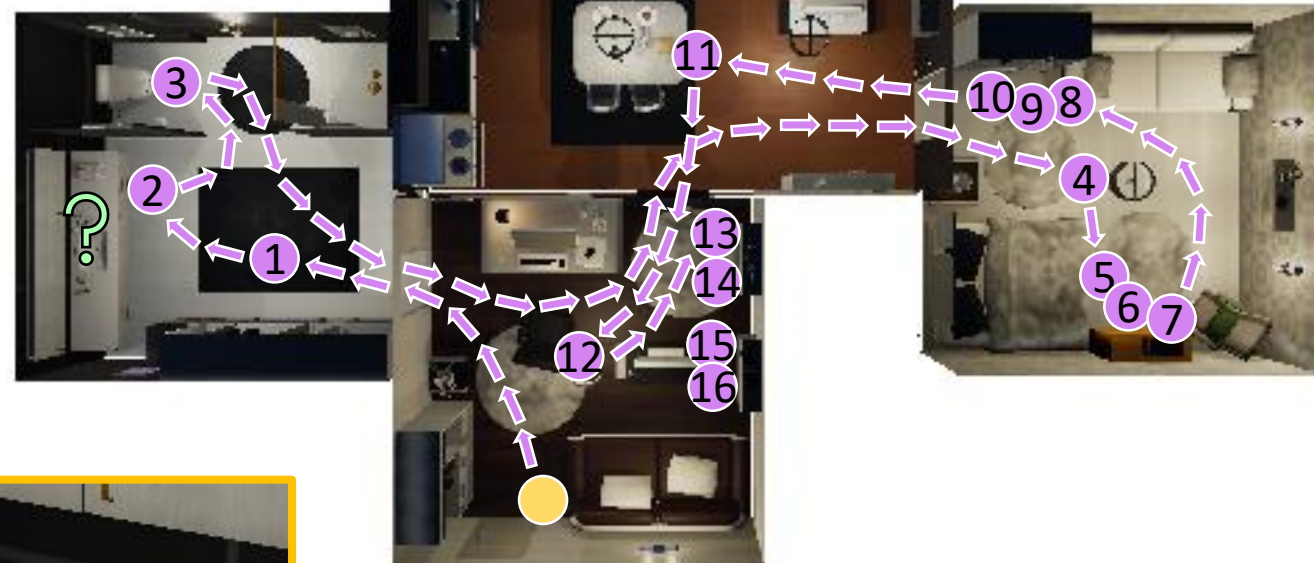

## Navi + Relation

Task: Can you bring me the **deodorant** close to the **toothpaste**?

- 1: Walk to the bathroom
- 2: Walk to the **deodorant**
- 3: Walk to the toilet
- 4: Walk to the bedroom
- 5: Walk to the cabinet (1)

- 6: Open the cabinet
- 7: Close the cabinet
- 8: Walk to the closet drawer (1)
- 9: Walk to the closet drawer (2)
- 10: Walk to the closet
- 11: Walk to the kitchen
- 12: Walk to the livingroom
- 13: Walk to the wall shelf (1)
- 14: Walk to the wall shelf (2)
- 15: Walk to the wall shelf (3)
- 16: Walk to the wall shelf (4)

NAVI/NAVI MANIPULATION  
OCCLUSION SIZE SUCCESS

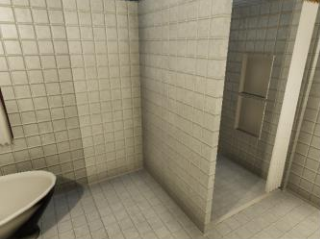

Can you locate the condiment shaker inside the kitchen?

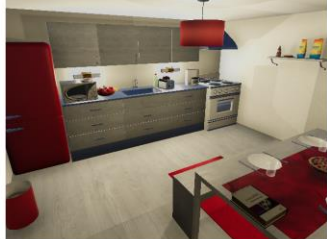

1: Walk to the kitchen

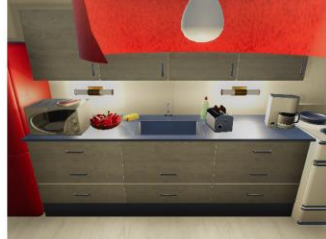

2: Walk to the kitchen counter (1)

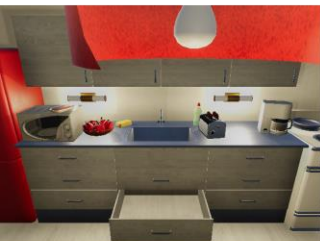

3: Open the kitchen counter

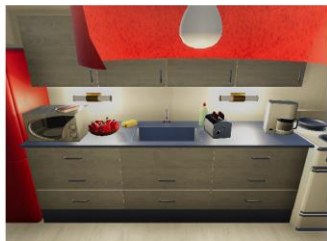

4: Close the kitchen counter

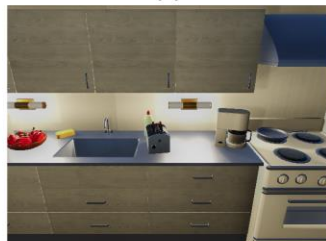

5: Walk to the kitchen cabinet (1)

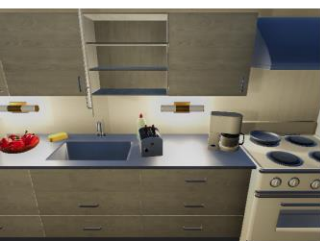

6: Open the kitchen cabinet

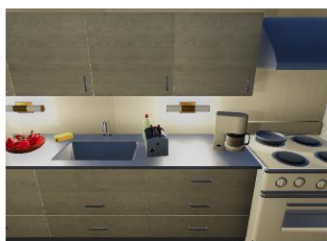

7: Close the kitchen cabinet

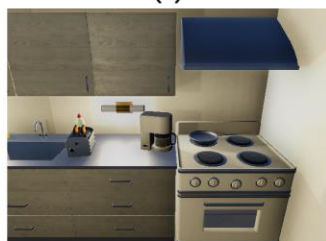

8: Walk to the kitchen cabinet (2)

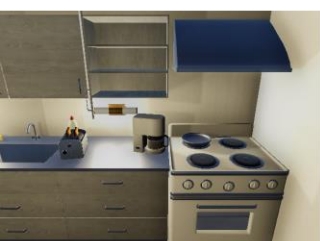

9: Open the kitchen cabinet

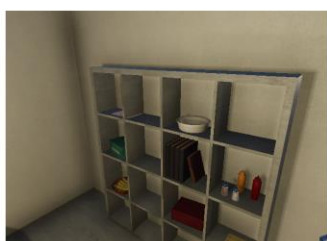

10: Walk to the bookshelf

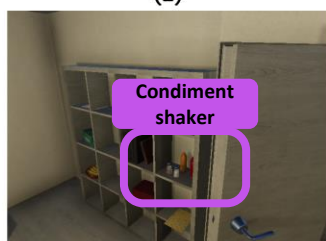

11: Walk to the condimentshaker

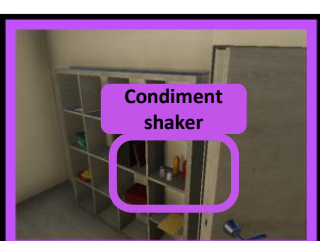

Detected object

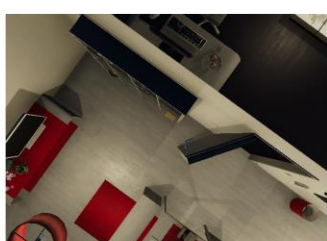

Final state

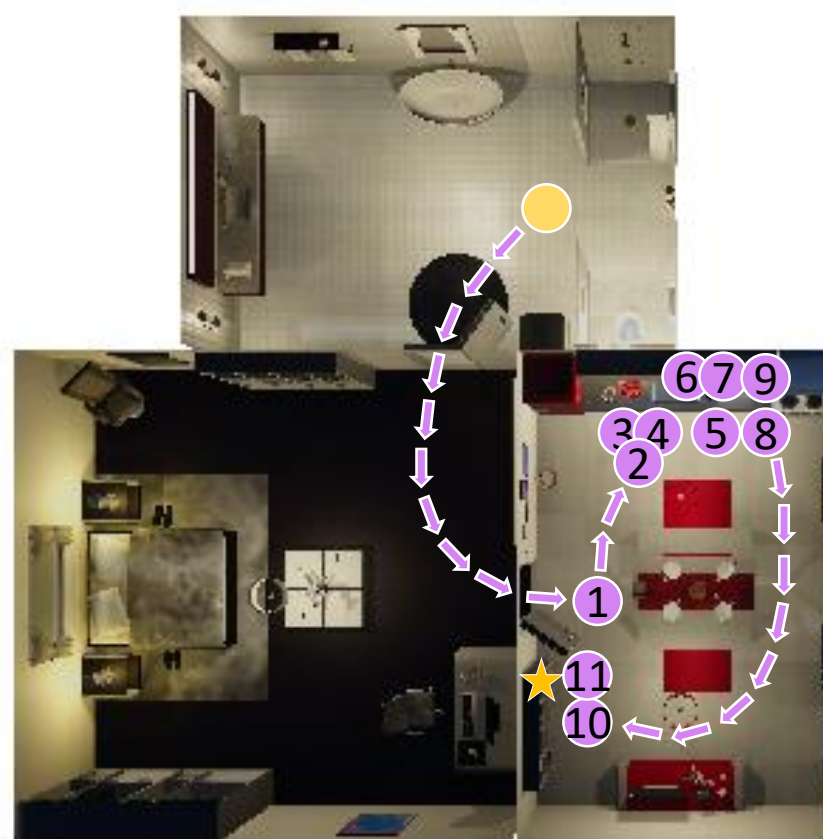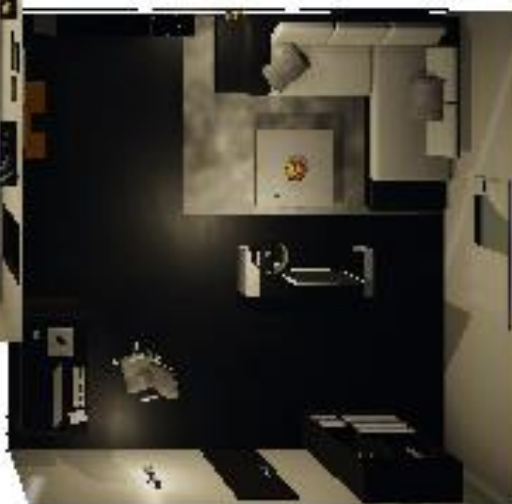

## Navi + Relation + Occlusion size

Task: Can you locate the **condiment shaker** inside the **kitchen**?

- 1: Walk to the **kitchen**
- 2: Walk to the kitchen counter (1)
- 3: Open the kitchen counter
- 4: Close the kitchen counter
- 5: Walk to the kitchen cabinet (1)

- 6: Open the kitchen cabinet
- 7: Close the kitchen cabinet
- 8: Walk to the kitchen cabinet (2)
- 9: Open the kitchen cabinet
- 10: Walk to the bookshelf
- 11: Walk to the **condiment shaker**

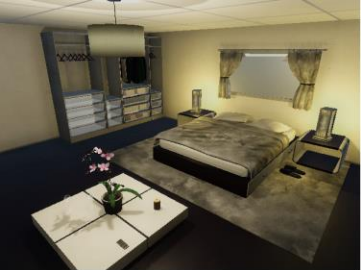

Can you bring me the toothbrush from inside the bathroom?

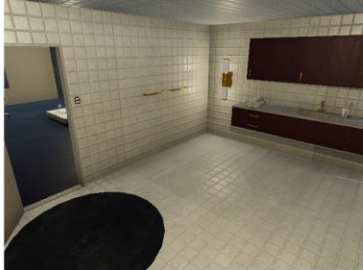

1: Walk to the bathroom

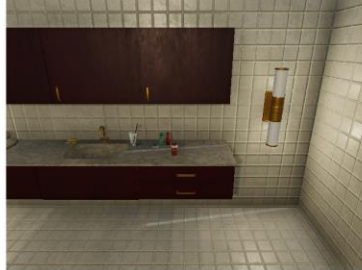

2: Walk to the bathroom counter (1)

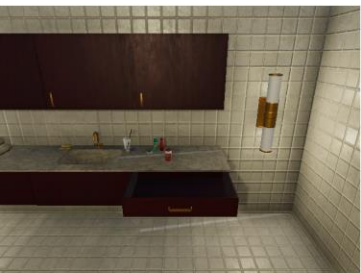

3: Open the bathroom counter

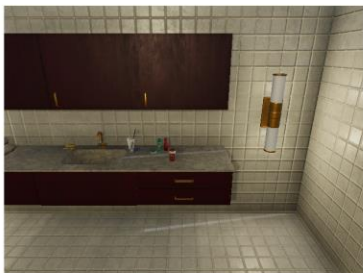

4: Close the bathroom counter

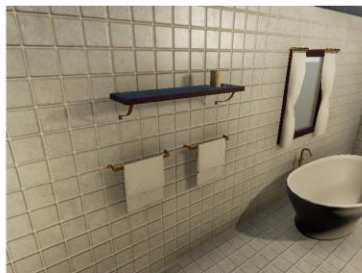

5: Walk to the wall shelf (1)

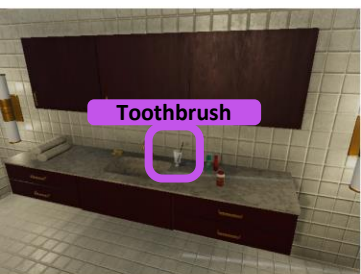

6: Walk to the toothbrush

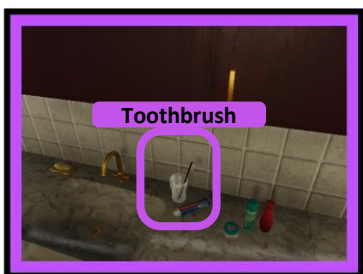

Detected object

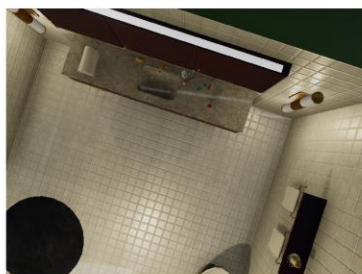

Final state

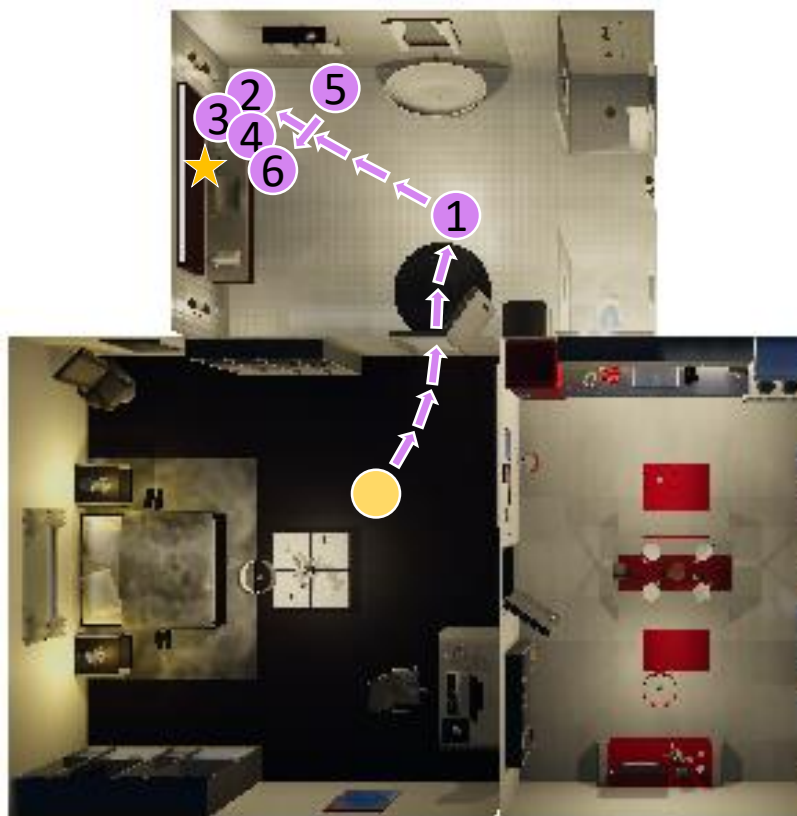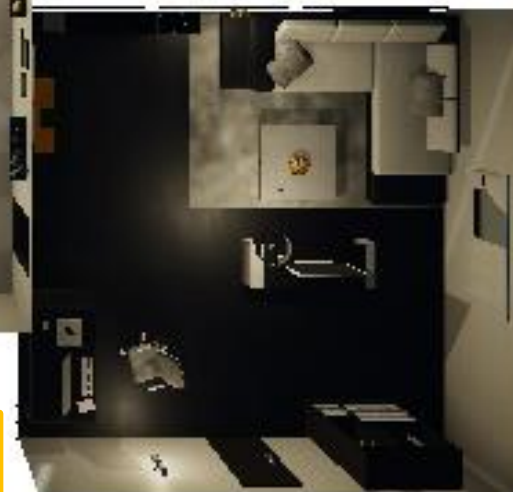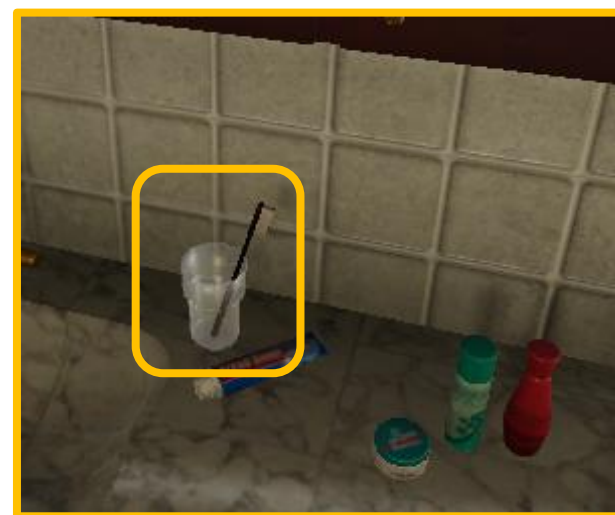

Toothbrush is semi-obstructed by the glass.

## Navi + Relation + Occlusion size

Task: Can you bring me the **toothbrush** from inside the **bathroom**

1: Walk to the **bathroom**  
2: Walk to the bathroom counter (1)

3: Open the bathroom counter  
4: Close the bathroom counter  
5: Walk to the wall shelf (1)  
6: Walk to the **toothbrush**

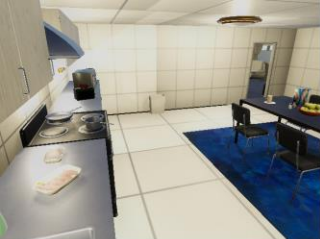

Find the mug and put it inside the fridge.

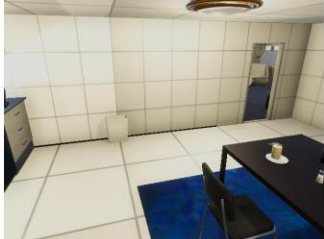

1: Walk to the kitchen

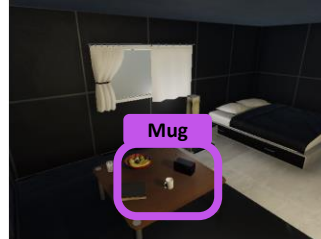

2: Walk to the mug

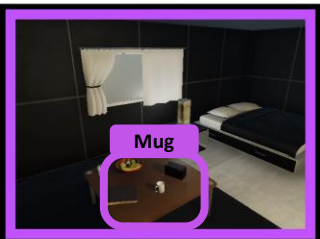

3: Grab the mug

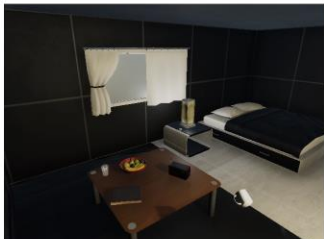

3: Grab the mug

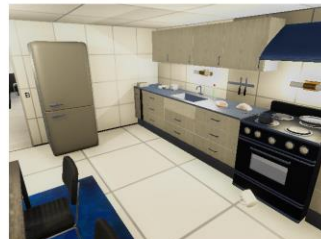

4: Walk to the kitchen

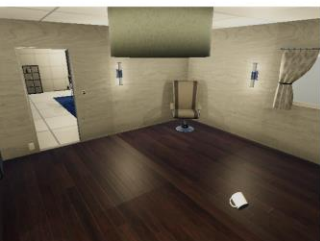

5: Walk to the livingroom

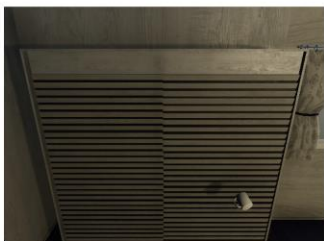

6: Walk to the closet

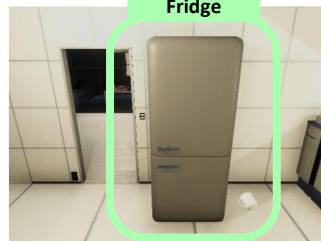

7: Walk to the fridge

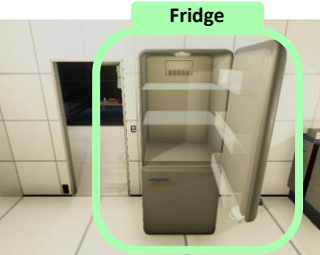

8: Open the fridge

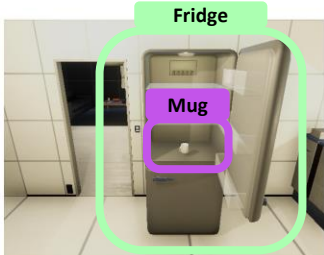

9: Put the mug inside the fridge

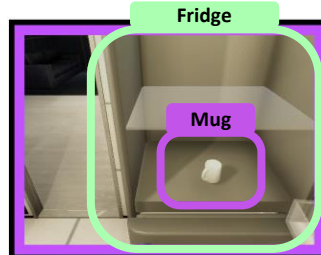

9: Put the mug inside the fridge

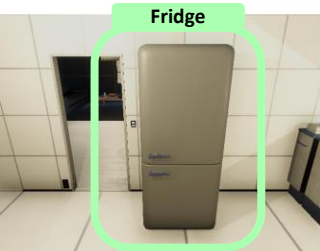

10: Close the fridge

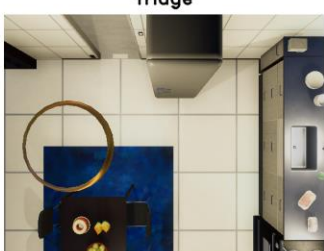

Final state

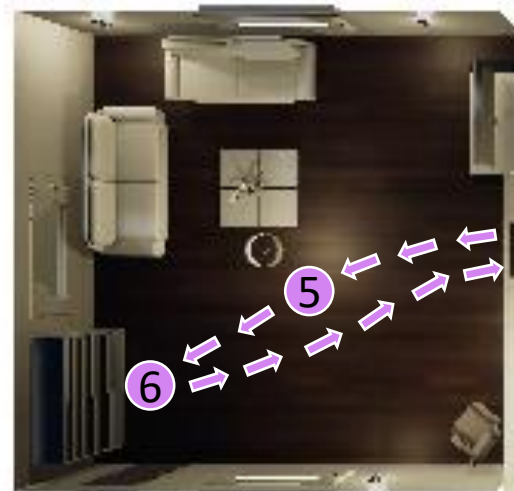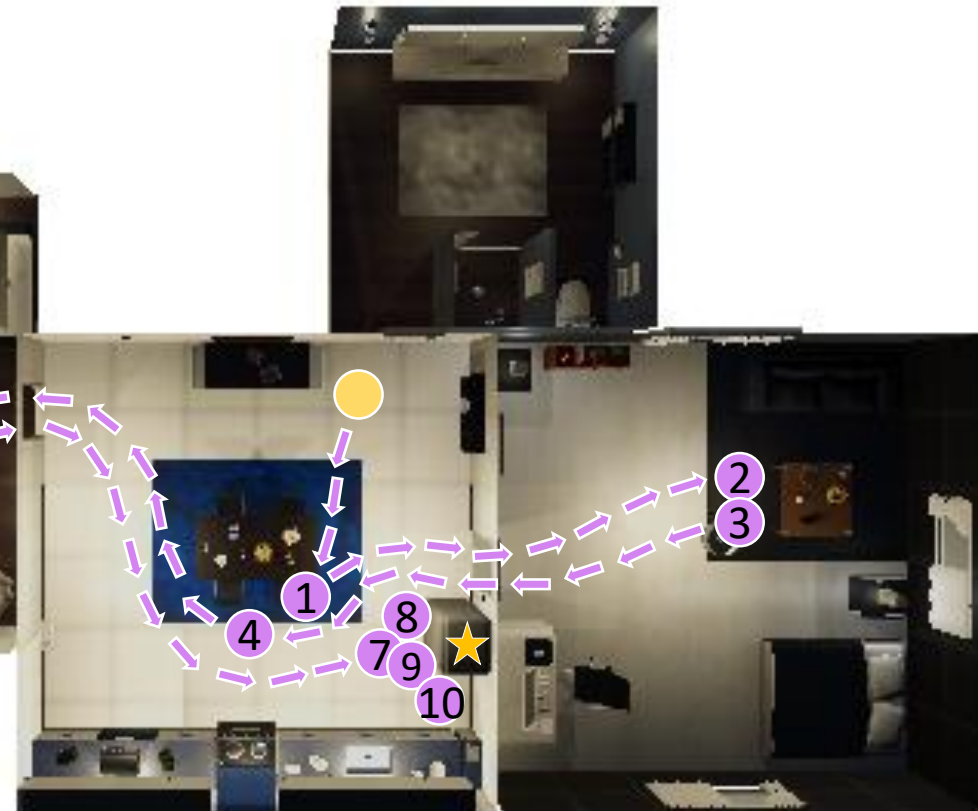

## Navi & Mani + Occlusion size

Task: Find the **mug** and put it inside the **fridge**.

- 1: Walk to the kitchen
- 2: Walk to the **mug**
- 3: Grab the **mug**
- 4: Walk to the kitchen
- 5: Walk to the livingroom

- 6: Walk to the closet
- 7: Walk to the **fridge**
- 8: Open the **fridge**
- 9: Put the **mug** inside the **fridge**
- 10: Close the **fridge**

NAVI + OCCLUSION SIZE  
FAILURE

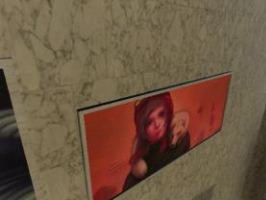

Can you get a cutlery fork from inside the kitchen?

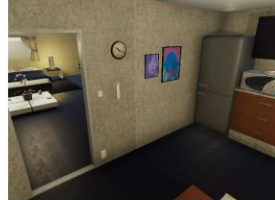

1: Walk to the kitchen

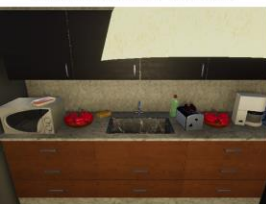

2: Walk to the kitchen cabinet (1)

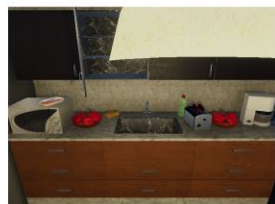

3: Open the kitchen cabinet

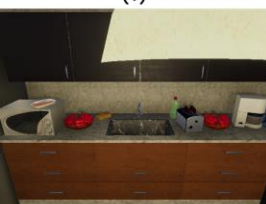

4: Close the kitchen cabinet

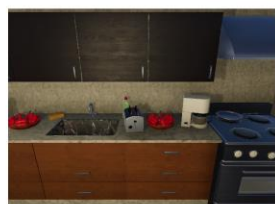

5: Walk to the kitchen cabinet (2)

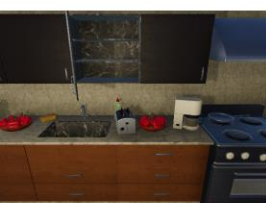

6: Open the kitchen cabinet

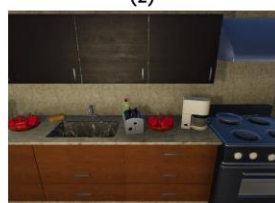

7: Close the kitchen cabinet

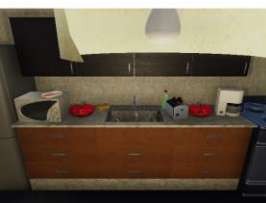

8: Walk to the kitchen counter (1)

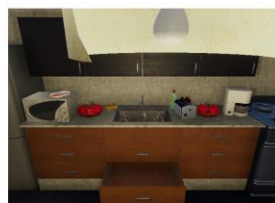

9: Open the kitchen counter

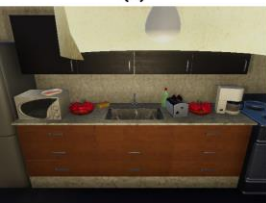

10: Close the kitchen counter

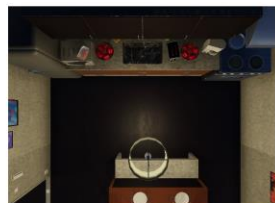

Final state

## Navi + Relation + Occlusion size

Task: Can you get a **cutlery fork** from inside the **kitchen**?

- 1: Walk to the **kitchen**
- 2: Walk to the kitchen cabinet (1)
- 3: Open the kitchen cabinet
- 4: Close the kitchen cabinet

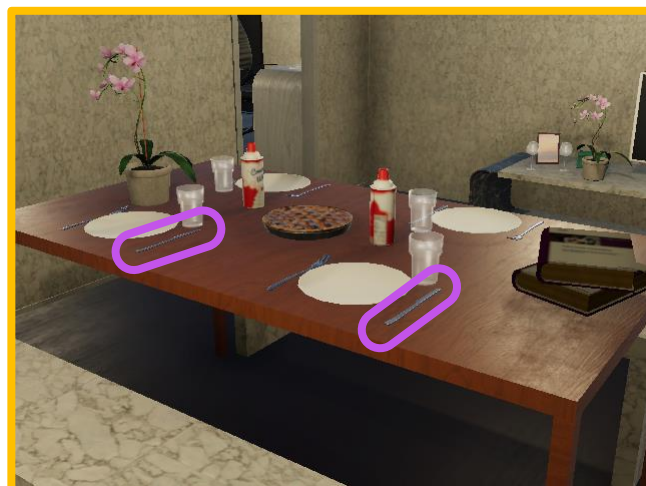

The LLM decides not to explore larger objects like the kitchen table, where the goal object is located.

- 5: Walk to the kitchen cabinet (2)
- 6: Open the kitchen cabinet
- 7: Close the kitchen cabinet
- 8: Walk to the kitchen counter (1)
- 9: Open the kitchen counter
- 10: Close the kitchen counter
- 11: ....

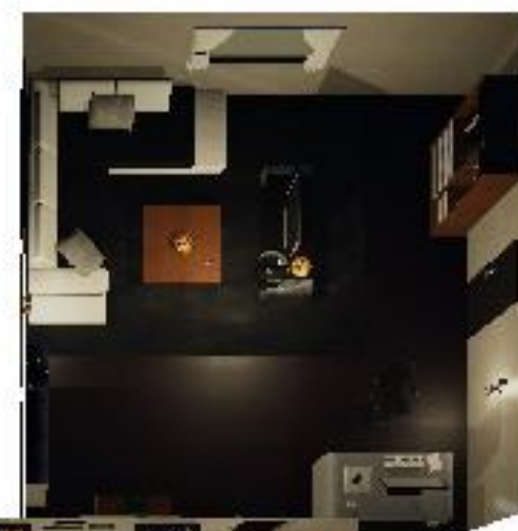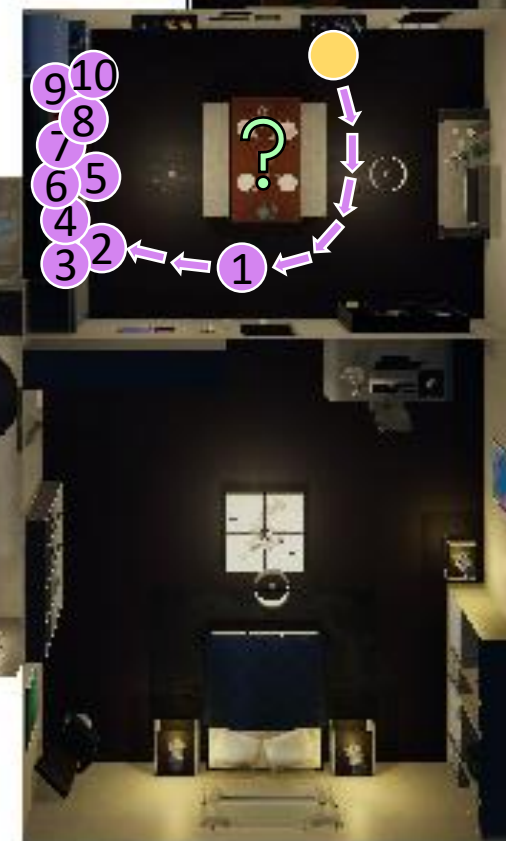

NAVI + OCCLUSION DISTANCE  
SUCCESS

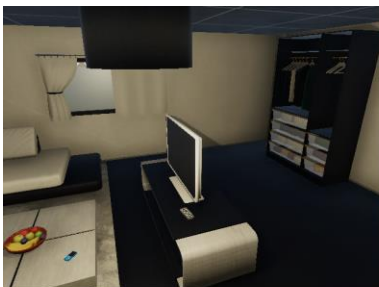

Can you find the candle inside the bedroom?

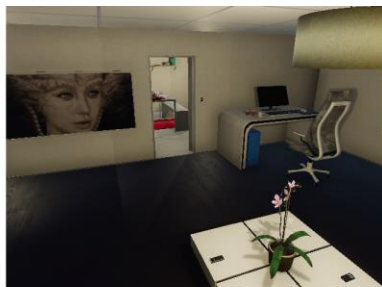

1: Walk to the bedroom

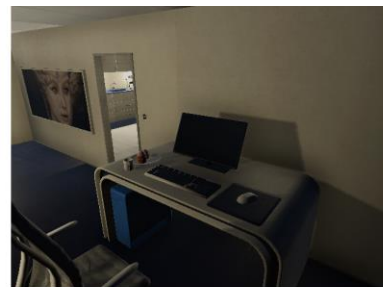

2: Walk to the desk

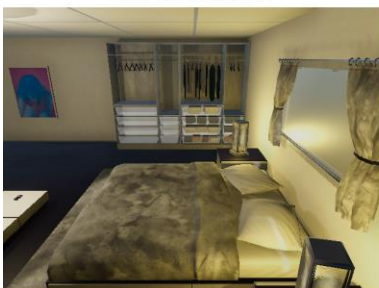

3: Walk to the bed

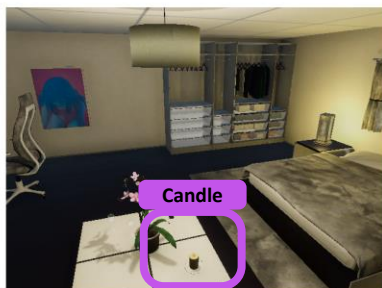

4: Walk to the candle

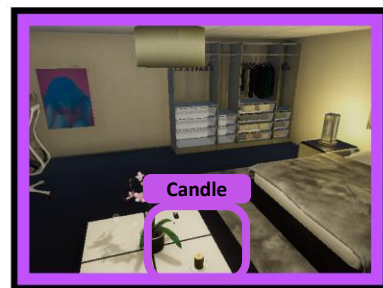

Detected object

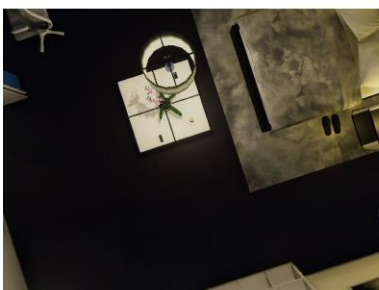

Final state

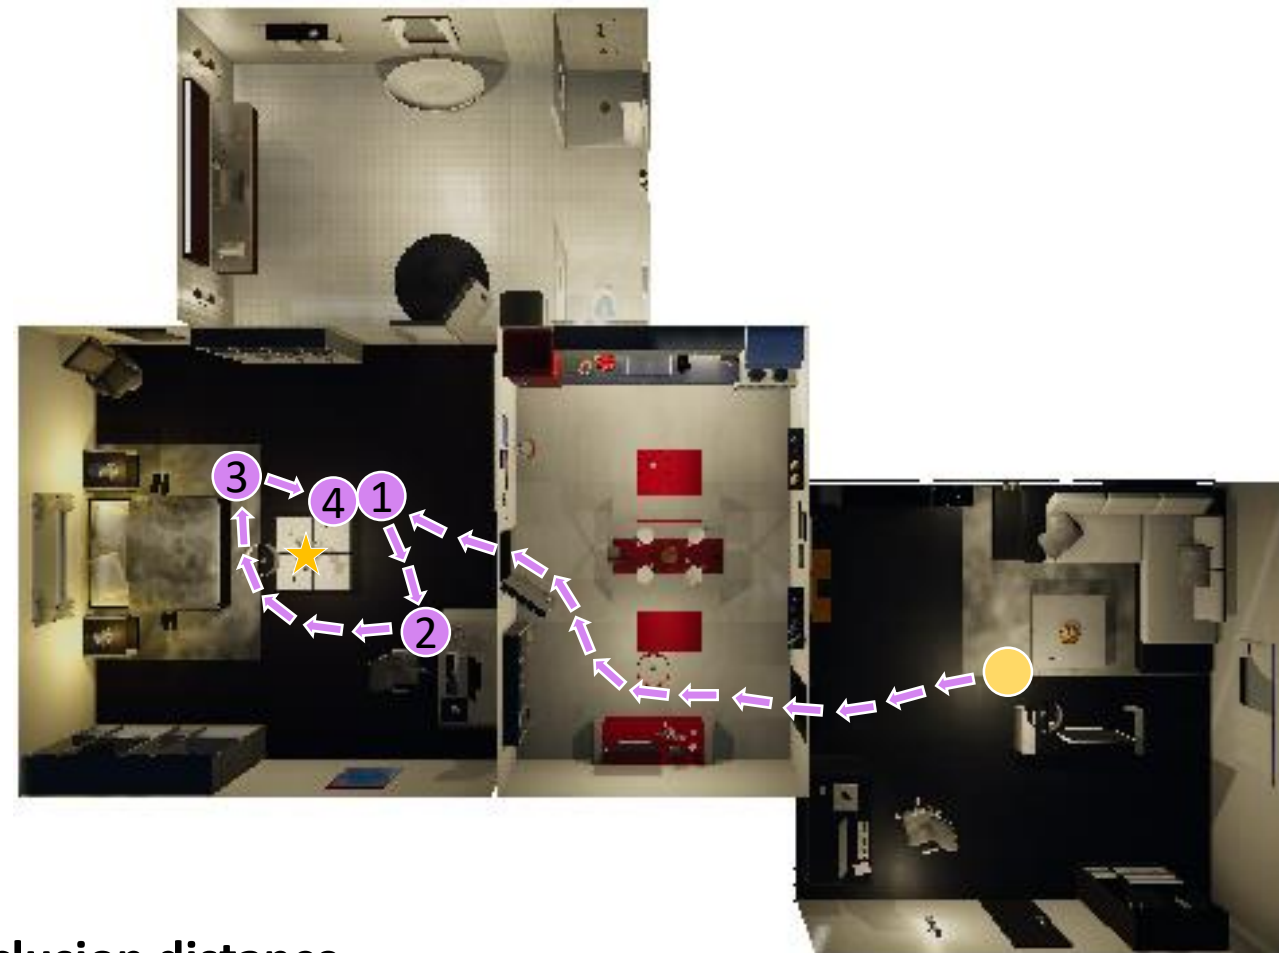

## Navi + Relation + Occlusion distance

Task: Can you find the **candle** inside the **bedroom**?

1: Walk to the **bedroom**

2: Walk to the desk

3: Walk to the bed

4: Walk to the **candle**

NAVI MANIPULATION +  
OCCLUSION DISTANCE  
FAILURE

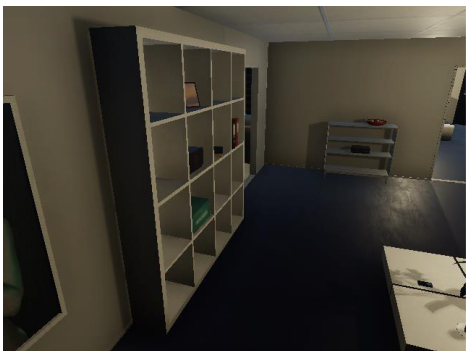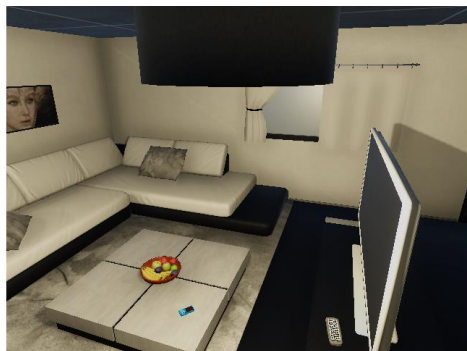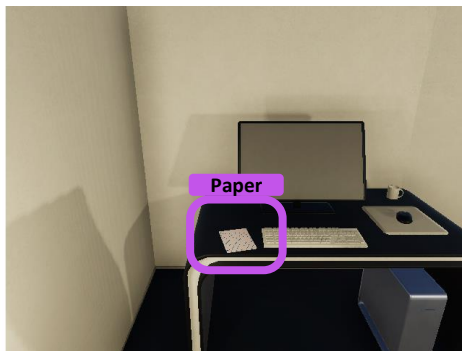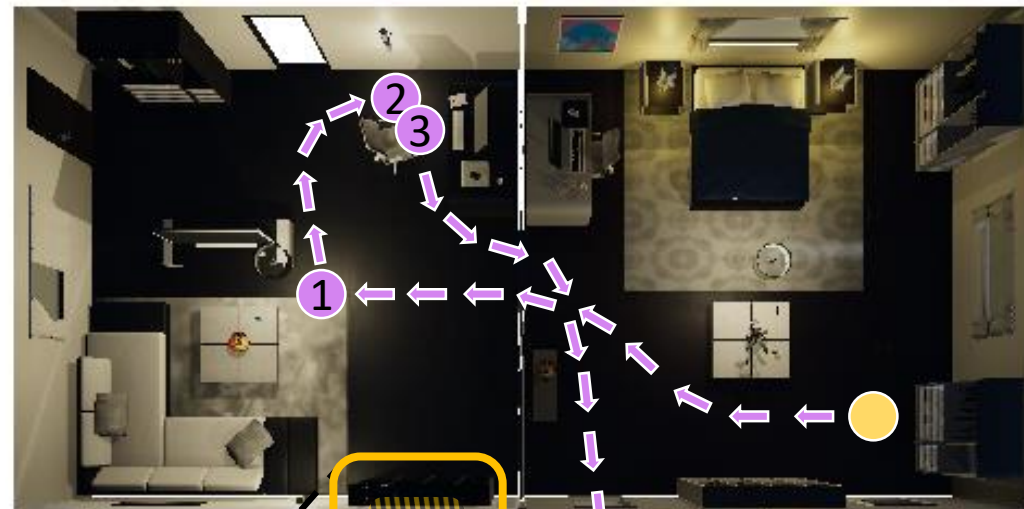

Your task is to get paper inside livingroom and move it to toilet inside bathroom.

1: Walk to the livingroom

2: Walk to the paper

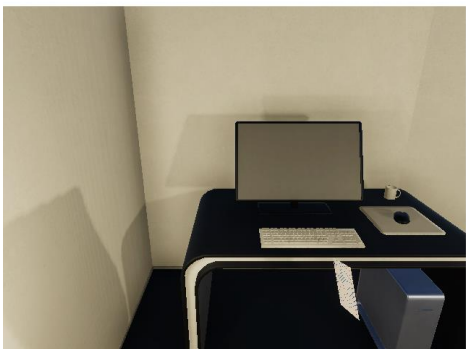

3: Grab the paper

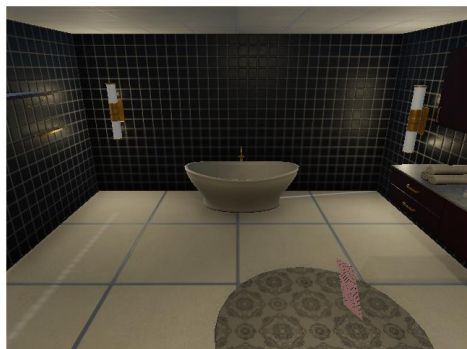

4: Walk to the bathroom

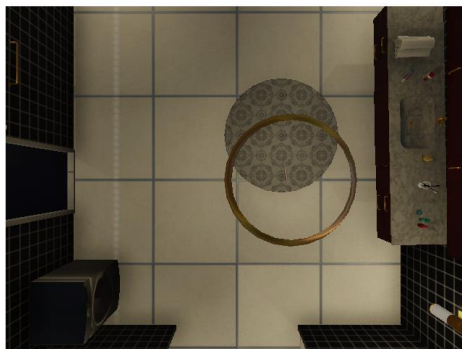

Final state

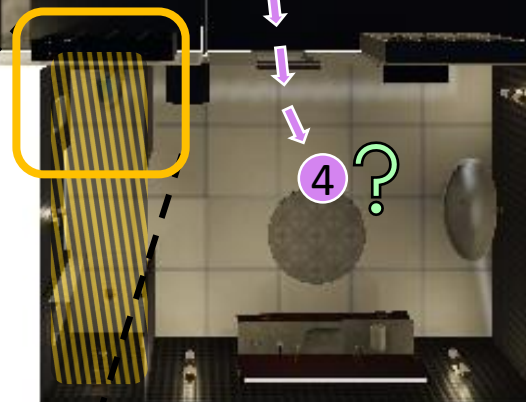

Unexplored area

## Navi & Mani + Relation + Occlusion distance

Your task is to get **paper** inside livingroom and move it to **toilet** inside bathroom.

1: Walk to the livingroom

2: Walk to the **paper**

3: Grab the **paper**

4: Walk to the bathroom

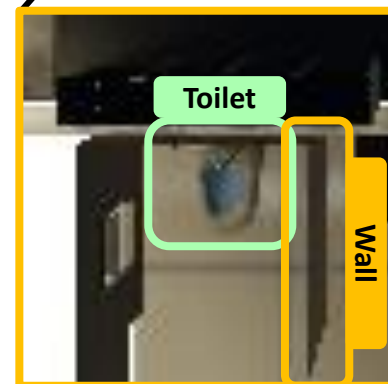

The toilet was blocked by a wall and the LLM decided not to explore near this area.

NAVI AND MANIPULATION +  
MULTIPLE OBJECTS  
SUCCESS

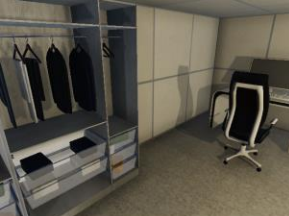

Find a wineglass and a mug, then put them on the kitchen cabinet

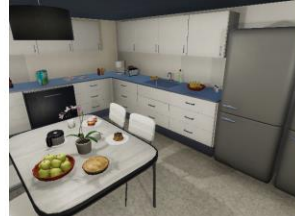

1: Walk to the kitchen

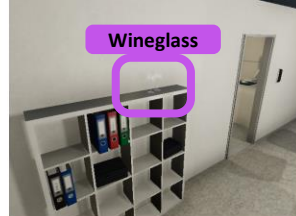

2: Walk to the wineglass

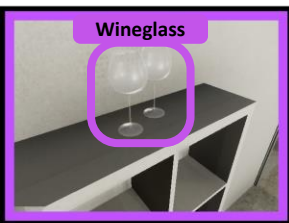

3: Grab the wineglass

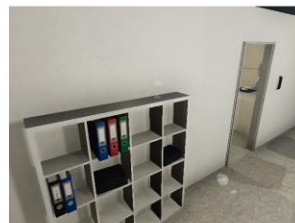

3: Grab the wineglass

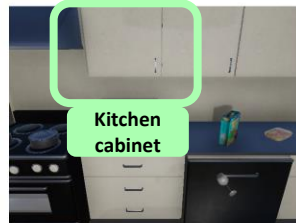

4: Walk to the kitchen cabinet (1)

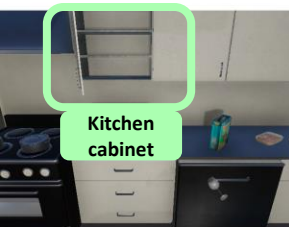

5: Open the kitchen cabinet

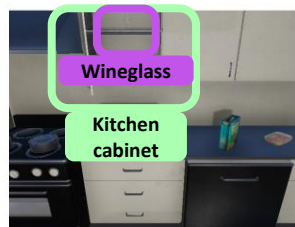

6: Put the wineglass inside the kitchen cabinet

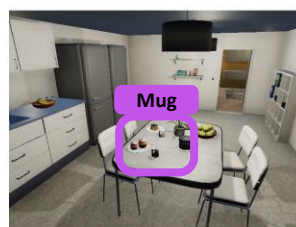

7: Walk to the mug

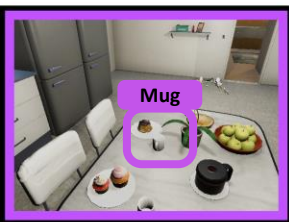

8: Grab the mug

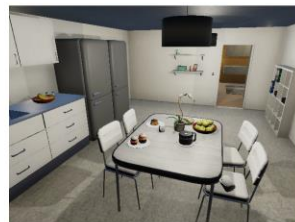

8: Grab the mug

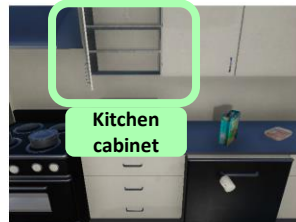

9: Walk to the kitchen cabinet (1)

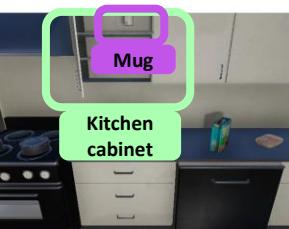

10: Put the mug inside the kitchen cabinet

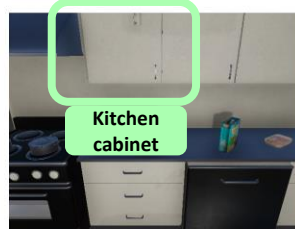

11: Close the kitchen cabinet

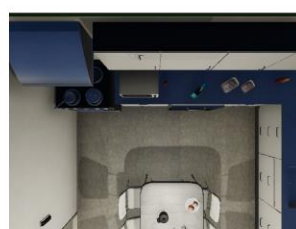

Final state

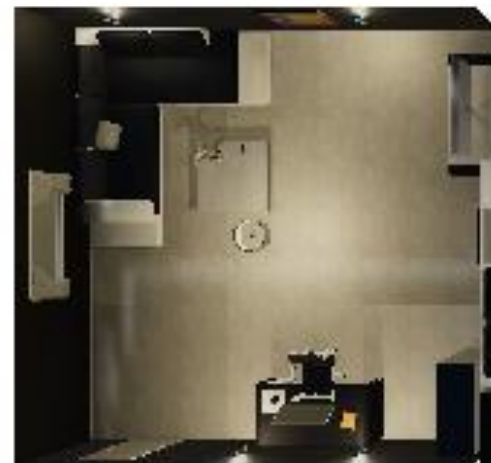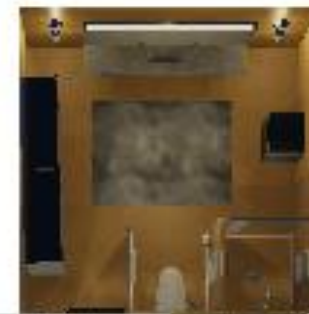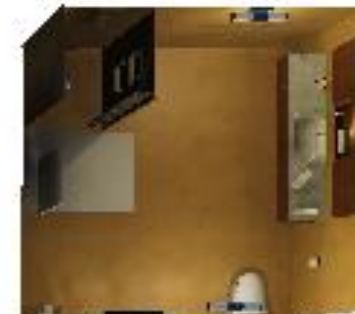

## Navi & Mani w/ Multiple objects

Task: Find a **wineglass** and a **mug**, then put them on the **kitchen cabinet**

1: Walk to the kitchen

2: Walk to the **wineglass**

3: Grab the **wineglass**

4: Walk to the **kitchen cabinet** (1)

5: Open the **kitchen cabinet**

6: Put the wineglass inside the **kitchen cabinet**

7: Walk to the **mug**

8: Grab the **mug**

9: Walk to the **kitchen cabinet** (1)

10: Put the mug inside the **kitchen cabinet**

11: Close the **kitchen cabinet**

NAVI AND MANIPULATION +  
MULTIPLE OBJECTS  
FAILURE

NAVI AND MANIPULATION w/  
multiple objects + OPTIMAL PATH  
SUCCESS

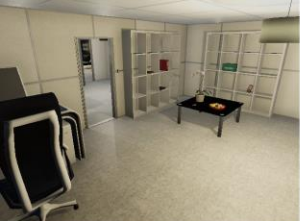

Gather the coffeepot and wineglass and then lay them into the dishwasher.

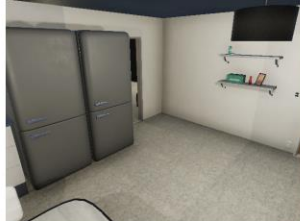

1: Walk to the kitchen

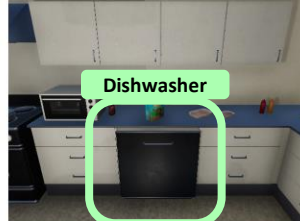

2: Walk to the dishwasher

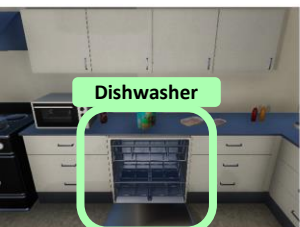

3: Open the dishwasher

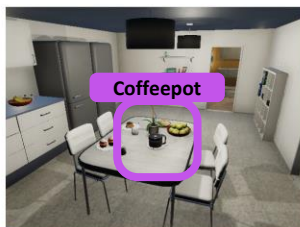

4: Walk to the coffeepot

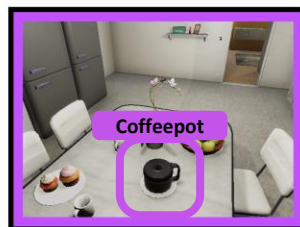

5: Grab the coffeepot

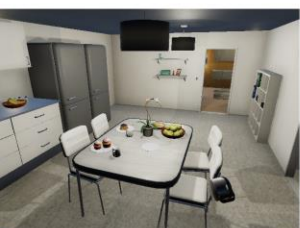

5: Grab the coffeepot

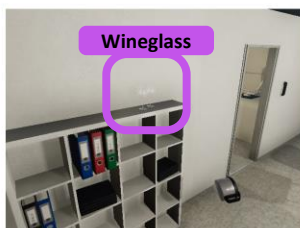

6: Walk to the wineglass

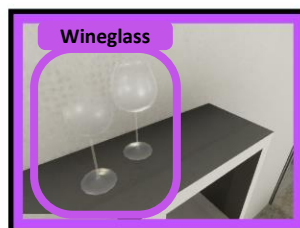

7: Grab the wineglass

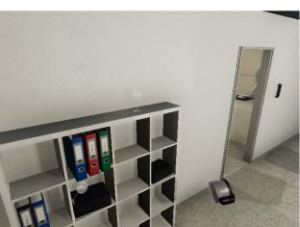

7: Grab the wineglass

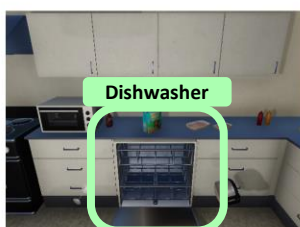

8: Walk to the dishwasher

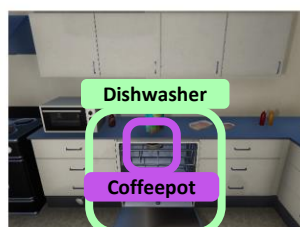

9: Put the coffeepot inside the dishwasher

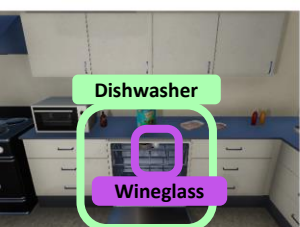

10: Put the wineglass inside the dishwasher

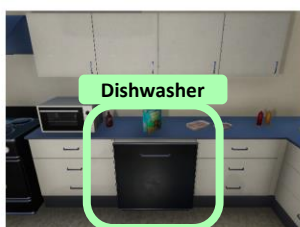

11: Close the dishwasher

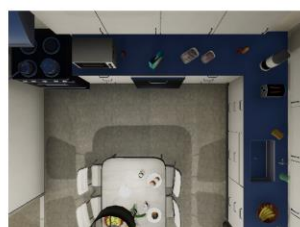

Final state

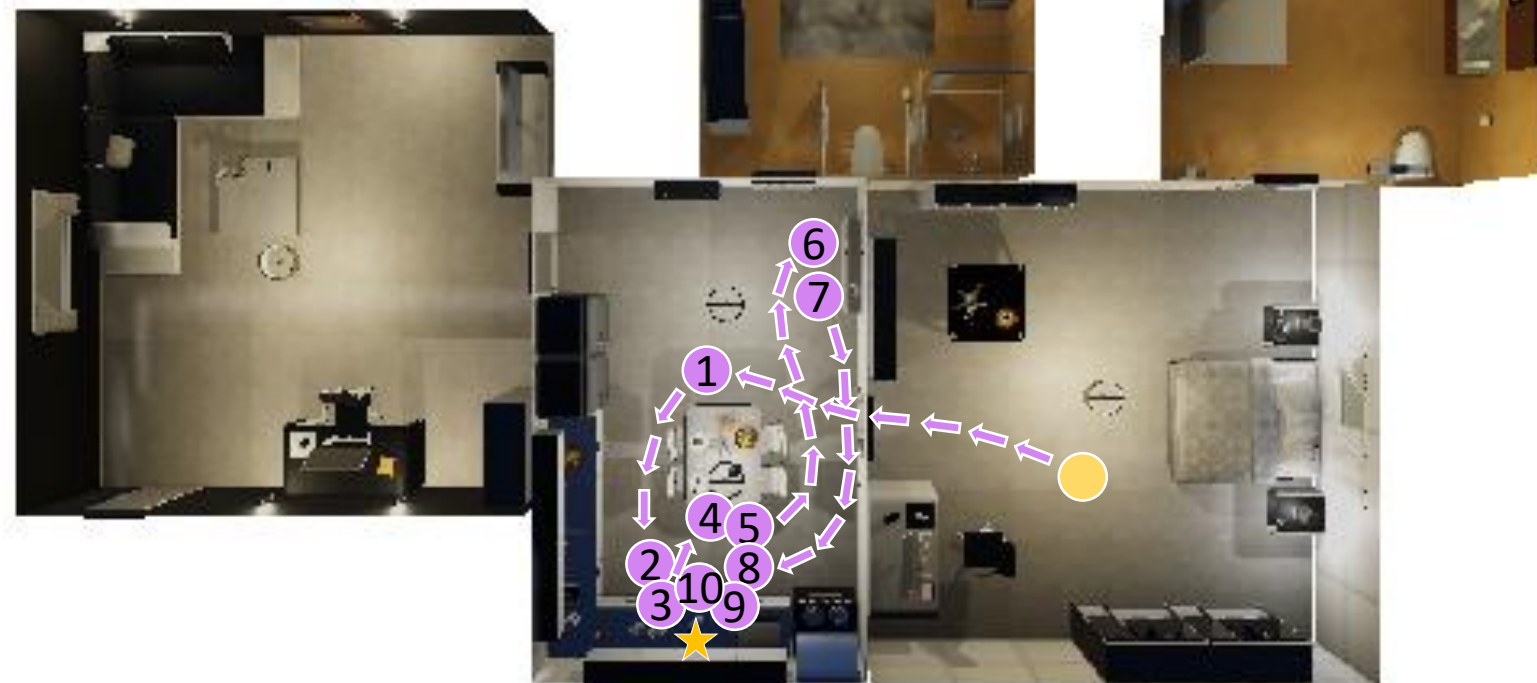

## Navi & Mani w/ Multiple objects

### + Optimal path

Task: Gather the **coffeepot** and **wineglass** and then lay them into the **dishwasher**.

- 1: Walk to the kitchen
- 2: Walk to the **dishwasher**
- 3: Open the **dishwasher**
- 4: Walk to the **coffeepot**

- 5: Grab the **coffeepot**
- 6: Walk to the **wineglass**
- 7: Grab the **wineglass**
- 8: Walk to the **dishwasher**
- 9: Put the **coffeepot** inside the **dishwasher**
- 10: Put the **wineglass** inside the **dishwasher**
- 11: Close the **dishwasher**

NAVI AND MANIPULATION w/  
multiple objects + OPTIMAL PATH  
FAILURE

NAVI AND MANIPULATION +  
TEMPORAL DEPENDENCY  
SUCCESS

NAVI AND MANIPULATION +  
TEMPORAL DEPENDENCY  
FAILURE
