# Supplementary material for: ET-Plan-Bench: Embodied Task-level Planning Benchmark Towards Spatial-Temporal Cognition with Foundation Models
Source: arXiv:2410.14682 source file (2025-02-13)
Supplement: Supplementary file 3 [file success_failure_demos_appendix.pdf]

Navi or Navi & Manipulation

Navi or Navi & Manipulation + relation (pick two relations, something like “face to”, ‘next to’)

Navi or Navi & Manipulation + occlusion size

Navi or Navi & Manipulation + distance

Navi & Manipulation + multiple objects

Navi & Manipulation + optimal path

Navi & Manipulation + temp dependency

| Task                                                  | Success | Failure |
|-------------------------------------------------------|---------|---------|
| Navi                                                  | 1       | 1       |
| Navi & Manipulation                                   | 1       |         |
| Navi + relation                                       | 3       | 1       |
| Navi & Manipulation + relation                        |         |         |
| Navi + occlusion size                                 | 2       | 1       |
| Navi & Manipulation + occlusion size                  | 1       |         |
| Navi + distance                                       | 1       |         |
| Navi & Manipulation + distance                        |         | 1       |
| Navi & Manipulation + multiple objects                | 1       |         |
| Navi & Manipulation + multiple objects + optimal path | 1       |         |
| Navi & Manipulation + temp dependency                 | -----   | -----   |

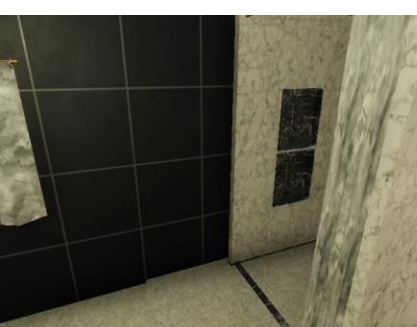

Can you lead me to the desk?

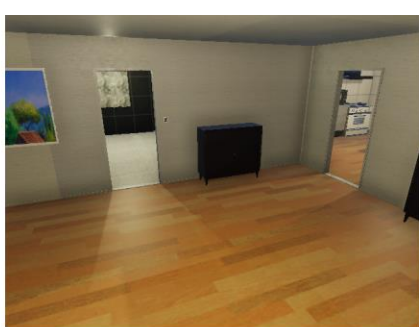

1: Walk to the bedroom

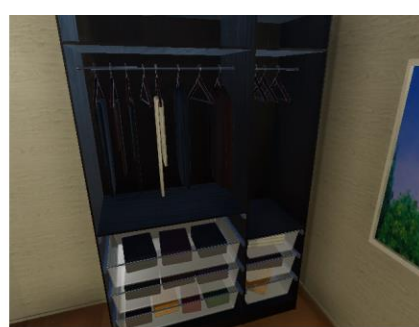

2: Walk to the closet

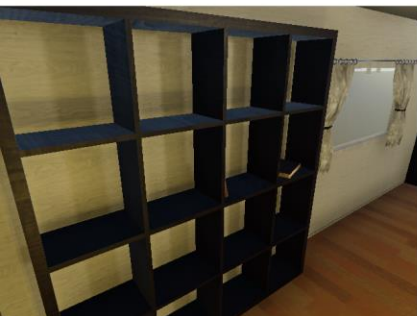

3: Walk to the bookshelf

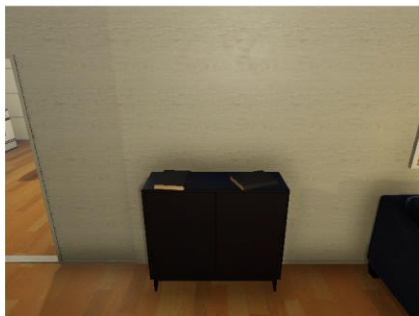

4: Walk to the cabinet (1)

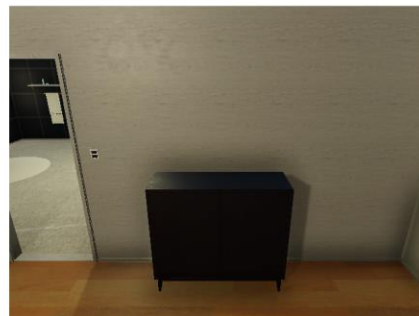

5: Walk to the cabinet (2)

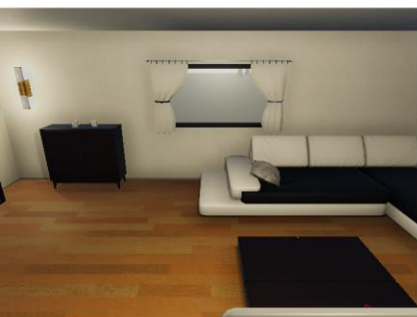

6: Walk to the livingroom

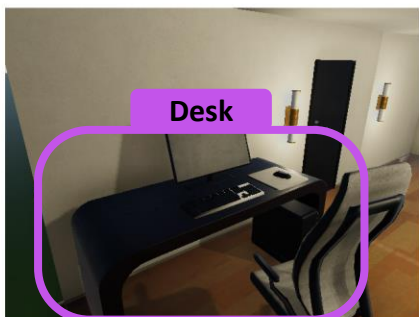

7: Walk to the desk

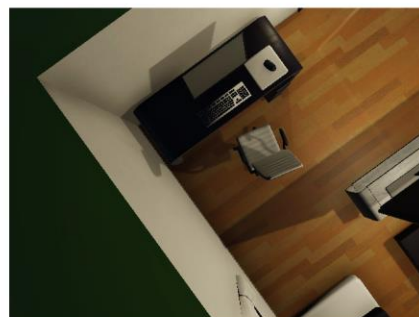

Final state

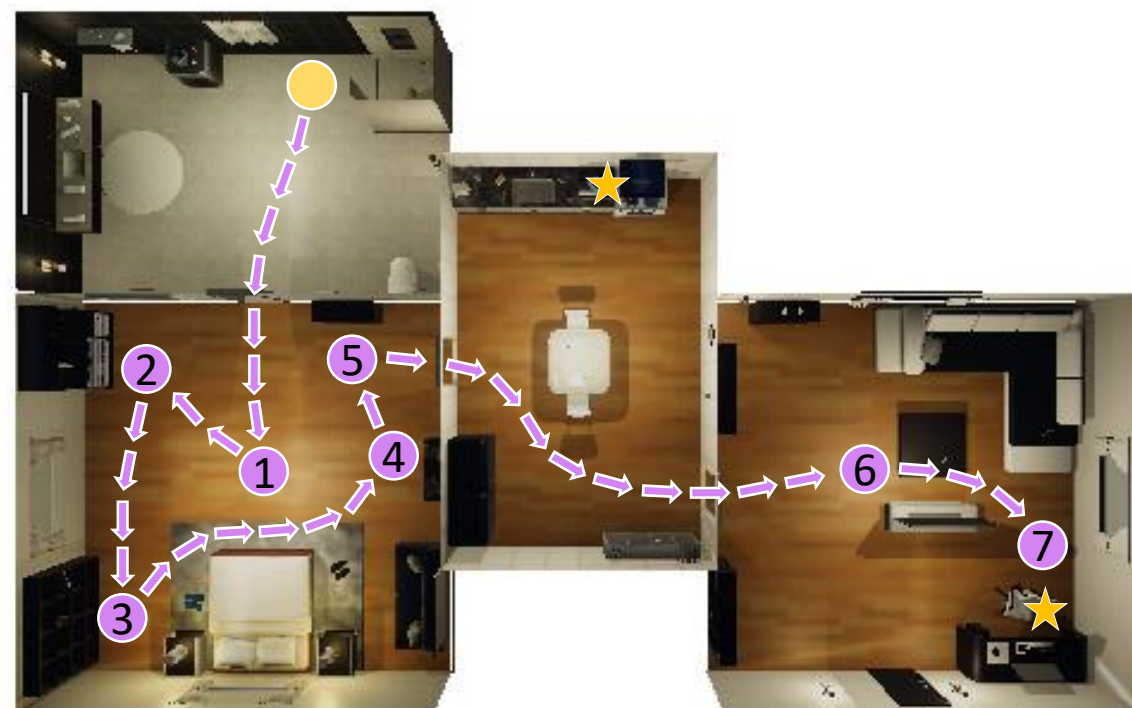

## Navigation

Task: Can you lead me to the **desk**?

- 1: Walk to the bedroom
- 2: Walk to the closet
- 3: Walk to the bookshelf

- 4: Walk to the cabinet (1)
- 5: Walk to the cabinet (2)
- 6: Walk to the livingroom
- 7: Walk to the **desk**

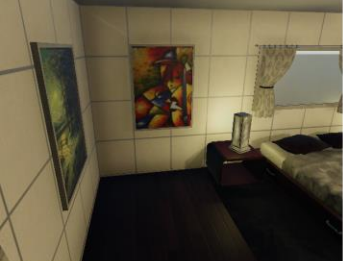

Please place the cutlets on the kitchen table.

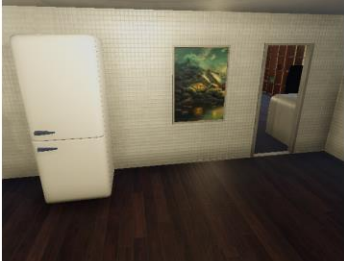

1: Walk to the kitchen

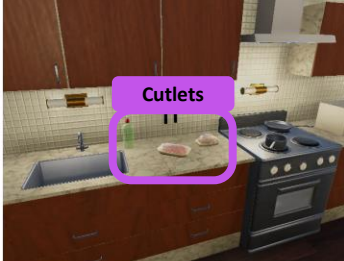

2: Walk to the cutlets

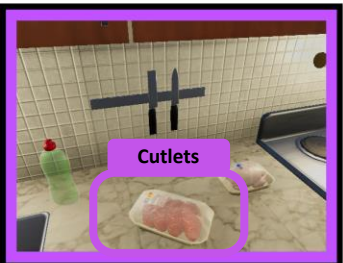

3: Grab the cutlets

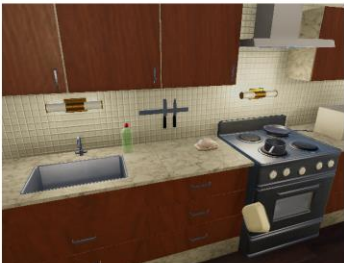

3: Grab the cutlets

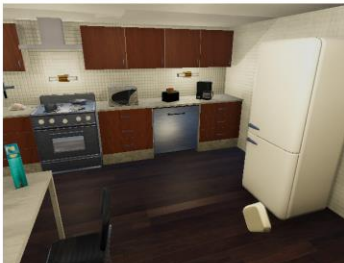

4: Walk to the kitchen

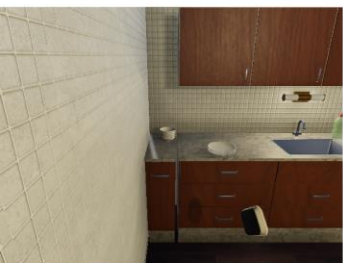

5: Walk to the kitchen counter (1)

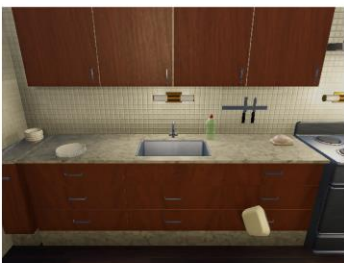

6: Walk to the kitchen counter (2)

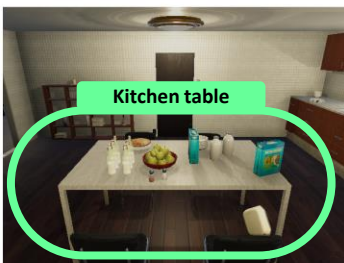

7: Walk to the kitchentable

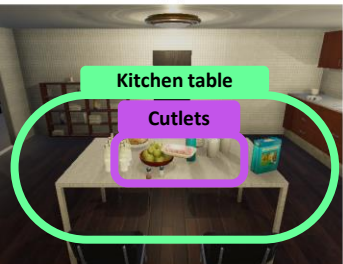

8: Put the cutlets in the kitchentable

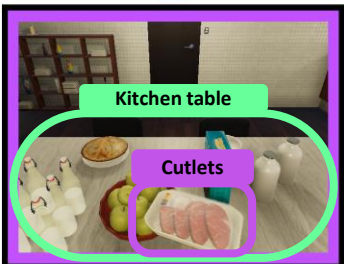

8: Put the cutlets in the kitchentable

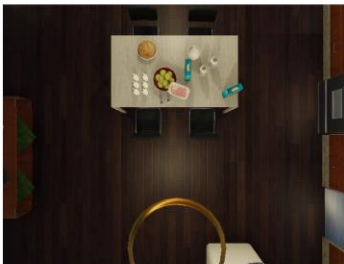

Final state

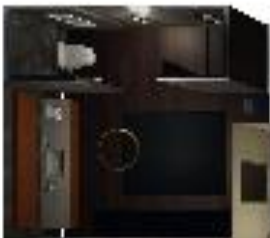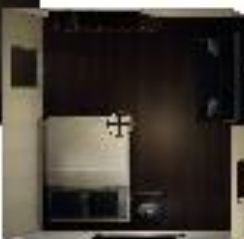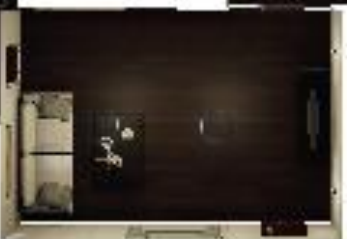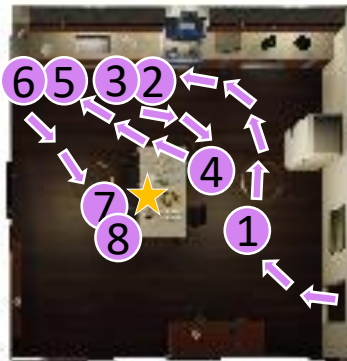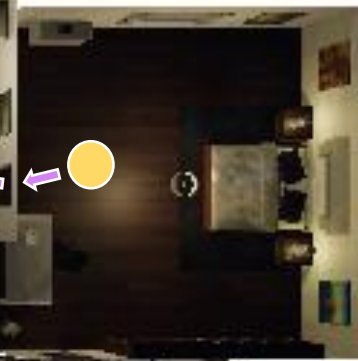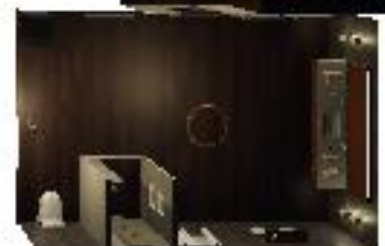

# Navi & Mani

Task: Please place the cutlets on the kitchen table.

- 1: Walk to the kitchen
- 2: Walk to the cutlets
- 3: Grab the cutlets
- 4: Walk to the kitchen

- 5: Walk to the kitchen counter (1)
- 6: Walk to the kitchen counter (2)
- 7: Walk to the kitchen table
- 8: Put the cutlets in the kitchen table



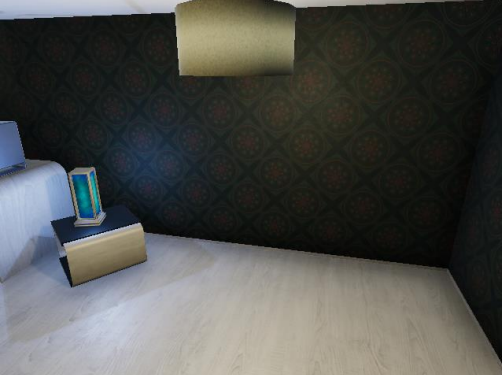

Can you show me where the bench is?

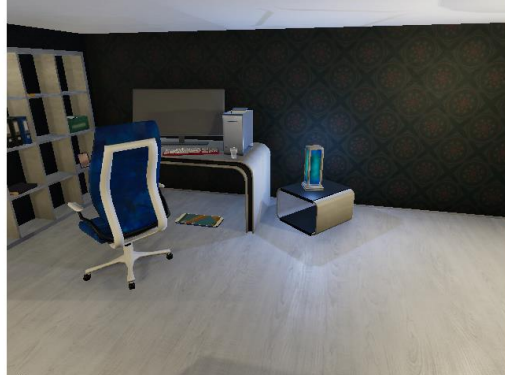

1: Walk to the livingroom

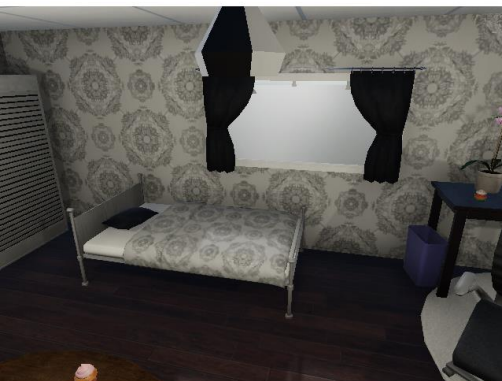

2: Walk to the bedroom

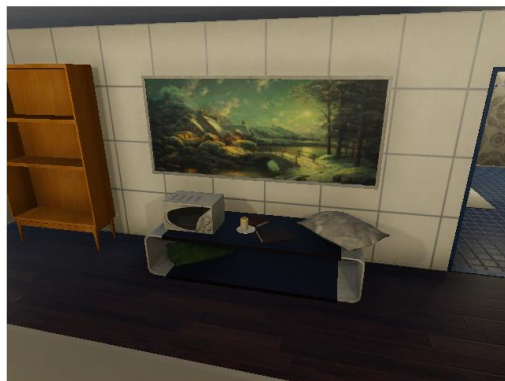

3: Walk to the kitchen

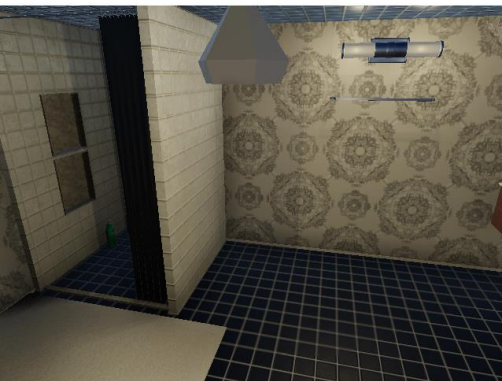

4: Walk to the bathroom

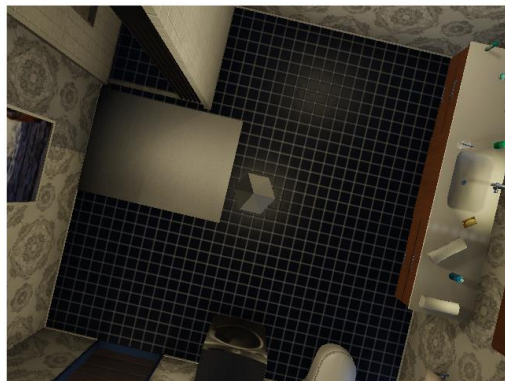

Final state

# Navigation

Task: Can you show me where the bench is?

- 1: Walk to the livingroom
- 2: Walk to the bedroom
- 3: Walk to the kitchen
- 4: Walk to the bathroom

*The LLM decided not to explore any of the rooms other than the initial observation.*

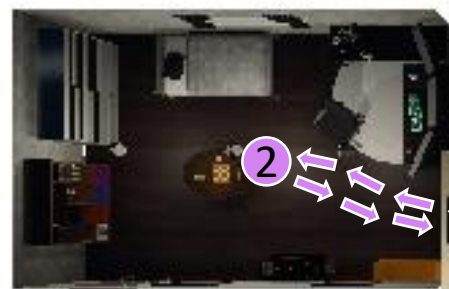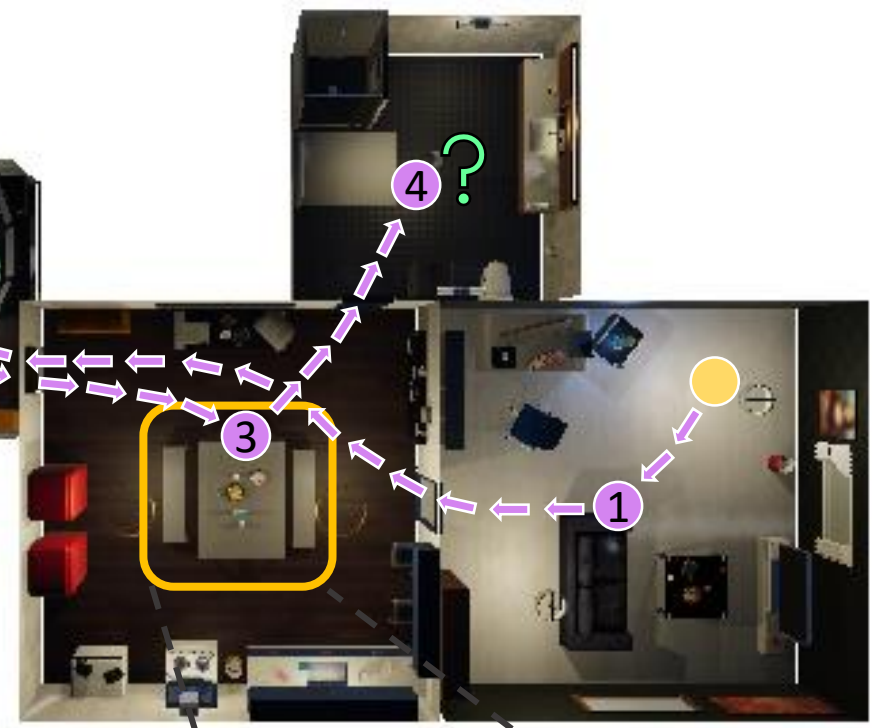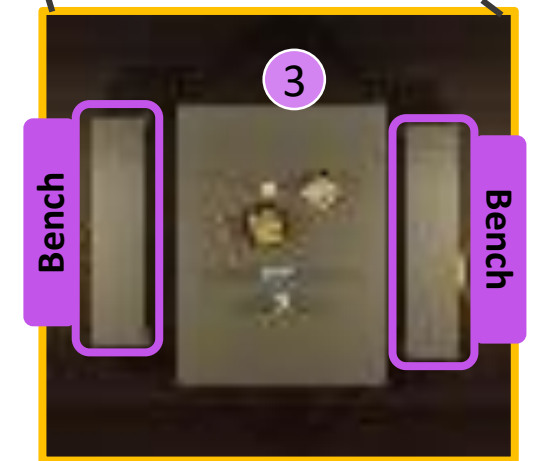

Both benches are obscured by the table.

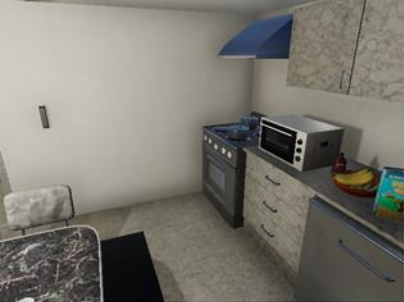

Can you get the box on the wall shelf?

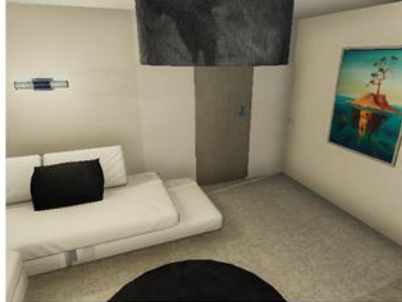

1: Walk to the livingroom

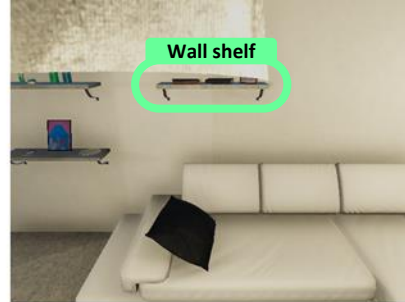

2: Walk to the wall shelf (1)

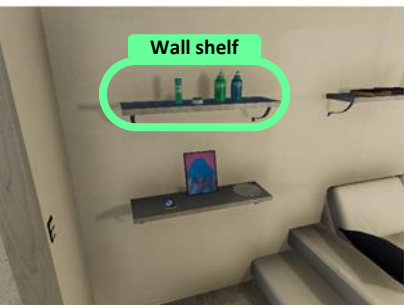

3: Walk to the wall shelf (2)

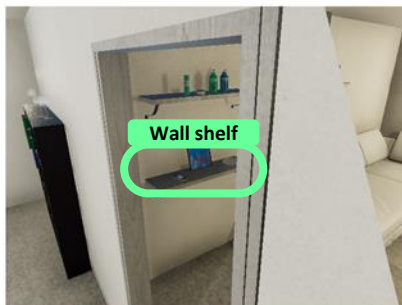

4: Walk to the wall shelf (3)

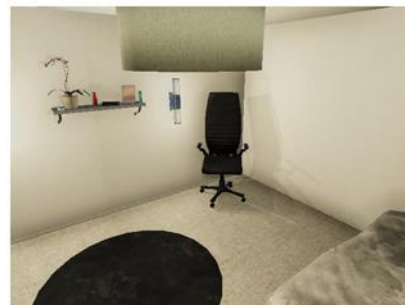

5: Walk to the bedroom

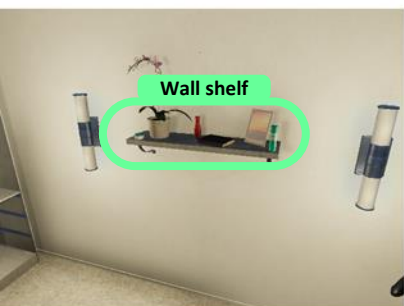

6: Walk to the wall shelf (4)

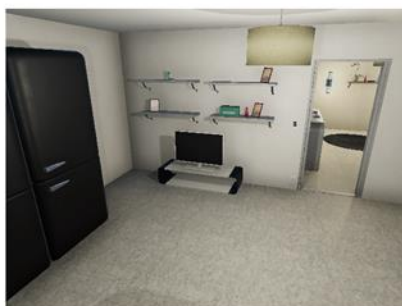

7: Walk to the kitchen

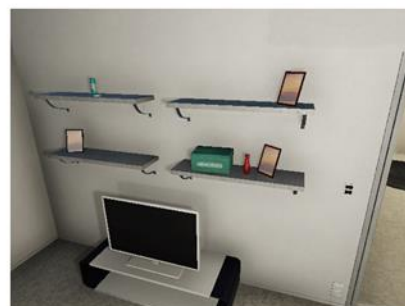

8: Walk to the box

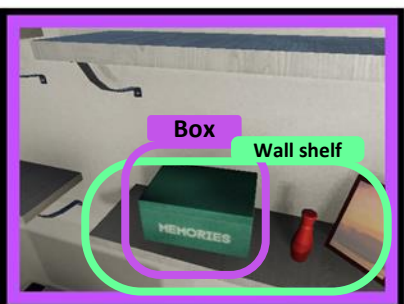

Detected object

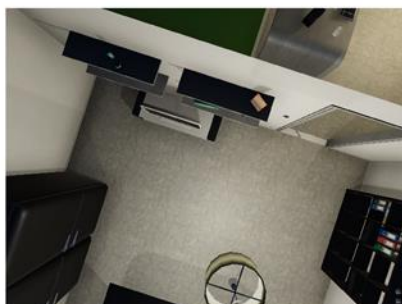

Final state

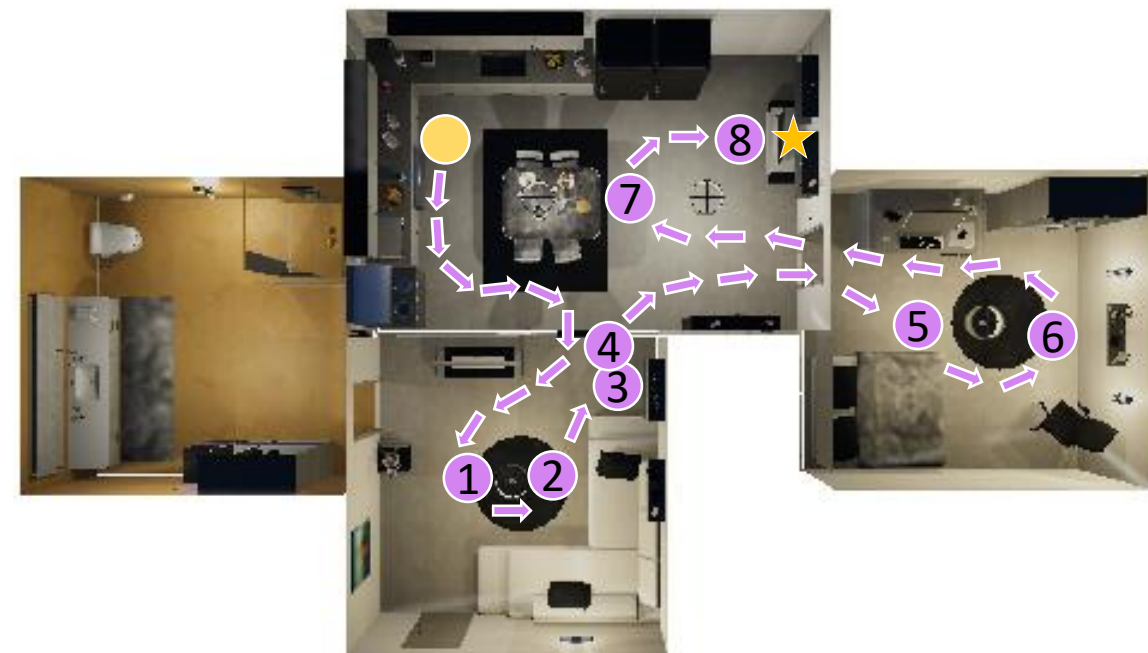

## Navi + Relation

Task: Can you get the **box** on the **wall shelf**?

- 1: Walk to the livingroom
- 2: Walk to the **wall shelf** (1)
- 3: Walk to the **wall shelf** (2)
- 4: Walk to the **wall shelf** (3)
- 5: Walk to the bedroom
- 6: Walk to the **wall shelf** (4)
- 7: Walk to the kitchen
- 8: Walk to the **box**



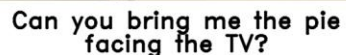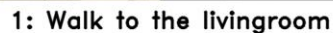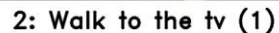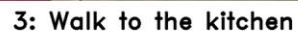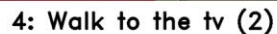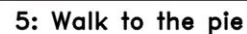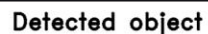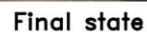

## Navi + Relation

**Task: Can you bring me the pie facing the TV?**

- 1: Walk to the livingroom
- 2: Walk to the tv (1)
- 3: Walk to the kitchen
- 4: Walk to the tv (2)
- 5: Walk to the pie

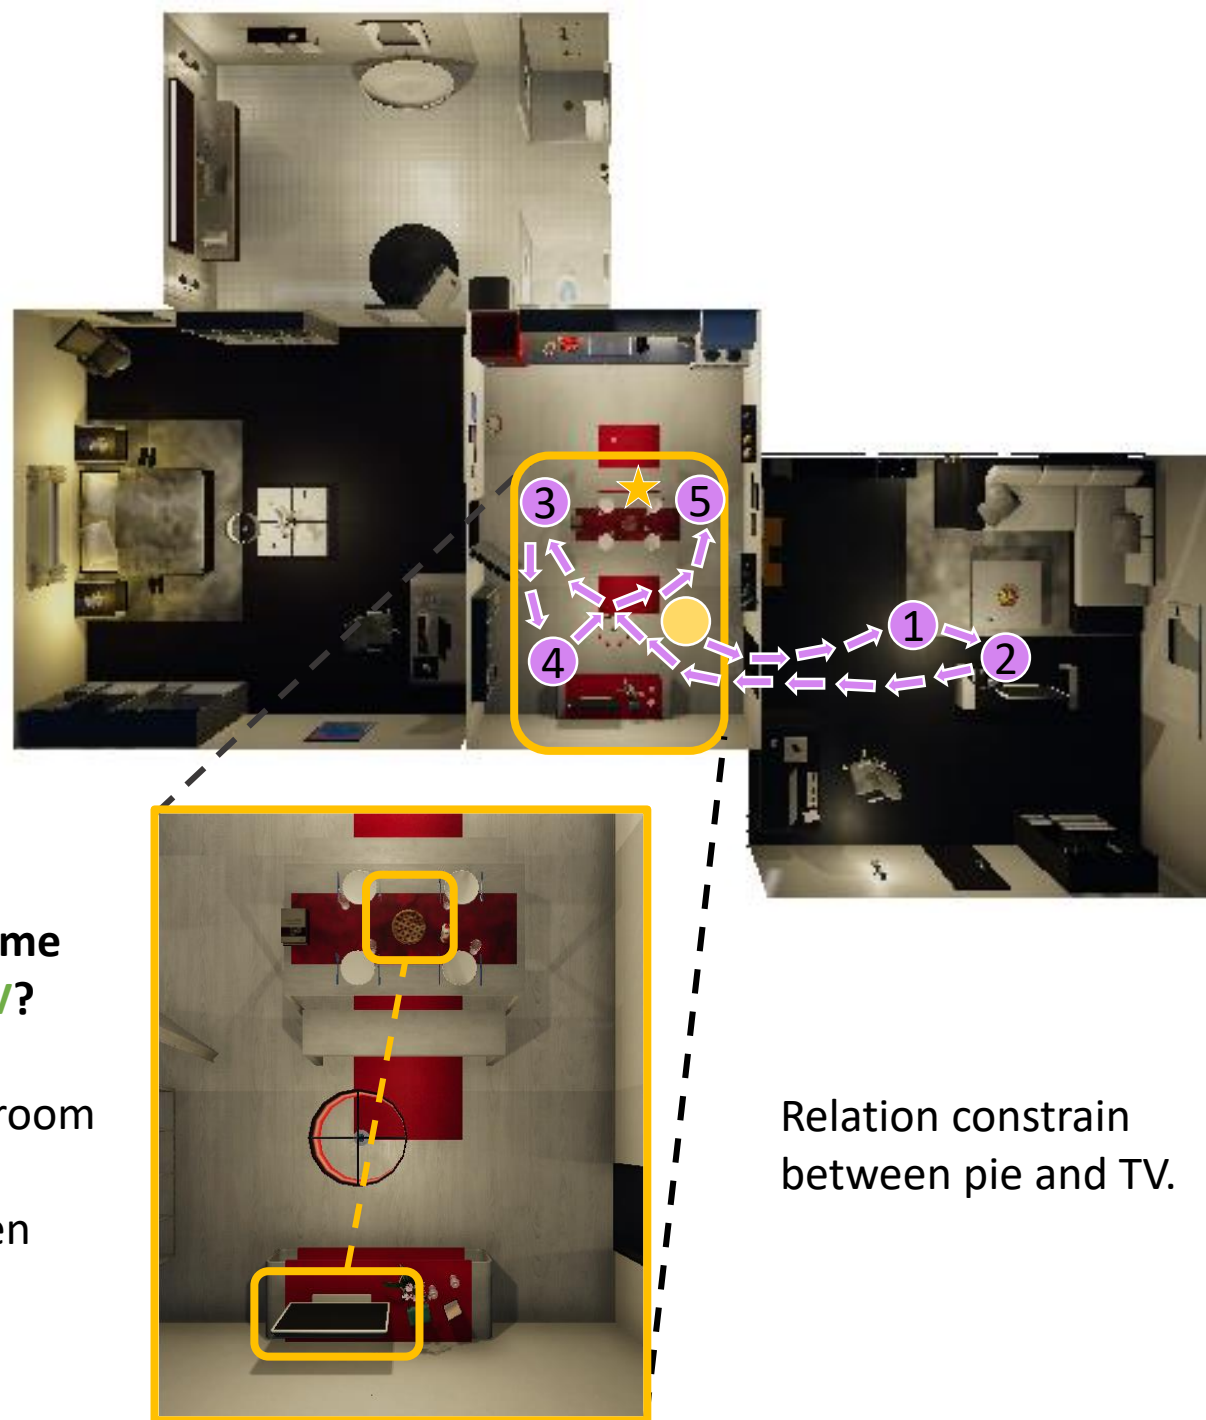

Relation constrain  
between pie and TV.

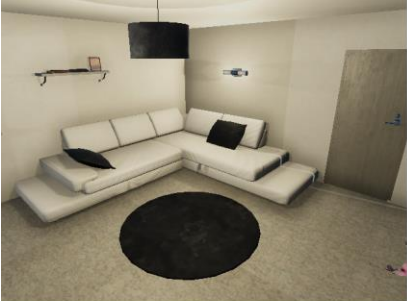

Can you locate the bookshelf facing the TV?

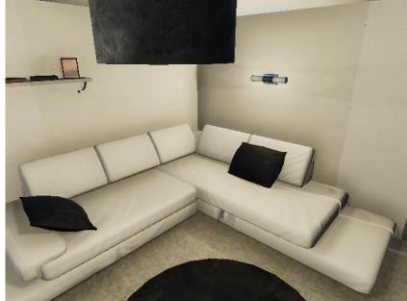

1: Walk to the livingroom

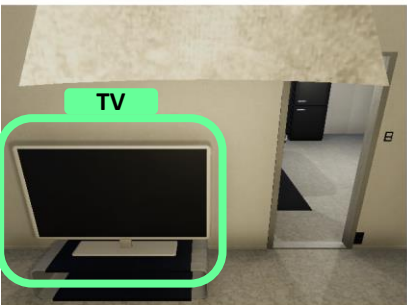

2: Walk to the tv (1)

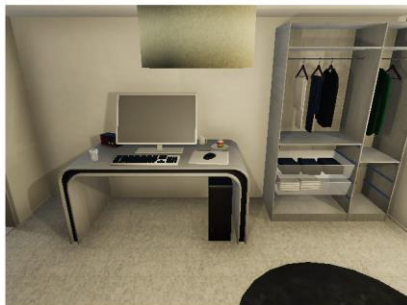

3: Walk to the bedroom

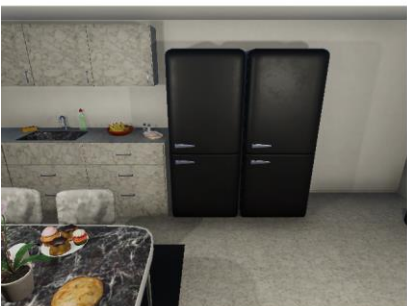

4: Walk to the kitchen

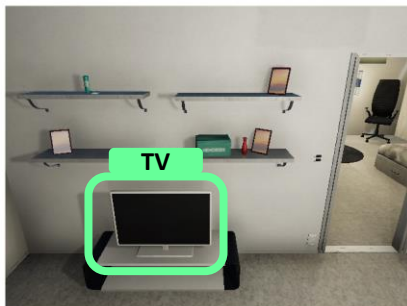

5: Walk to the tv (2)

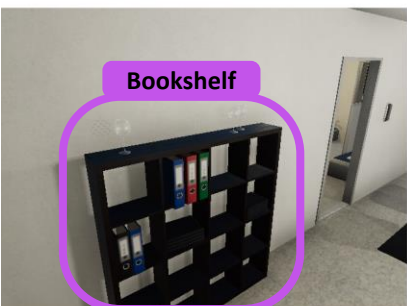

6: Walk to the bookshelf

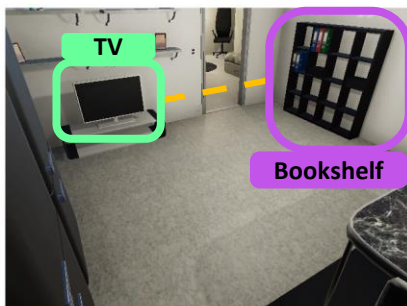

Final state

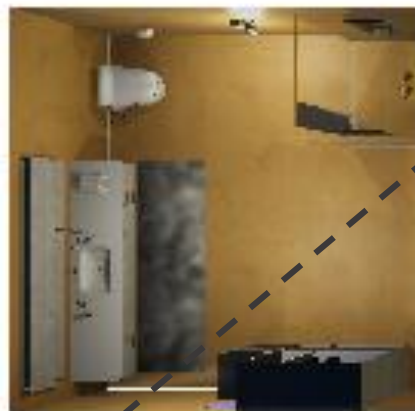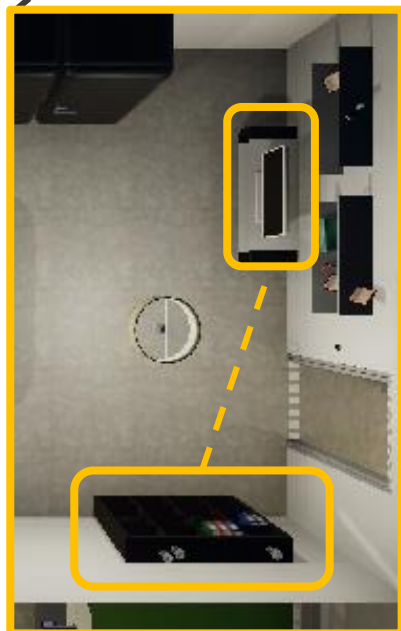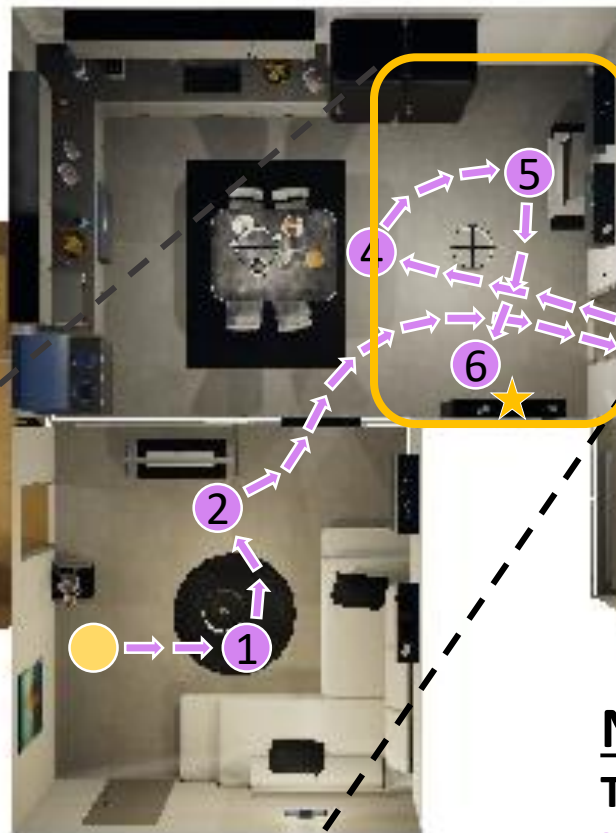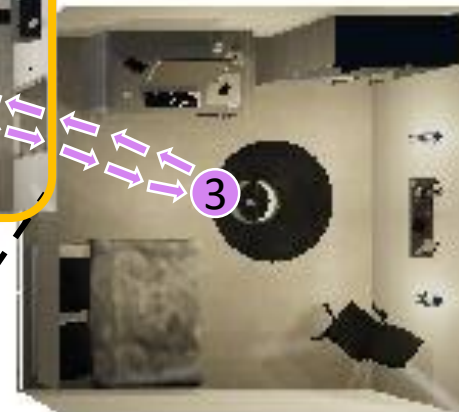

## Navi + Relation

Task: Can you locate the bookshelf facing the TV?

- 1: Walk to the livingroom
- 2: Walk to the tv (1)
- 3: Walk to the bedroom
- 4: Walk to the kitchen
- 5: Walk to the tv (2)
- 6: Walk to the bookshelf

Relation constrain  
between bookshelf  
and TV.



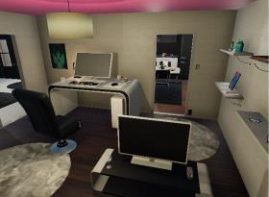

Can you bring me the deodorant close to the toothpaste?

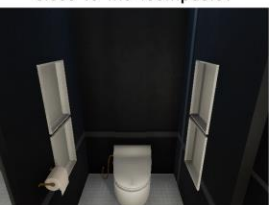

3: Walk to the toilet

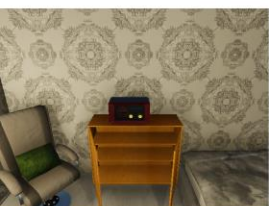

6: Open the cabinet

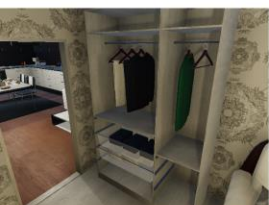

9: Walk to the closet drawer (2)

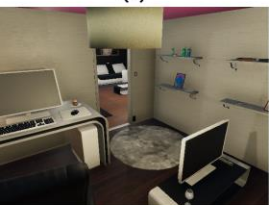

12: Walk to the livingroom

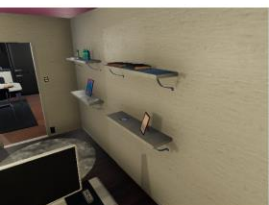

15: Walk to the wall shelf (3)

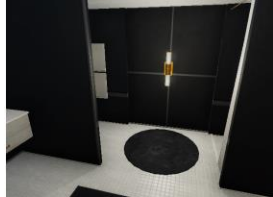

1: Walk to the bathroom

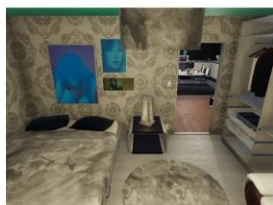

4: Walk to the bedroom

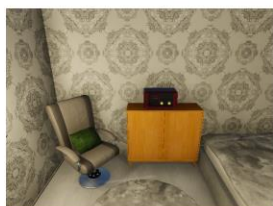

7: Close the cabinet

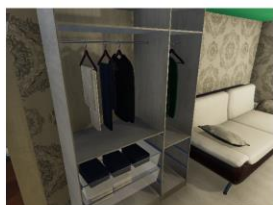

10: Walk to the closet

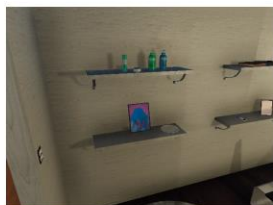

13: Walk to the wall shelf (1)

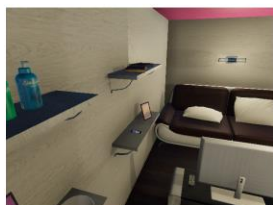

16: Walk to the wall shelf (4)

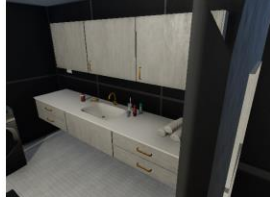

5: Walk to the cabinet (1)

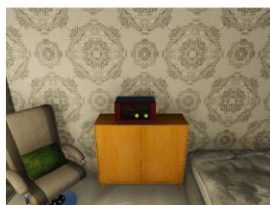

8: Walk to the closet drawer (1)

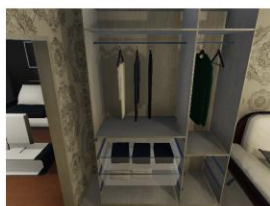

11: Walk to the kitchen

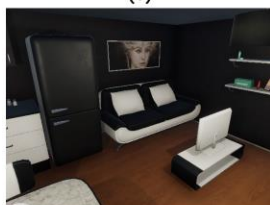

14: Walk to the wall shelf (2)

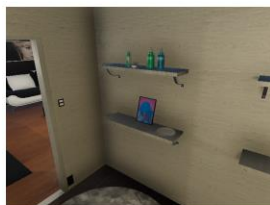

Final state

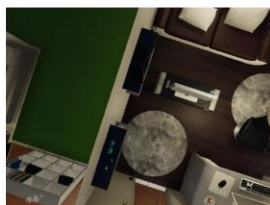

Final state

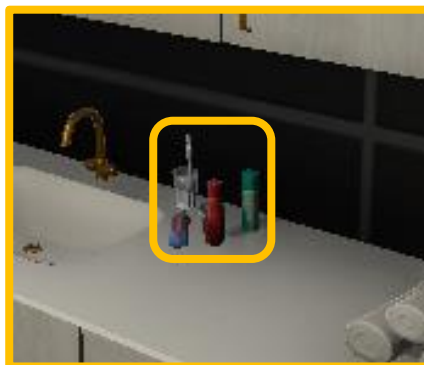

The objects in the counter obstruct the visibility and relations between them.

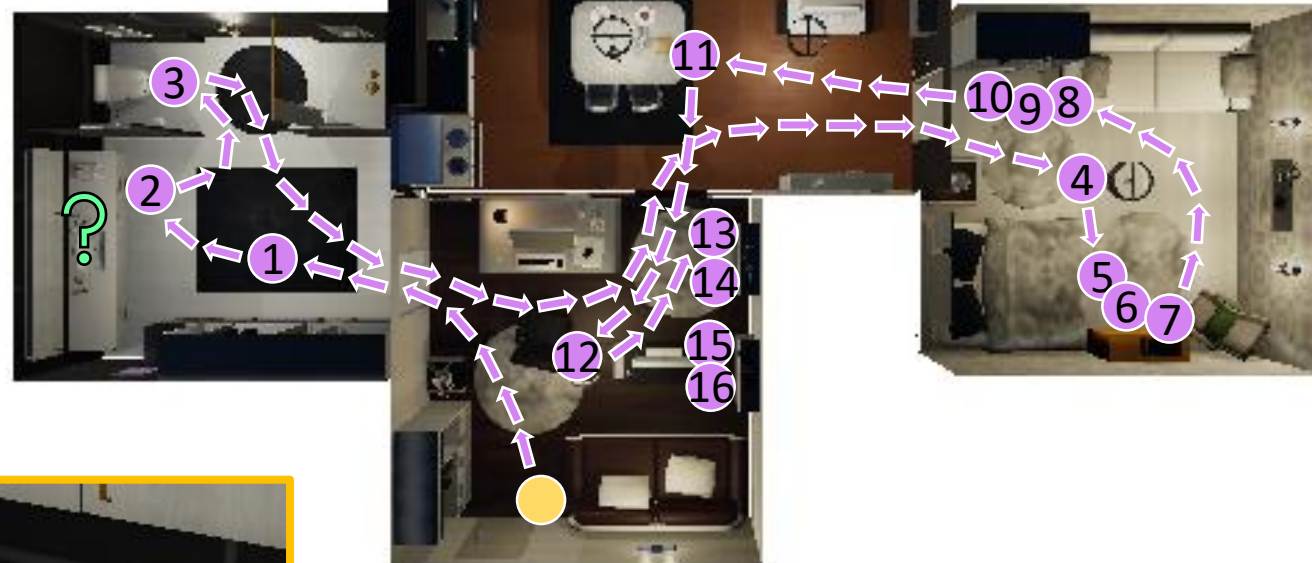

## Navi + Relation

Task: Can you bring me the **deodorant** close to the **toothpaste**?

- 1: Walk to the bathroom
- 2: Walk to the **deodorant**
- 3: Walk to the toilet
- 4: Walk to the bedroom
- 5: Walk to the cabinet (1)

- 6: Open the cabinet
- 7: Close the cabinet
- 8: Walk to the closet drawer (1)
- 9: Walk to the closet drawer (2)
- 10: Walk to the closet
- 11: Walk to the kitchen
- 12: Walk to the livingroom
- 13: Walk to the wall shelf (1)
- 14: Walk to the wall shelf (2)
- 15: Walk to the wall shelf (3)
- 16: Walk to the wall shelf (4)



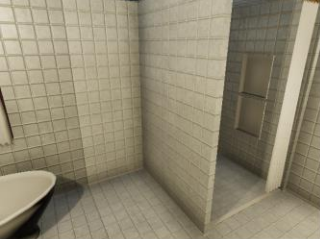

Can you locate the condiment shaker inside the kitchen?

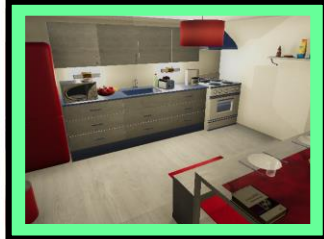

1: Walk to the kitchen

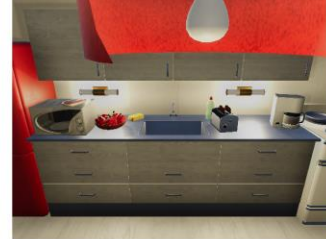

2: Walk to the kitchen counter (1)

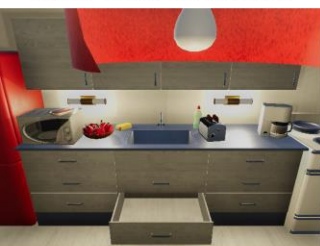

3: Open the kitchen counter

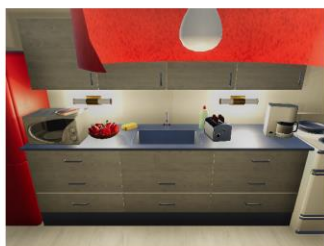

4: Close the kitchen counter

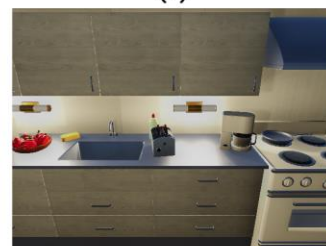

5: Walk to the kitchen cabinet (1)

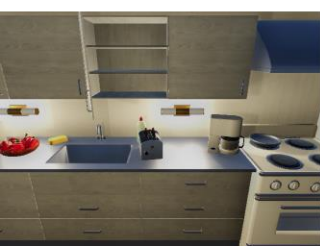

6: Open the kitchen cabinet

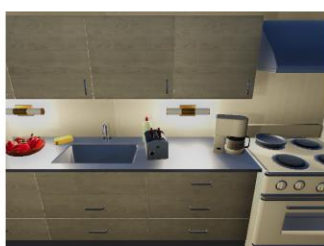

7: Close the kitchen cabinet

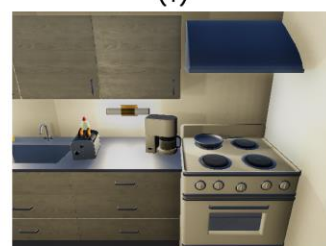

8: Walk to the kitchen cabinet (2)

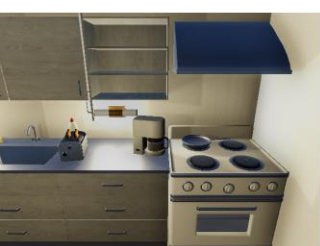

9: Open the kitchen cabinet

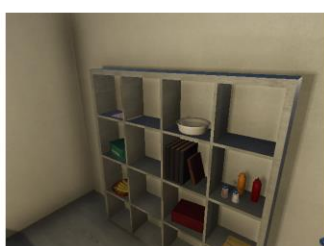

10: Walk to the bookshelf

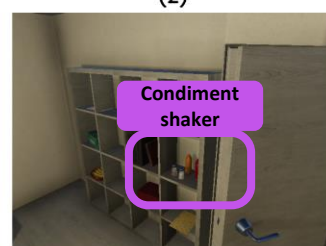

11: Walk to the condimentshaker

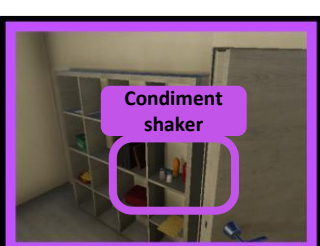

Detected object

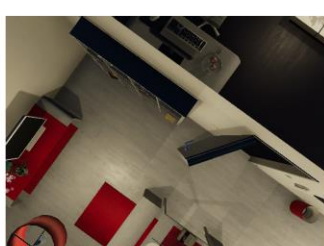

Final state

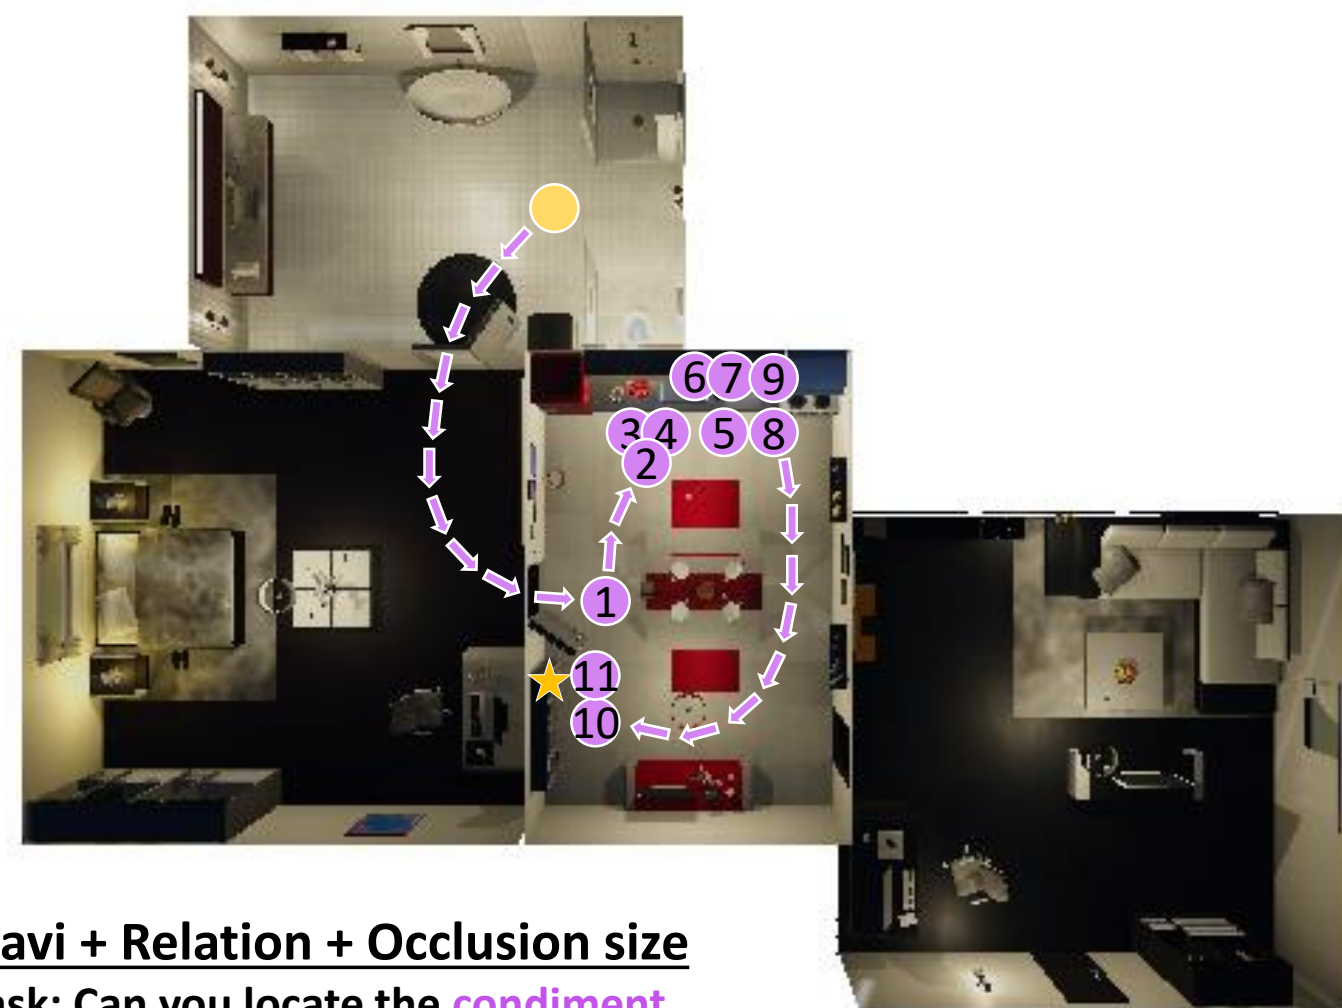

## Navi + Relation + Occlusion size

Task: Can you locate the **condiment shaker** inside the **kitchen**?

- 1: Walk to the **kitchen**
- 2: Walk to the kitchen counter (1)
- 3: Open the kitchen counter
- 4: Close the kitchen counter
- 5: Walk to the kitchen cabinet (1)

- 6: Open the kitchen cabinet
- 7: Close the kitchen cabinet
- 8: Walk to the kitchen cabinet (2)
- 9: Open the kitchen cabinet
- 10: Walk to the bookshelf
- 11: Walk to the **condiment shaker**



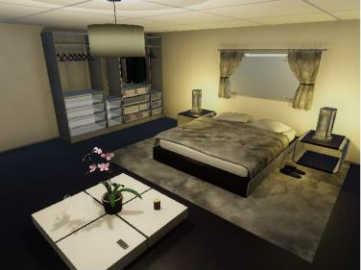

Can you bring me the toothbrush from inside the bathroom?

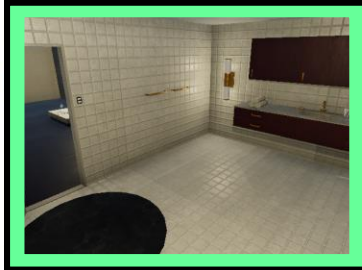

1: Walk to the bathroom

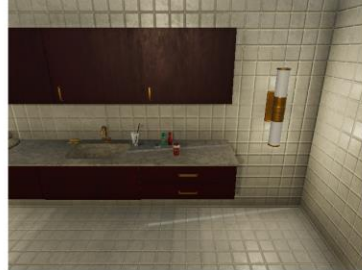

2: Walk to the bathroom counter (1)

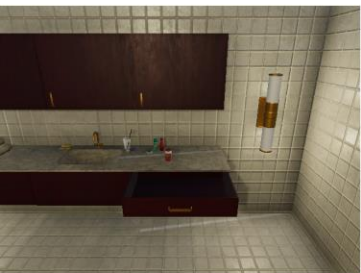

3: Open the bathroom counter

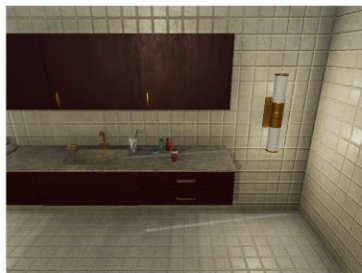

4: Close the bathroom counter

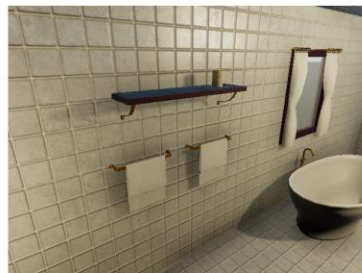

5: Walk to the wall shelf (1)

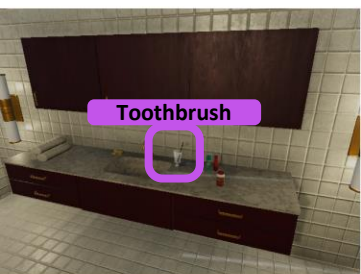

6: Walk to the toothbrush

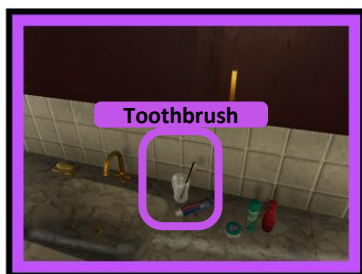

Detected object

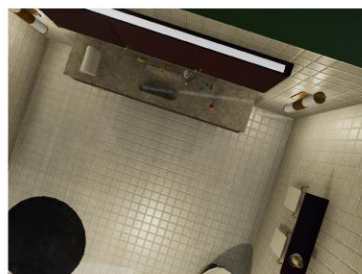

Final state

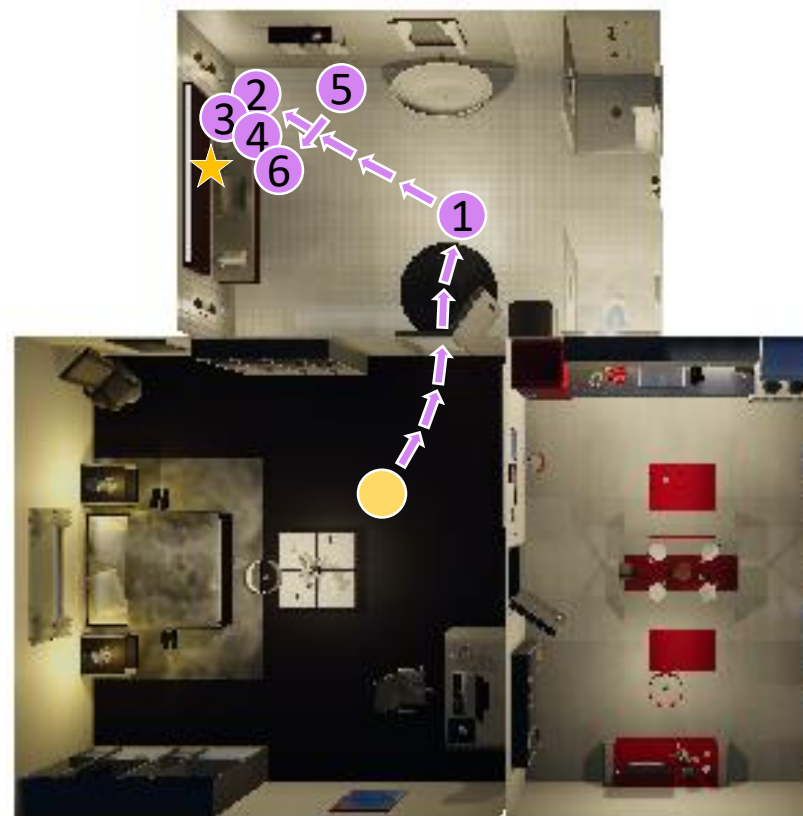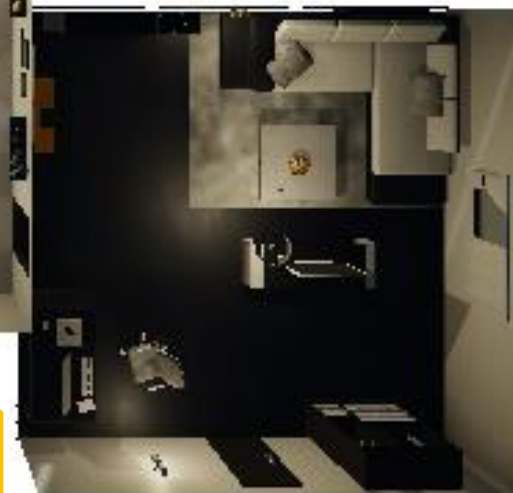

## Navi + Relation + Occlusion size

Task: Can you bring me the **toothbrush** from inside the **bathroom**

1: Walk to the **bathroom**  
2: Walk to the bathroom counter (1)

3: Open the bathroom counter  
4: Close the bathroom counter  
5: Walk to the wall shelf (1)  
6: Walk to the **toothbrush**

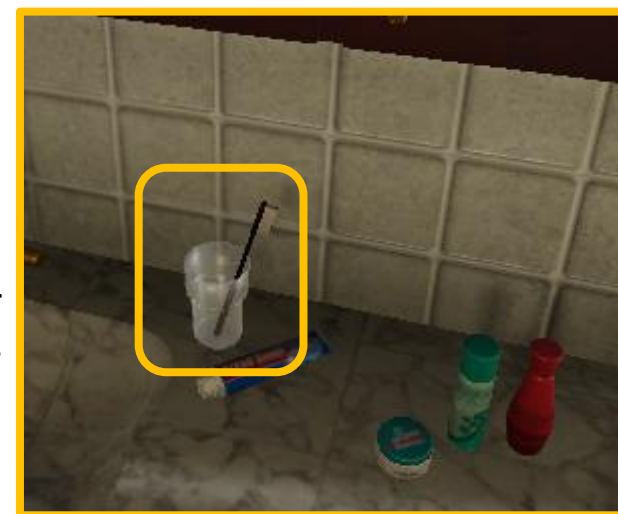

Toothbrush is semi-obstructed by the glass.



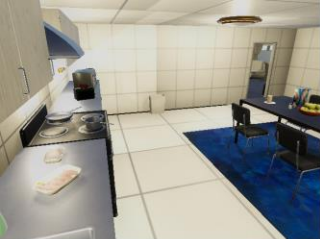

Find the mug and put it inside the fridge.

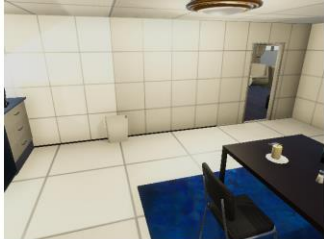

1: Walk to the kitchen

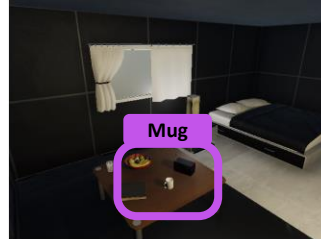

2: Walk to the mug

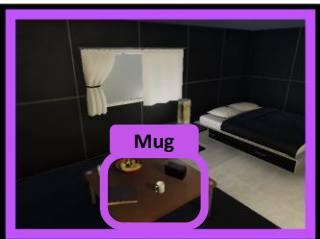

3: Grab the mug

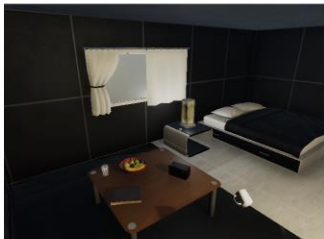

3: Grab the mug

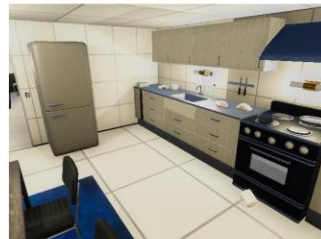

4: Walk to the kitchen

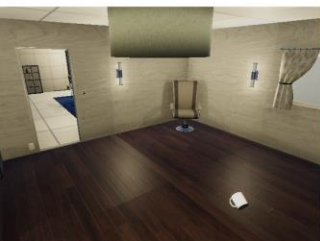

5: Walk to the livingroom

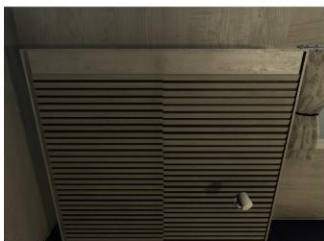

6: Walk to the closet

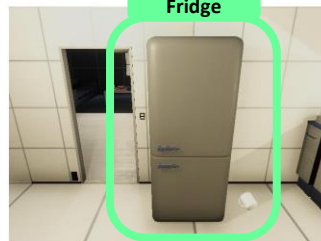

7: Walk to the fridge

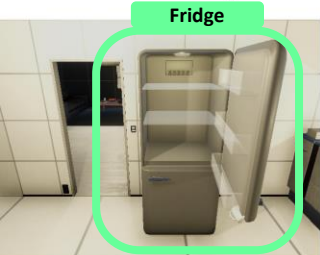

8: Open the fridge

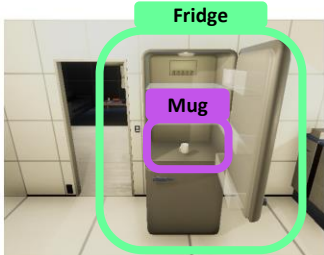

9: Put the mug inside the fridge

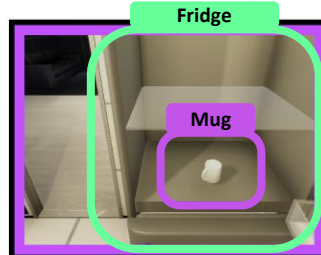

9: Put the mug inside the fridge

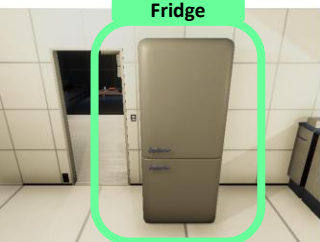

10: Close the fridge

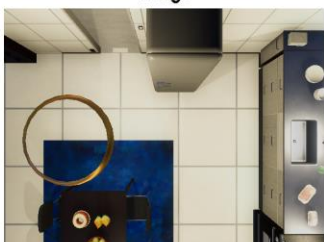

Final state

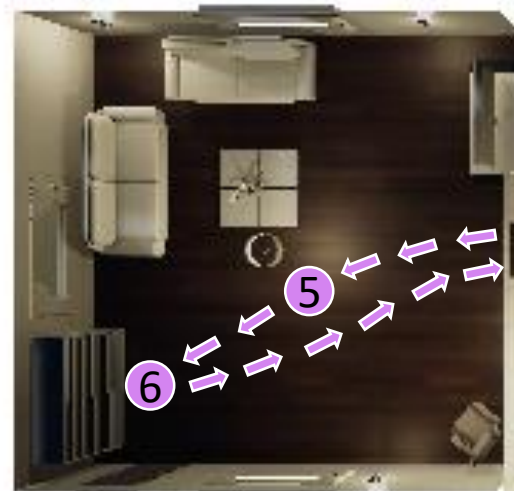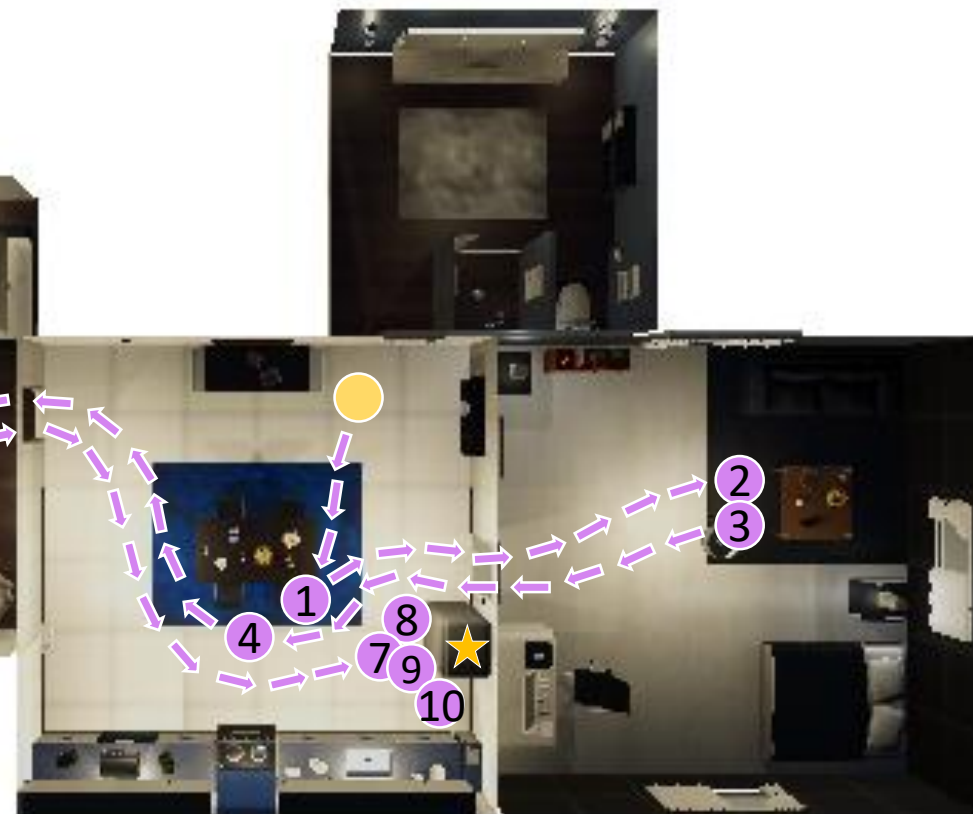

## Navi & Mani + Occlusion size

Task: Find the **mug** and put it inside the **fridge**.

- 1: Walk to the kitchen
- 2: Walk to the **mug**
- 3: Grab the **mug**
- 4: Walk to the kitchen
- 5: Walk to the livingroom

- 6: Walk to the closet
- 7: Walk to the **fridge**
- 8: Open the **fridge**
- 9: Put the **mug** inside the **fridge**
- 10: Close the **fridge**

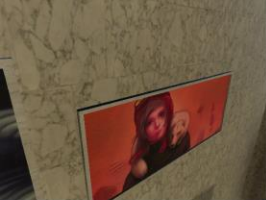

Can you get a cutlery fork from inside the kitchen?

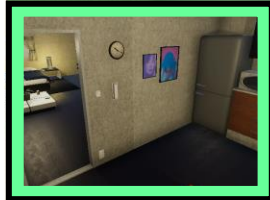

1: Walk to the kitchen

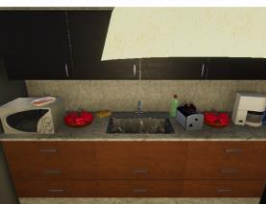

2: Walk to the kitchen cabinet (1)

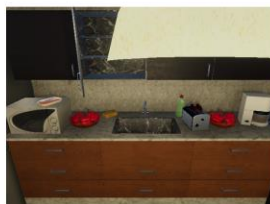

3: Open the kitchen cabinet

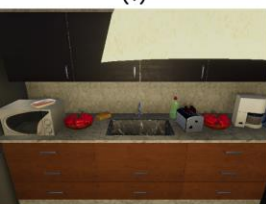

4: Close the kitchen cabinet

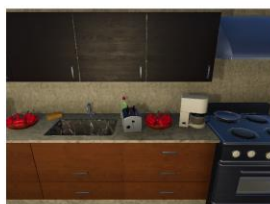

5: Walk to the kitchen cabinet (2)

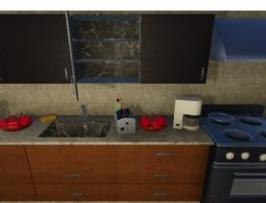

6: Open the kitchen cabinet

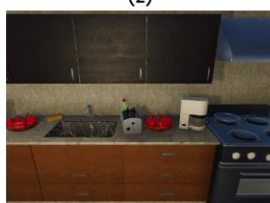

7: Close the kitchen cabinet

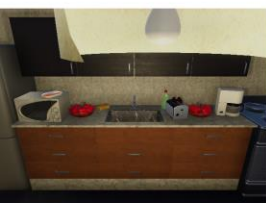

8: Walk to the kitchen counter (1)

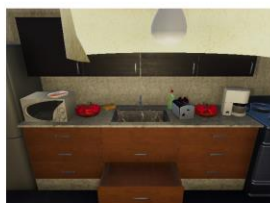

9: Open the kitchen counter

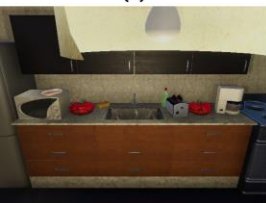

10: Close the kitchen counter

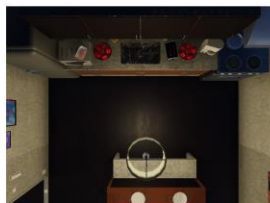

Final state

## Navi + Relation + Occlusion size

Task: Can you get a **cutlery fork** from inside the **kitchen**?

- 1: Walk to the **kitchen**
- 2: Walk to the kitchen cabinet (1)
- 3: Open the kitchen cabinet
- 4: Close the kitchen cabinet

- 5: Walk to the kitchen cabinet (2)
- 6: Open the kitchen cabinet
- 7: Close the kitchen cabinet
- 8: Walk to the kitchen counter (1)
- 9: Open the kitchen counter
- 10: Close the kitchen counter
- 11: ....

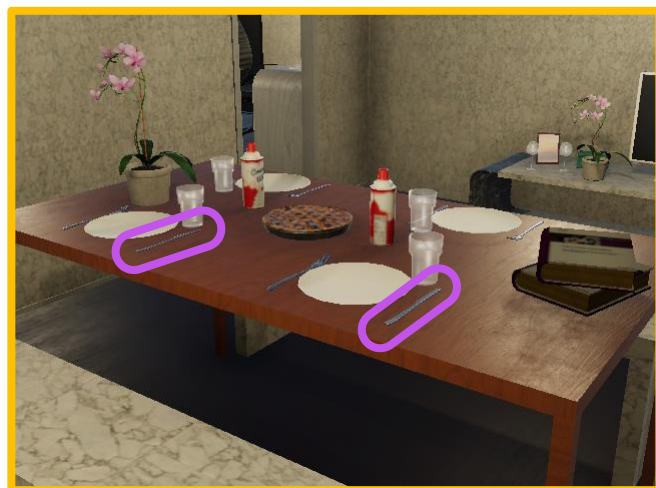

The LLM decides not to explore larger objects like the kitchen table, where the goal object is located.

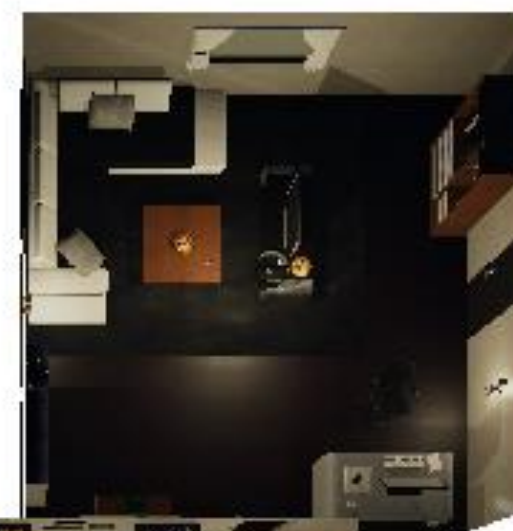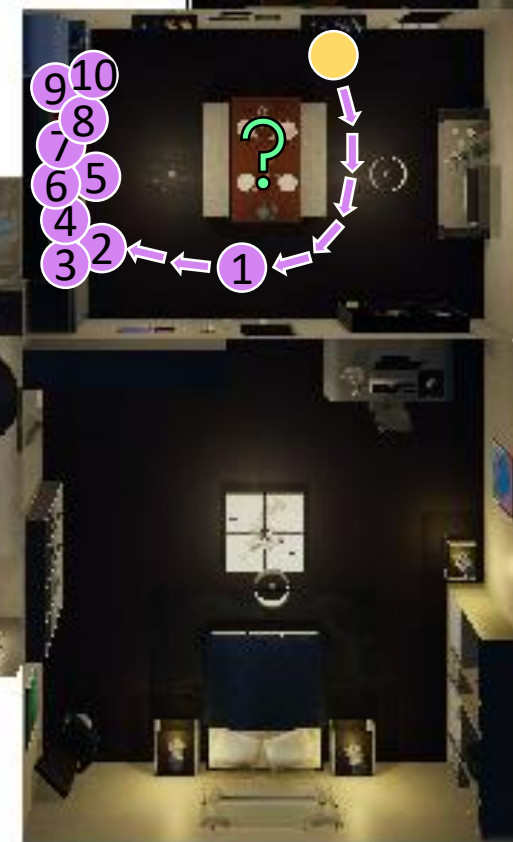



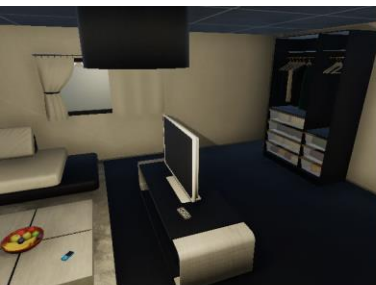

Can you find the candle inside the bedroom?

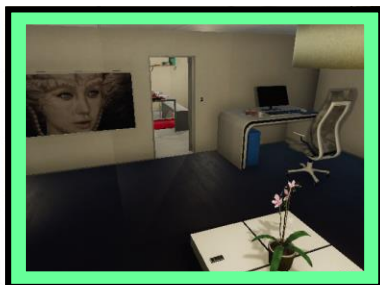

1: Walk to the bedroom

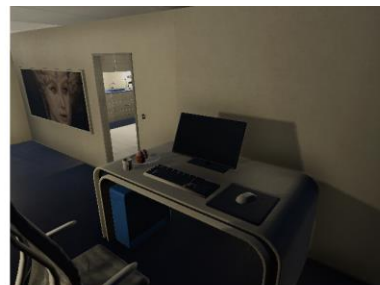

2: Walk to the desk

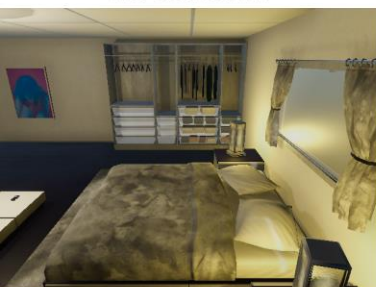

3: Walk to the bed

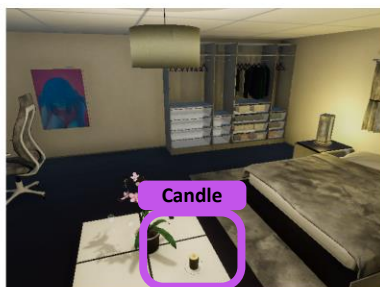

4: Walk to the candle

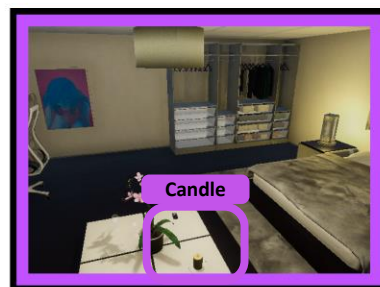

Detected object

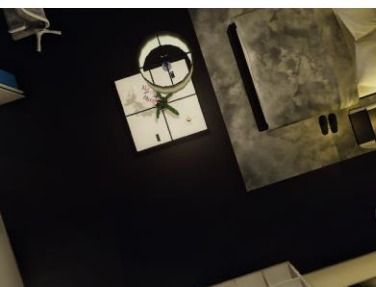

Final state

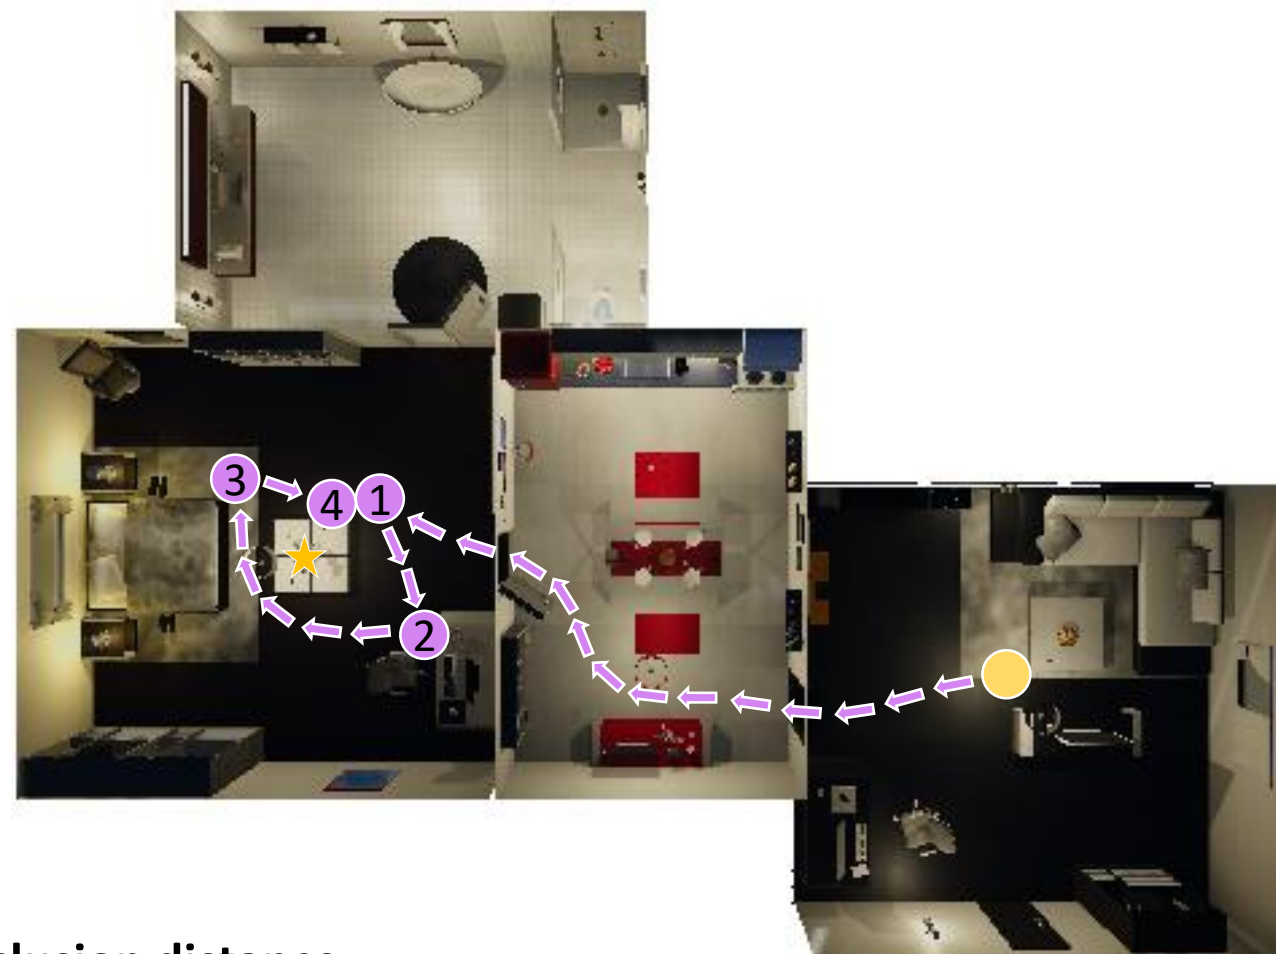

## Navi + Relation + Occlusion distance

Task: Can you find the **candle** inside the **bedroom**?

1: Walk to the **bedroom**

2: Walk to the desk

3: Walk to the bed

4: Walk to the **candle**

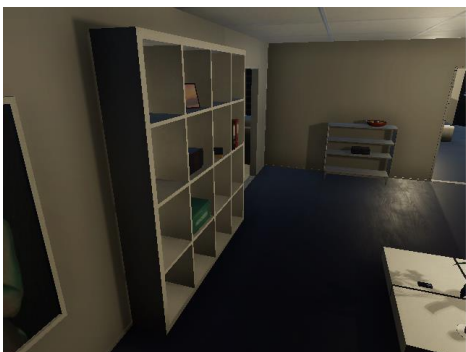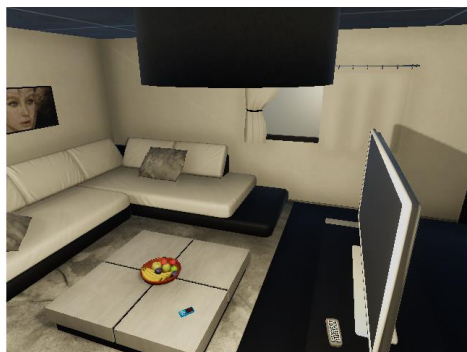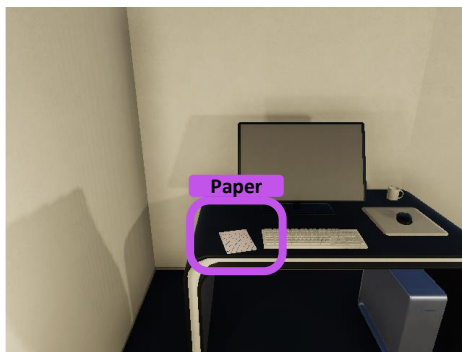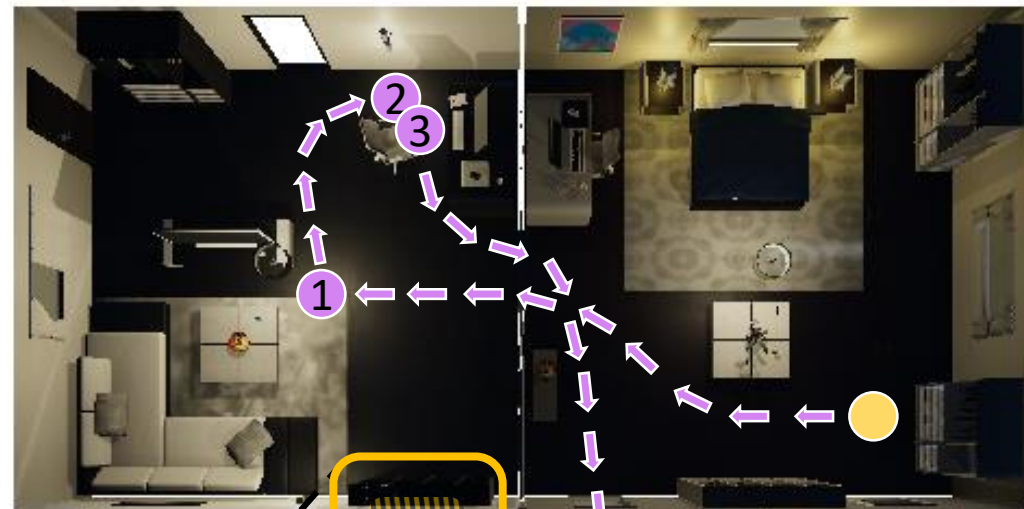

Your task is to get paper inside livingroom and move it to toilet inside bathroom.

1: Walk to the livingroom

2: Walk to the paper

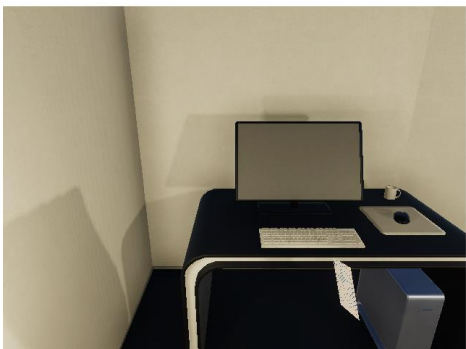

3: Grab the paper

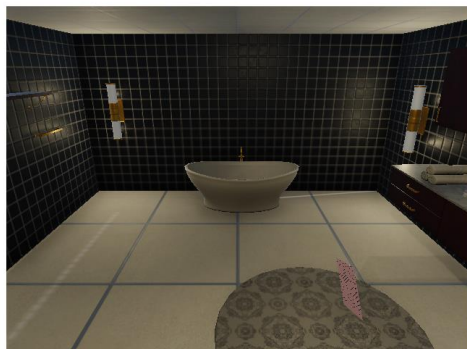

4: Walk to the bathroom

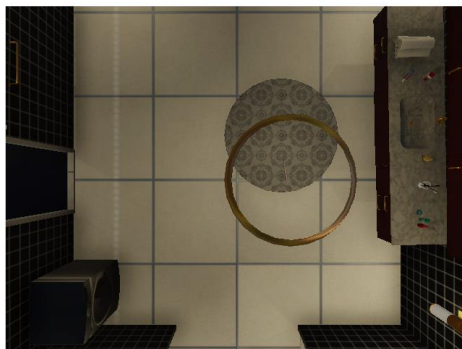

Final state

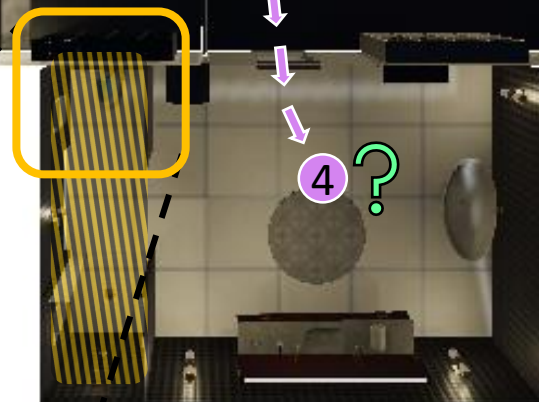

Unexplored area

The toilet was blocked by a wall and the LLM decided not to explore near this area.

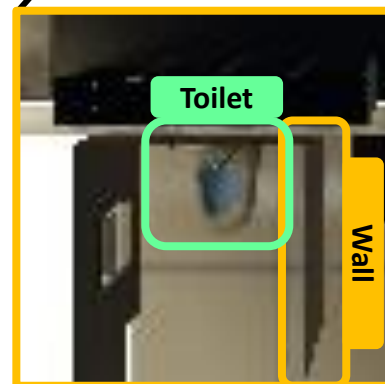

## Navi & Mani + Relation + Occlusion distance

Your task is to get **paper** inside livingroom and move it to **toilet** inside bathroom.

1: Walk to the livingroom

2: Walk to the **paper**

3: Grab the **paper**

4: Walk to the bathroom



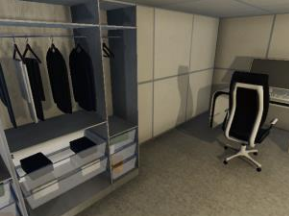

Find a wineglass and a mug, then put them on the kitchen cabinet

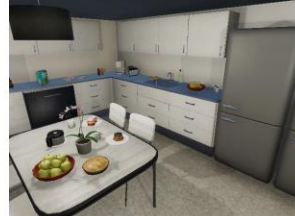

1: Walk to the kitchen

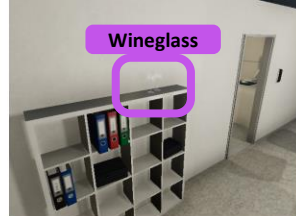

2: Walk to the wineglass

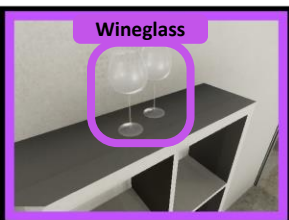

3: Grab the wineglass

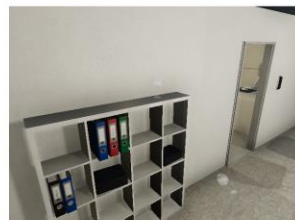

3: Grab the wineglass

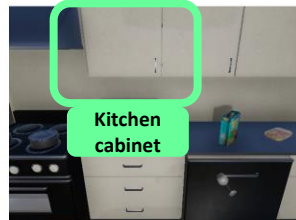

4: Walk to the kitchen cabinet (1)

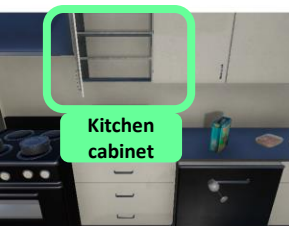

5: Open the kitchen cabinet

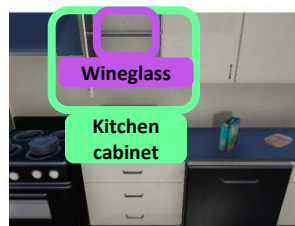

6: Put the wineglass inside the kitchen cabinet

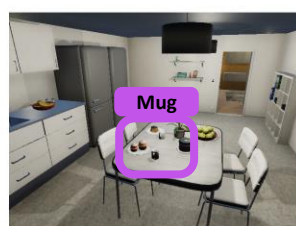

7: Walk to the mug

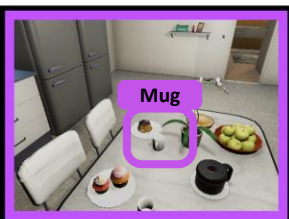

8: Grab the mug

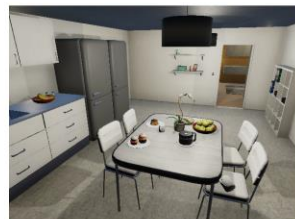

8: Grab the mug

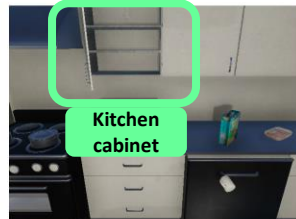

9: Walk to the kitchen cabinet (1)

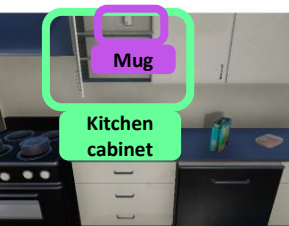

10: Put the mug inside the kitchen cabinet

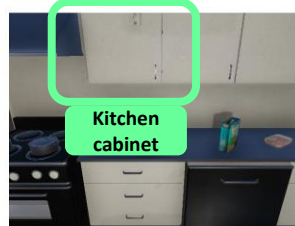

11: Close the kitchen cabinet

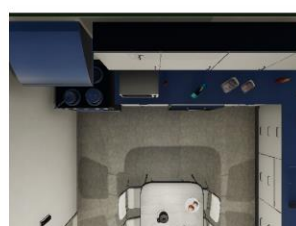

Final state

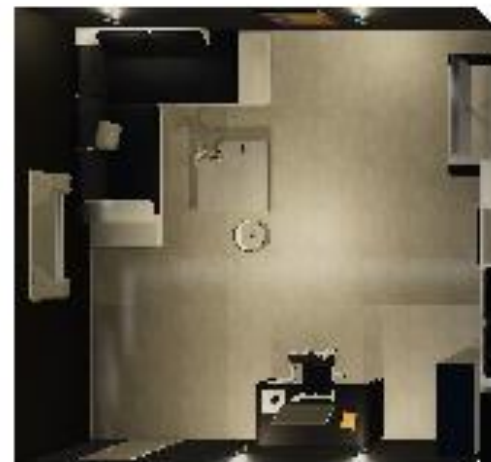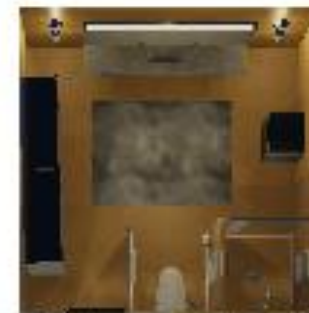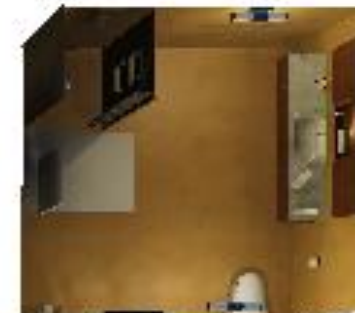

## Navi & Mani w/ Multiple objects

Task: Find a **wineglass** and a **mug**, then put them on the **kitchen cabinet**

1: Walk to the kitchen

2: Walk to the **wineglass**

3: Grab the **wineglass**

4: Walk to the **kitchen cabinet** (1)

5: Open the **kitchen cabinet**

6: Put the wineglass inside the **kitchen cabinet**

7: Walk to the **mug**

8: Grab the **mug**

9: Walk to the **kitchen cabinet** (1)

10: Put the mug inside the **kitchen cabinet**

11: Close the **kitchen cabinet**

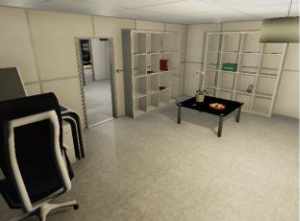

Gather the coffeepot and wineglass and then lay them into then dishwasher.

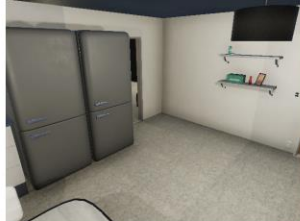

1: Walk to the kitchen

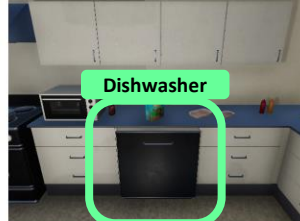

2: Walk to the dishwasher

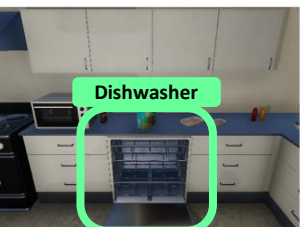

3: Open the dishwasher

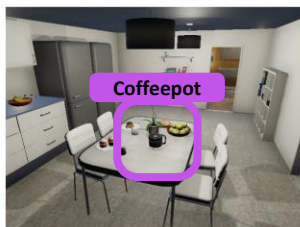

4: Walk to the coffeepot

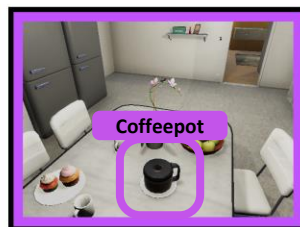

5: Grab the coffeepot

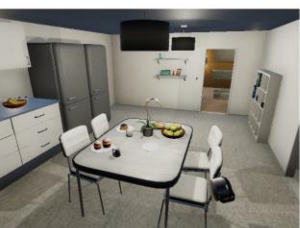

5: Grab the coffeepot

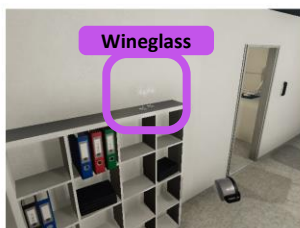

6: Walk to the wineglass

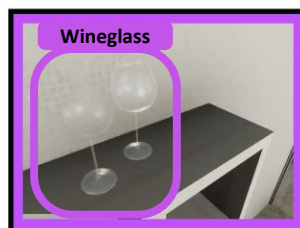

7: Grab the wineglass

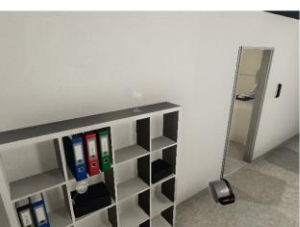

7: Grab the wineglass

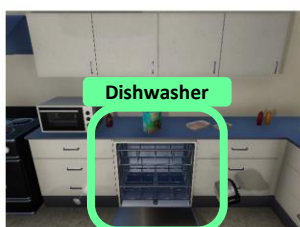

8: Walk to the dishwasher

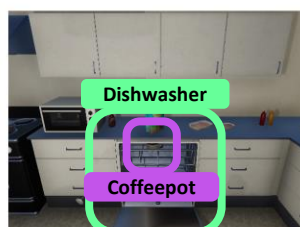

9: Put the coffeepot inside the dishwasher

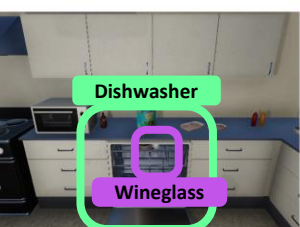

10: Put the wineglass inside the dishwasher

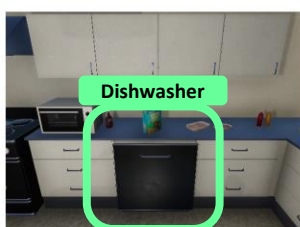

11: Close the dishwasher

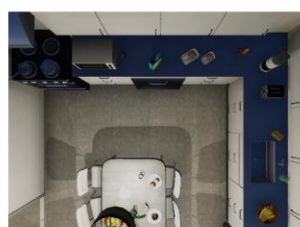

Final state

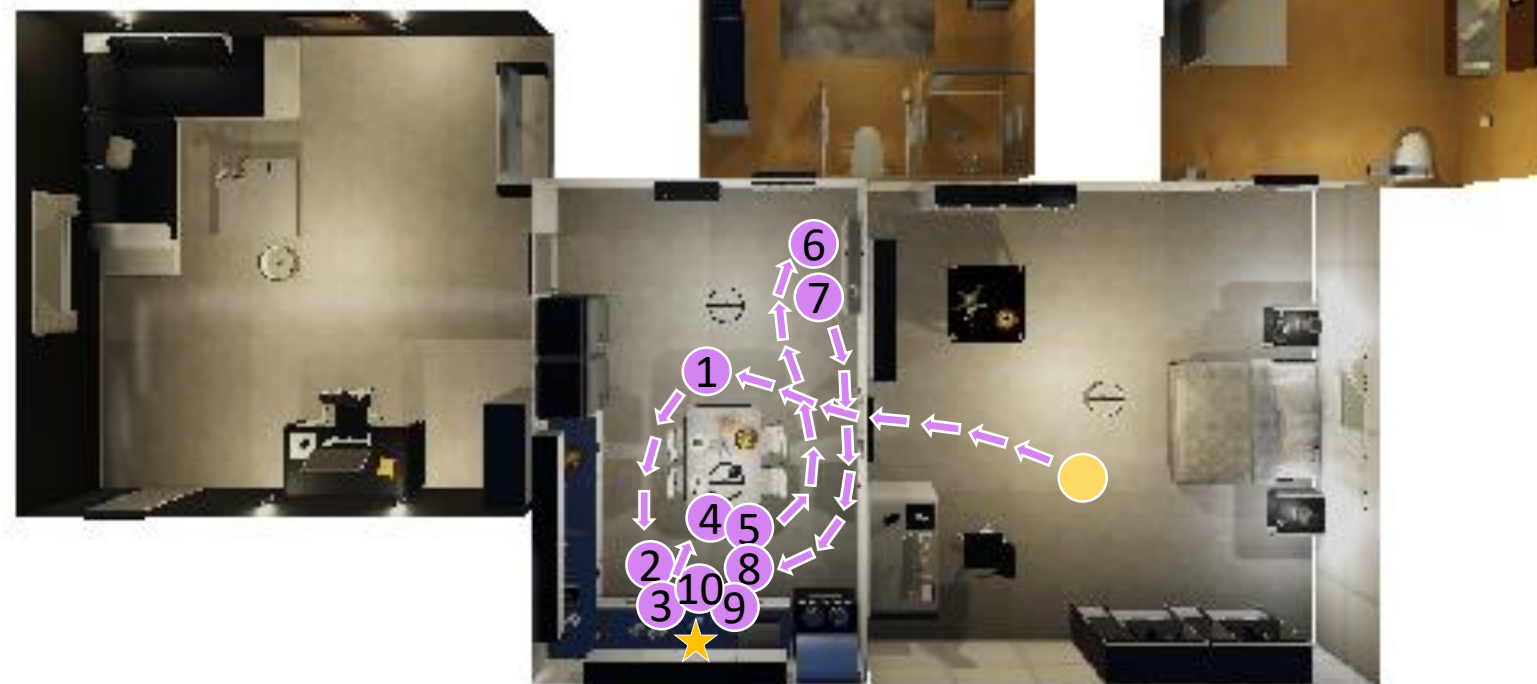

## Navi & Mani w/ Multiple objects

### + Optimal path

Task: Gather the **coffeepot** and **wineglass** and then lay them into the **dishwasher**.

- 1: Walk to the kitchen
- 2: Walk to the **dishwasher**
- 3: Open the **dishwasher**
- 4: Walk to the **coffeepot**

5: Grab the **coffeepot**

6: Walk to the **wineglass**

7: Grab the **wineglass**

8: Walk to the **dishwasher**

9: Put the **coffeepot** inside the **dishwasher**

10: Put the **wineglass** inside the **dishwasher**

11: Close the **dishwasher**
